# Supplementary material for: Training High-Level Schedulers with Execution-Feedback Reinforcement Learning for Long-Horizon GUI Automation
Source: arXiv:2511.22235 source file (2026-03-04)
Supplement: Supplementary file 1 [file case.pdf]

# User Instruction

Organize a business meeting with saltyfunswweets using ZOOM Cloud Meetings, send out the meeting invitations via Tumblr, and set an alarm clock for the meeting time using the Clock app.

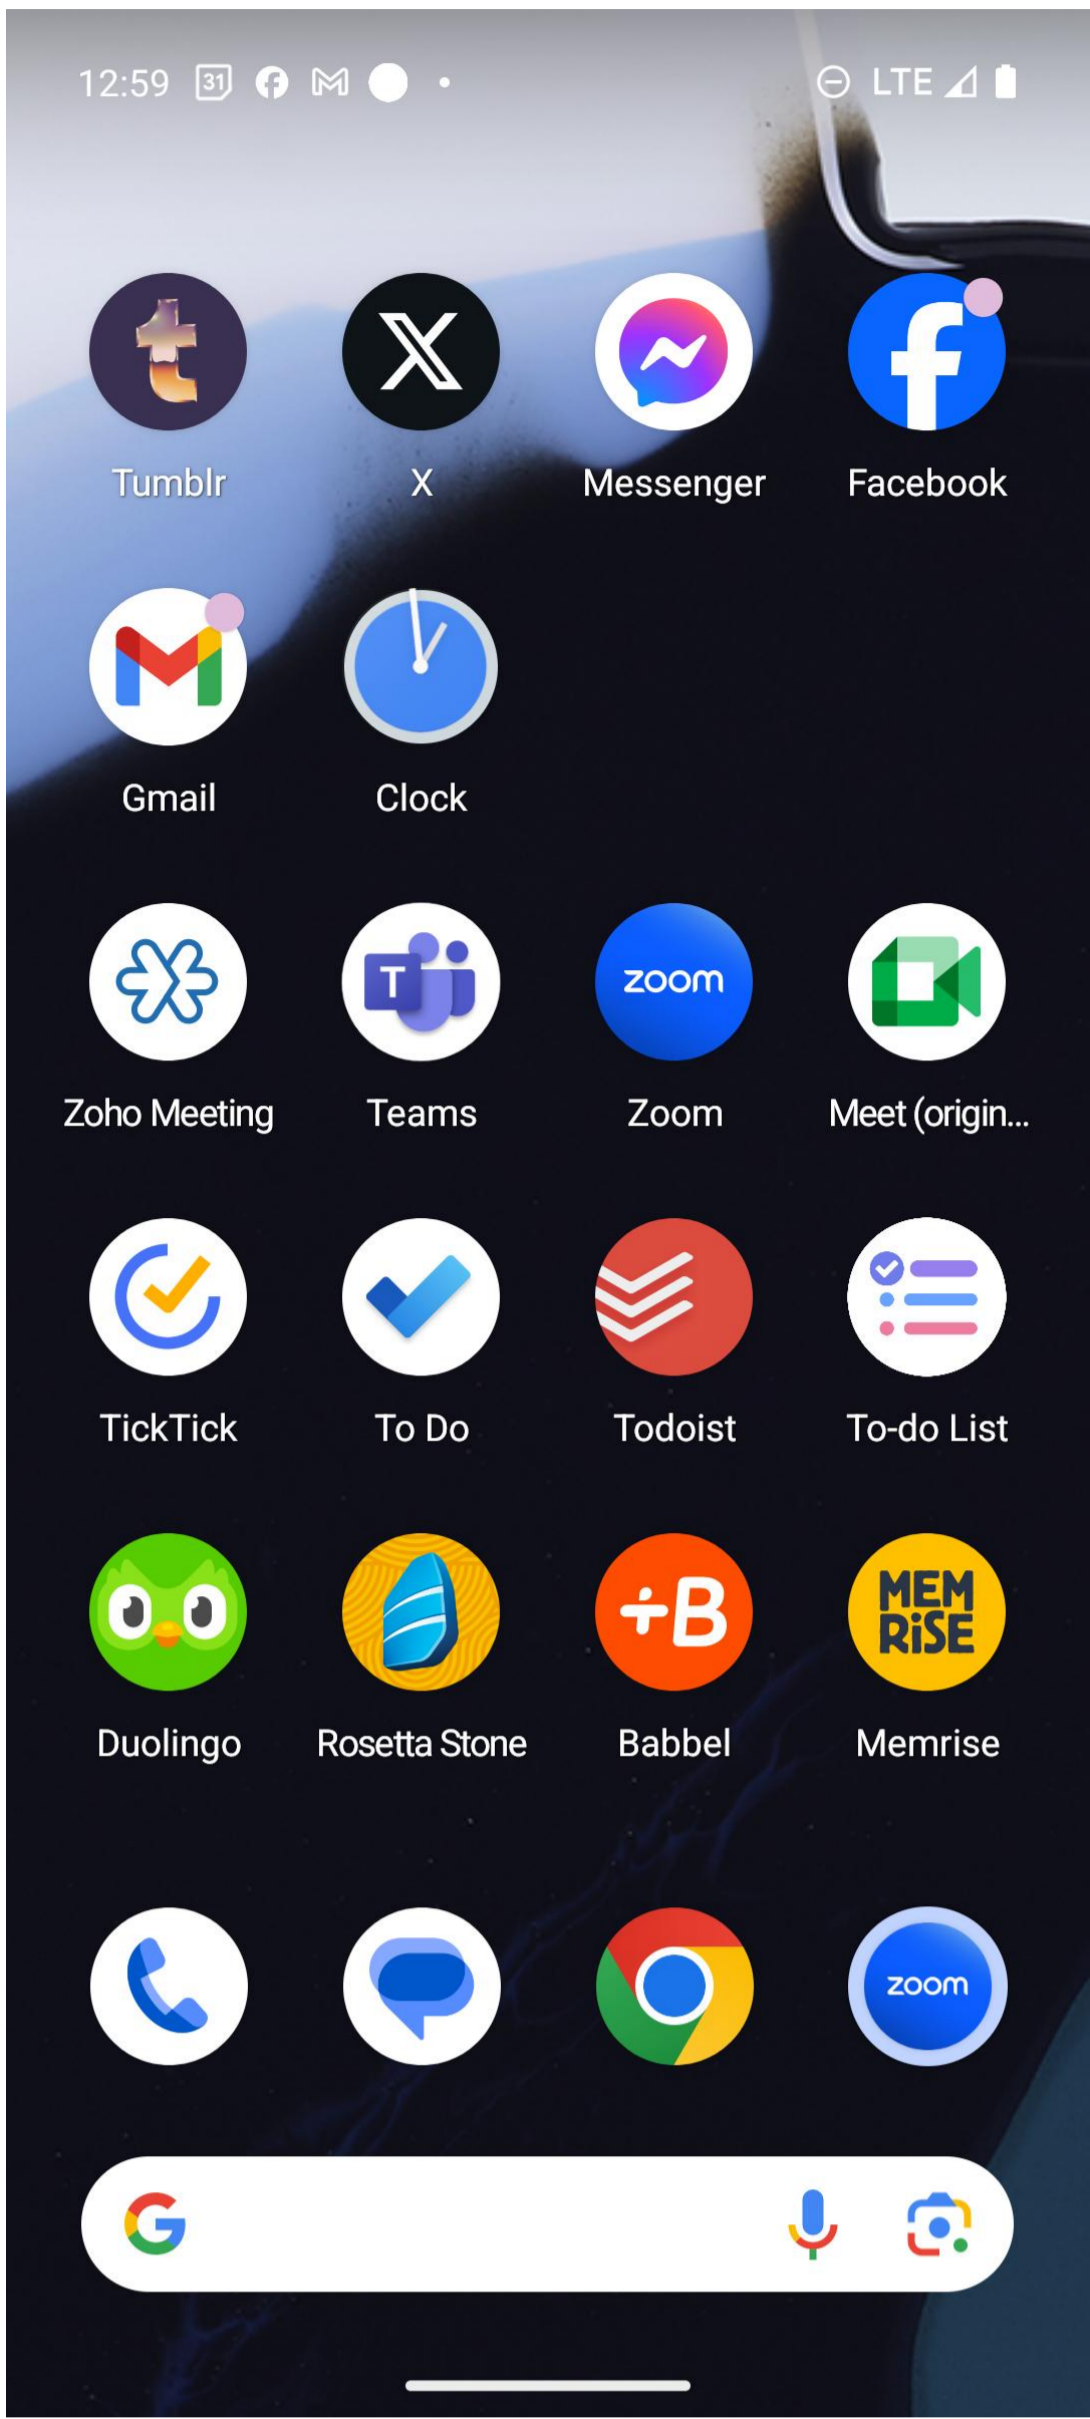

Step 1

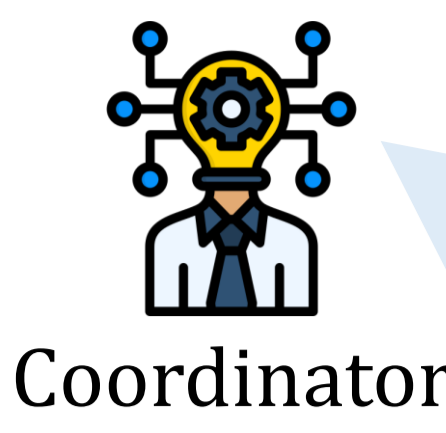

<think>I am selecting the Zoom app to start organizing a business meeting with saltyfunswweets. This action is appropriate as it is the first step in setting up the meeting, which is necessary before sending out invitations and setting an alarm.</think>  
<answer>Open the Zoom app.</answer>

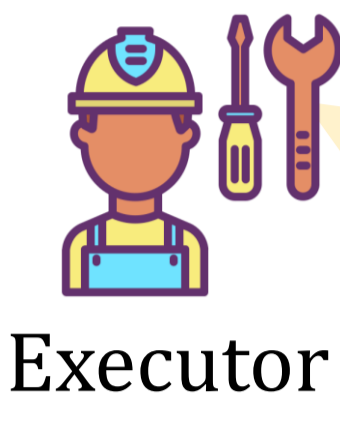

<think>The user wants to open the Zoom app. The Zoom app icon is visible on the screen, so the next step is to click on it to open the app.</think>  
<answer>CLICK: (669, 976)</answer>

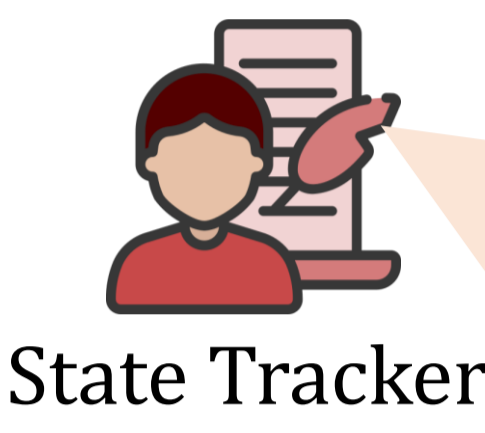

The Zoom app has been selected to start organizing a business meeting with saltyfunswweets.

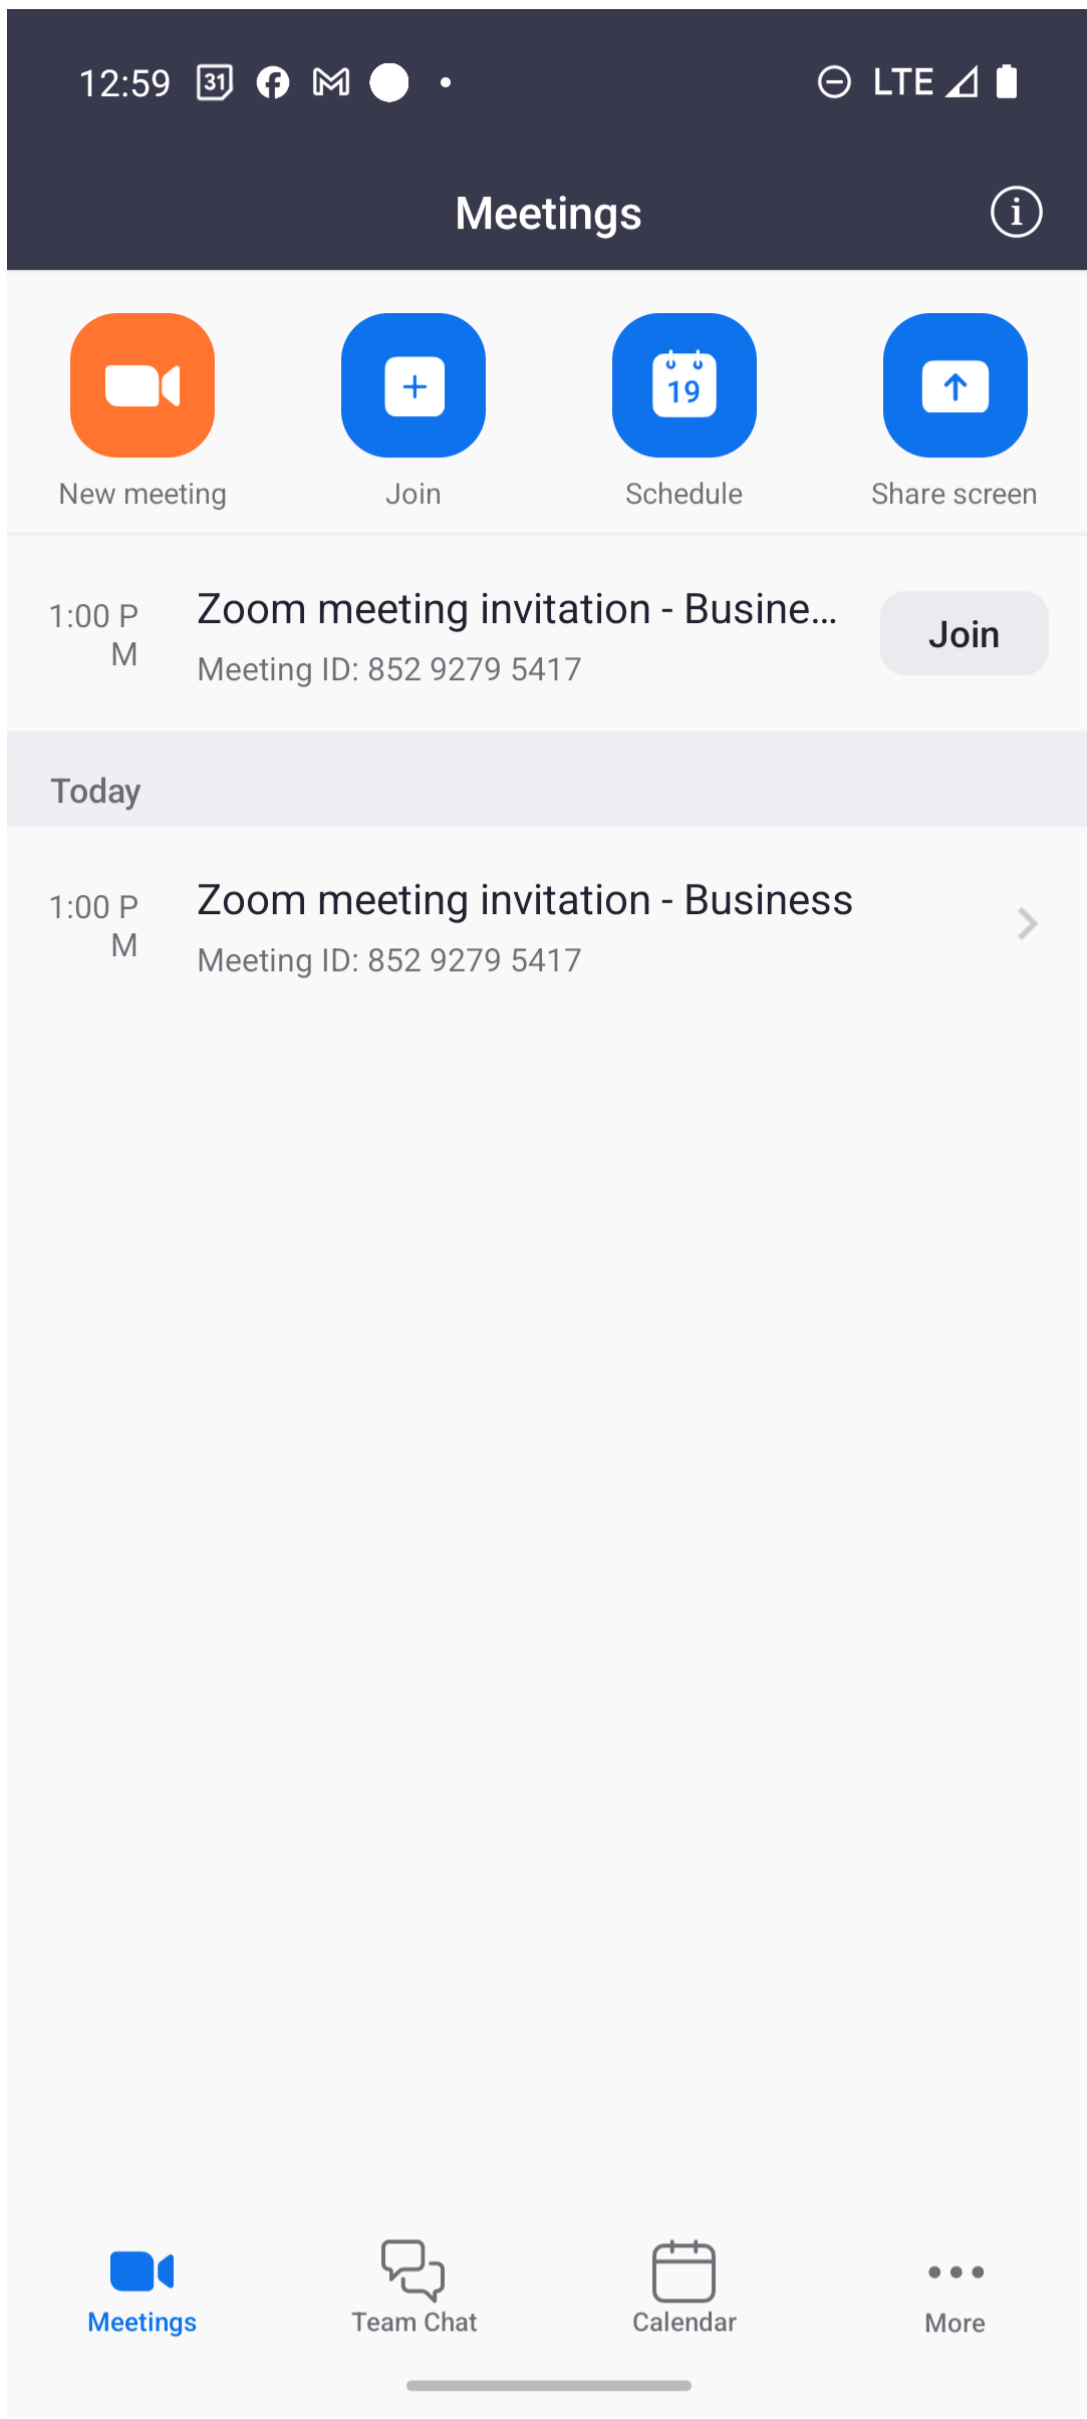

Step 2

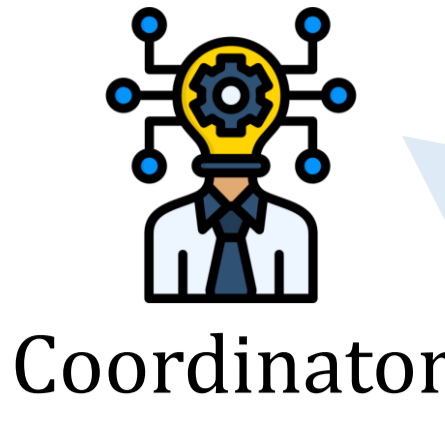

This is a screenshot of the Zoom app displaying a scheduled meeting invitation. The screen shows options to start a new meeting, join a meeting, schedule a meeting, or share a screen. I should select the 'Schedule' option to set up a new meeting. This action is appropriate as it allows me to organize the business meeting with saltyfunswweets.</think>  
<answer>Go to the schedule section.</answer>

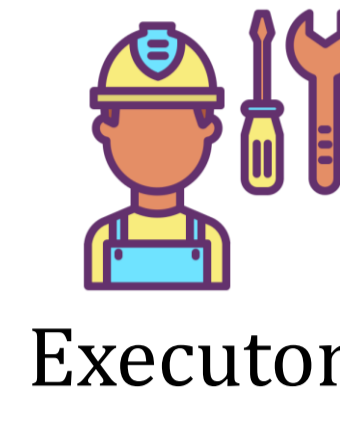

<think>The user wants to go to the schedule section. The 'Schedule' button is clearly visible in the top row of the interface. The button is located at the coordinates (678, 370) based on the layout provided.</think>  
<answer>CLICK: (678, 370)</answer>

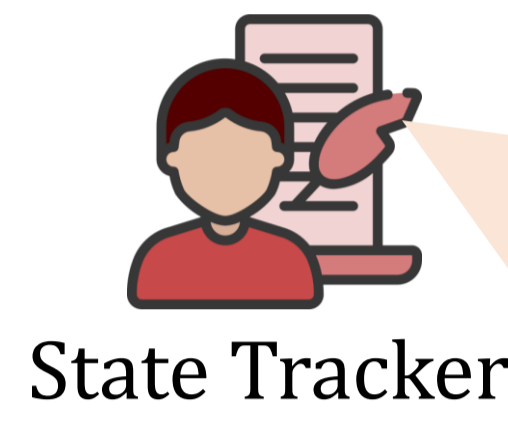

In order to organize the business meeting, I have accessed the 'Schedule' section in the Zoom app.

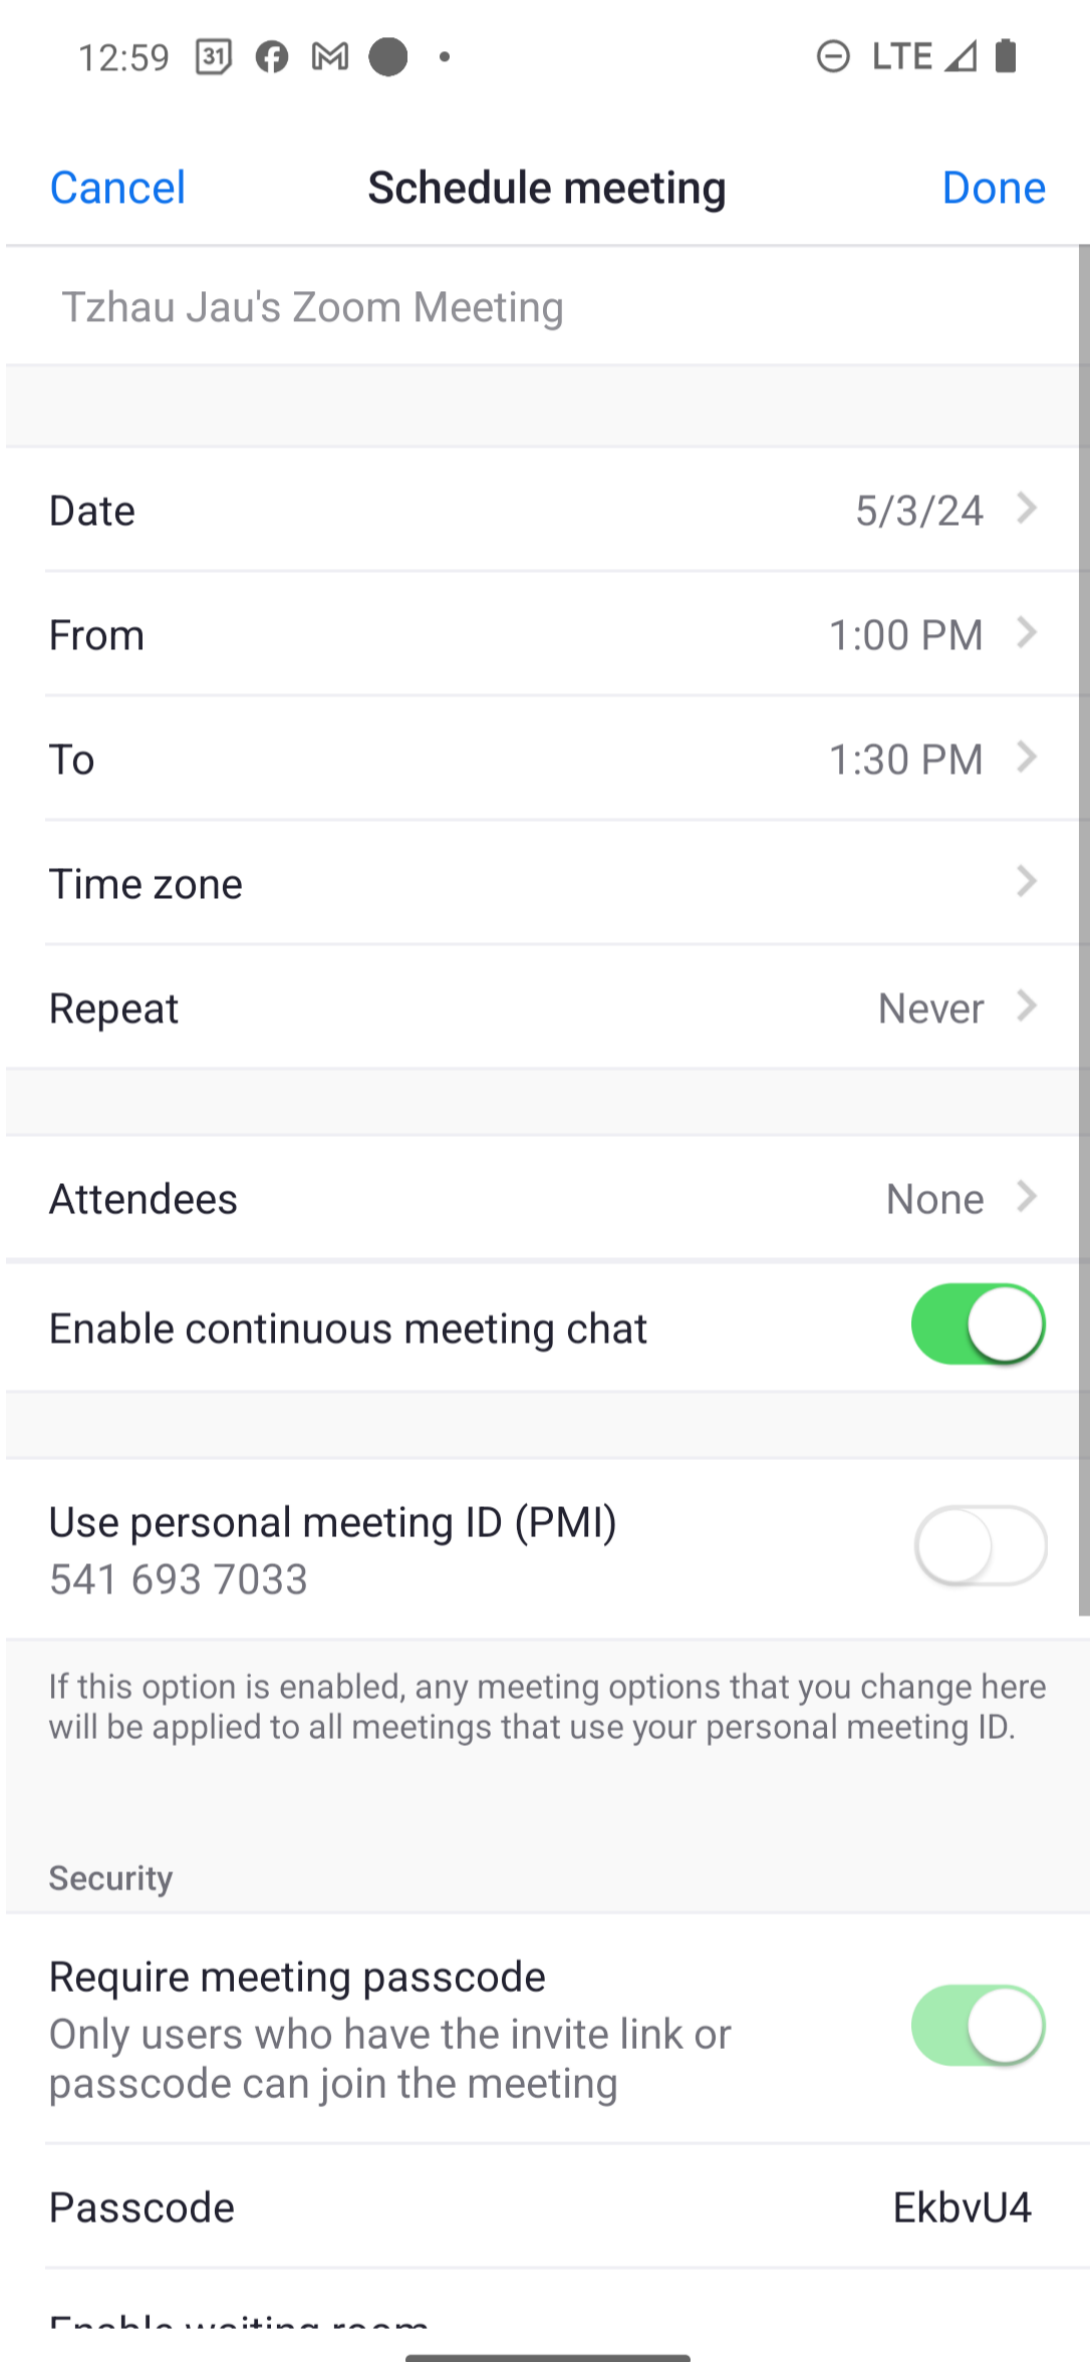

Step 3

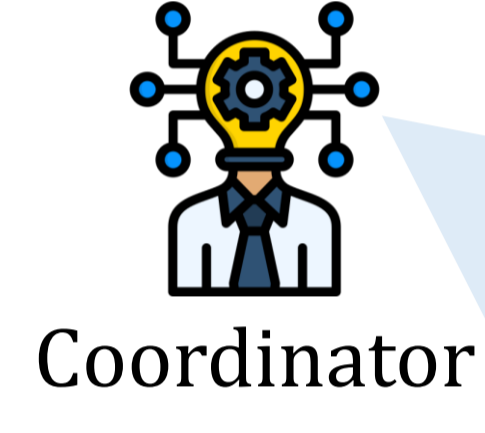

<think>I am scheduling a business meeting using the Zoom app to ensure that all necessary details are organized and ready. This step is crucial for setting the meeting time, enabling security features, and preparing to send out invitations via Tumblr.</think>  
<answer>Scroll through the meeting details to adjust settings.</answer>

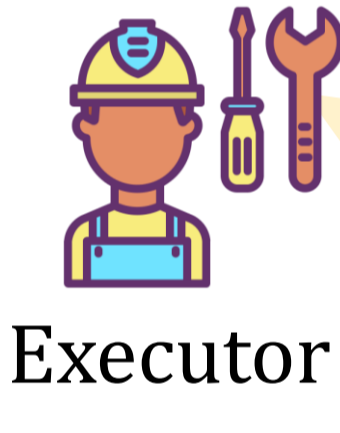

<think>The user wants to scroll through the meeting details to review or adjust settings. The current view shows a portion of the meeting details, and there are more options that are not visible on the screen.</think>  
<answer>SCROLL: DOWN</answer>

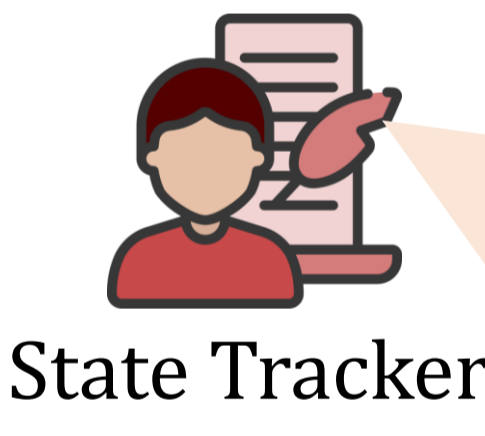

The process of organizing a business meeting with saltyfunswweets has commenced by selecting the Zoom app.

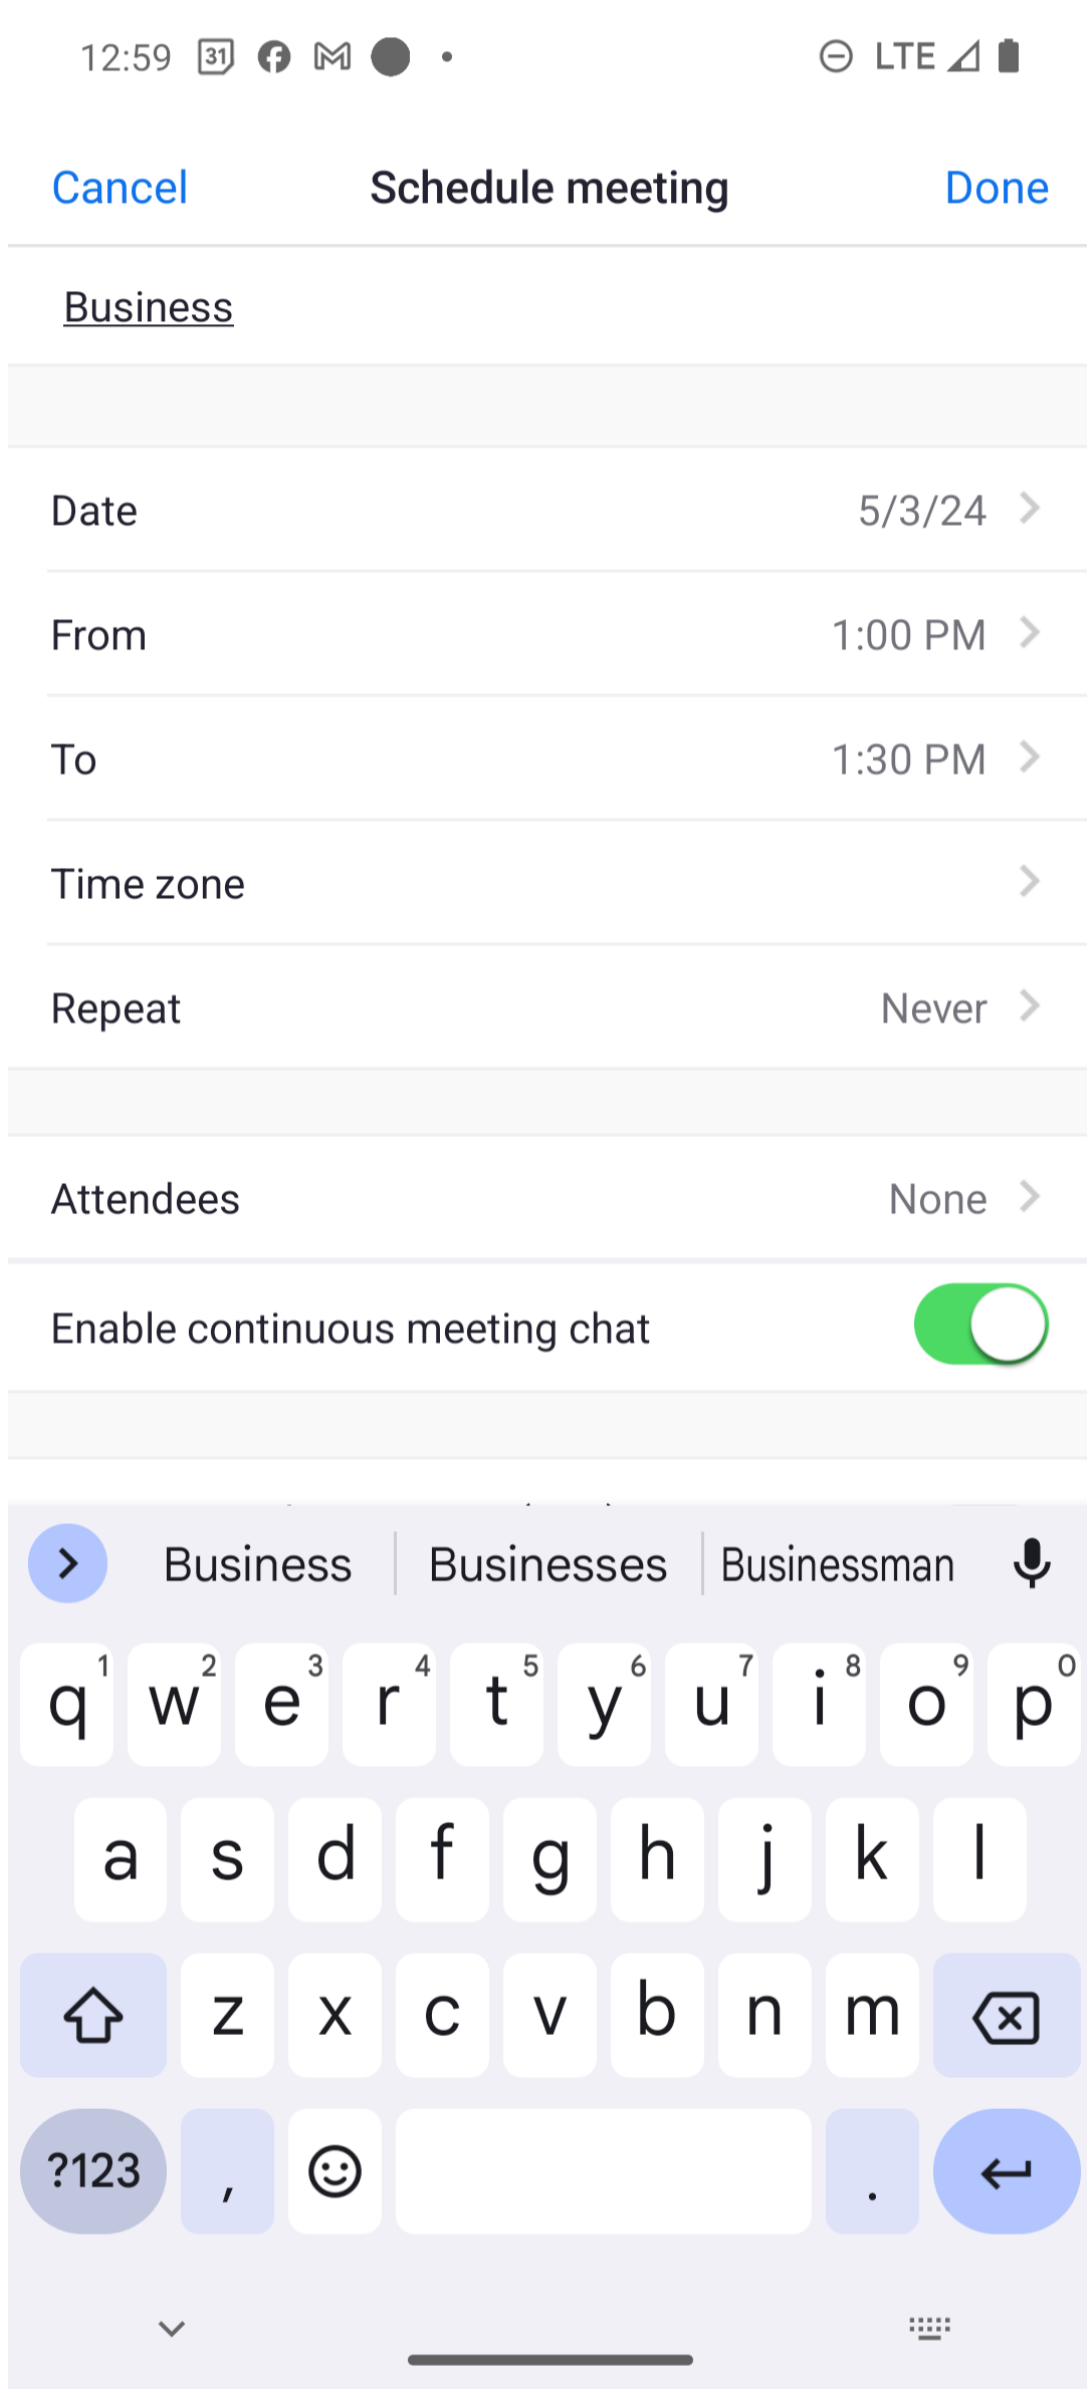

Step 4

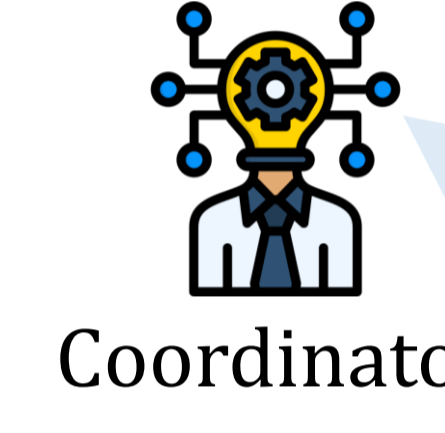

<think>This is a screenshot of the Zoom app's 'Schedule meeting' screen, where details for a business meeting are being set. The user is in the process of finalizing the meeting settings, including date, time, and other options. I am confirming the meeting details to finalize the scheduling process. By clicking 'Done,' I ensure that the meeting is set up correctly and can proceed to send out invitations via Tumblr.</think>  
<answer>Confirm the meeting schedule by clicking 'Done.'</answer>

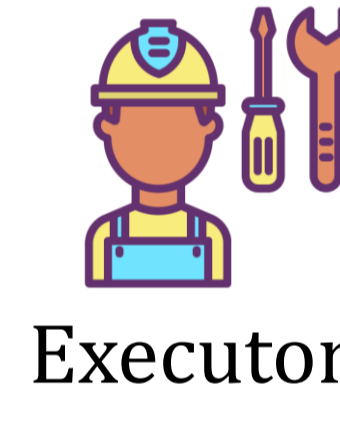

<think>The user wants to confirm the meeting schedule. The 'Done' button is visible at the top right of the screen, which is typically used to finalize or confirm actions in such interfaces. Clicking this button will likely save the meeting details and complete the scheduling process.</think>  
<answer>CLICK: (994, 203)</answer>

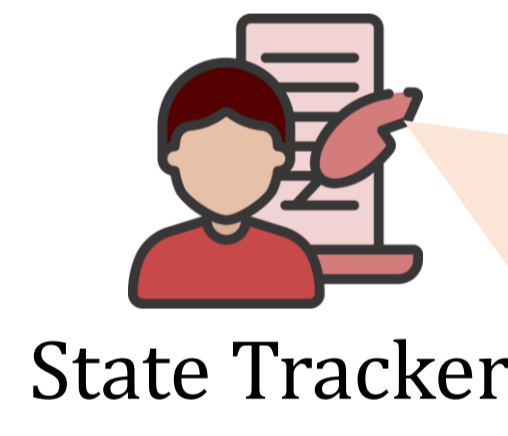

The Zoom app has been accessed to organize a business meeting with saltyfunswweets. The meeting has been scheduled by selecting the appropriate options and entering the necessary details. The setup has been confirmed by finalizing the scheduling process.

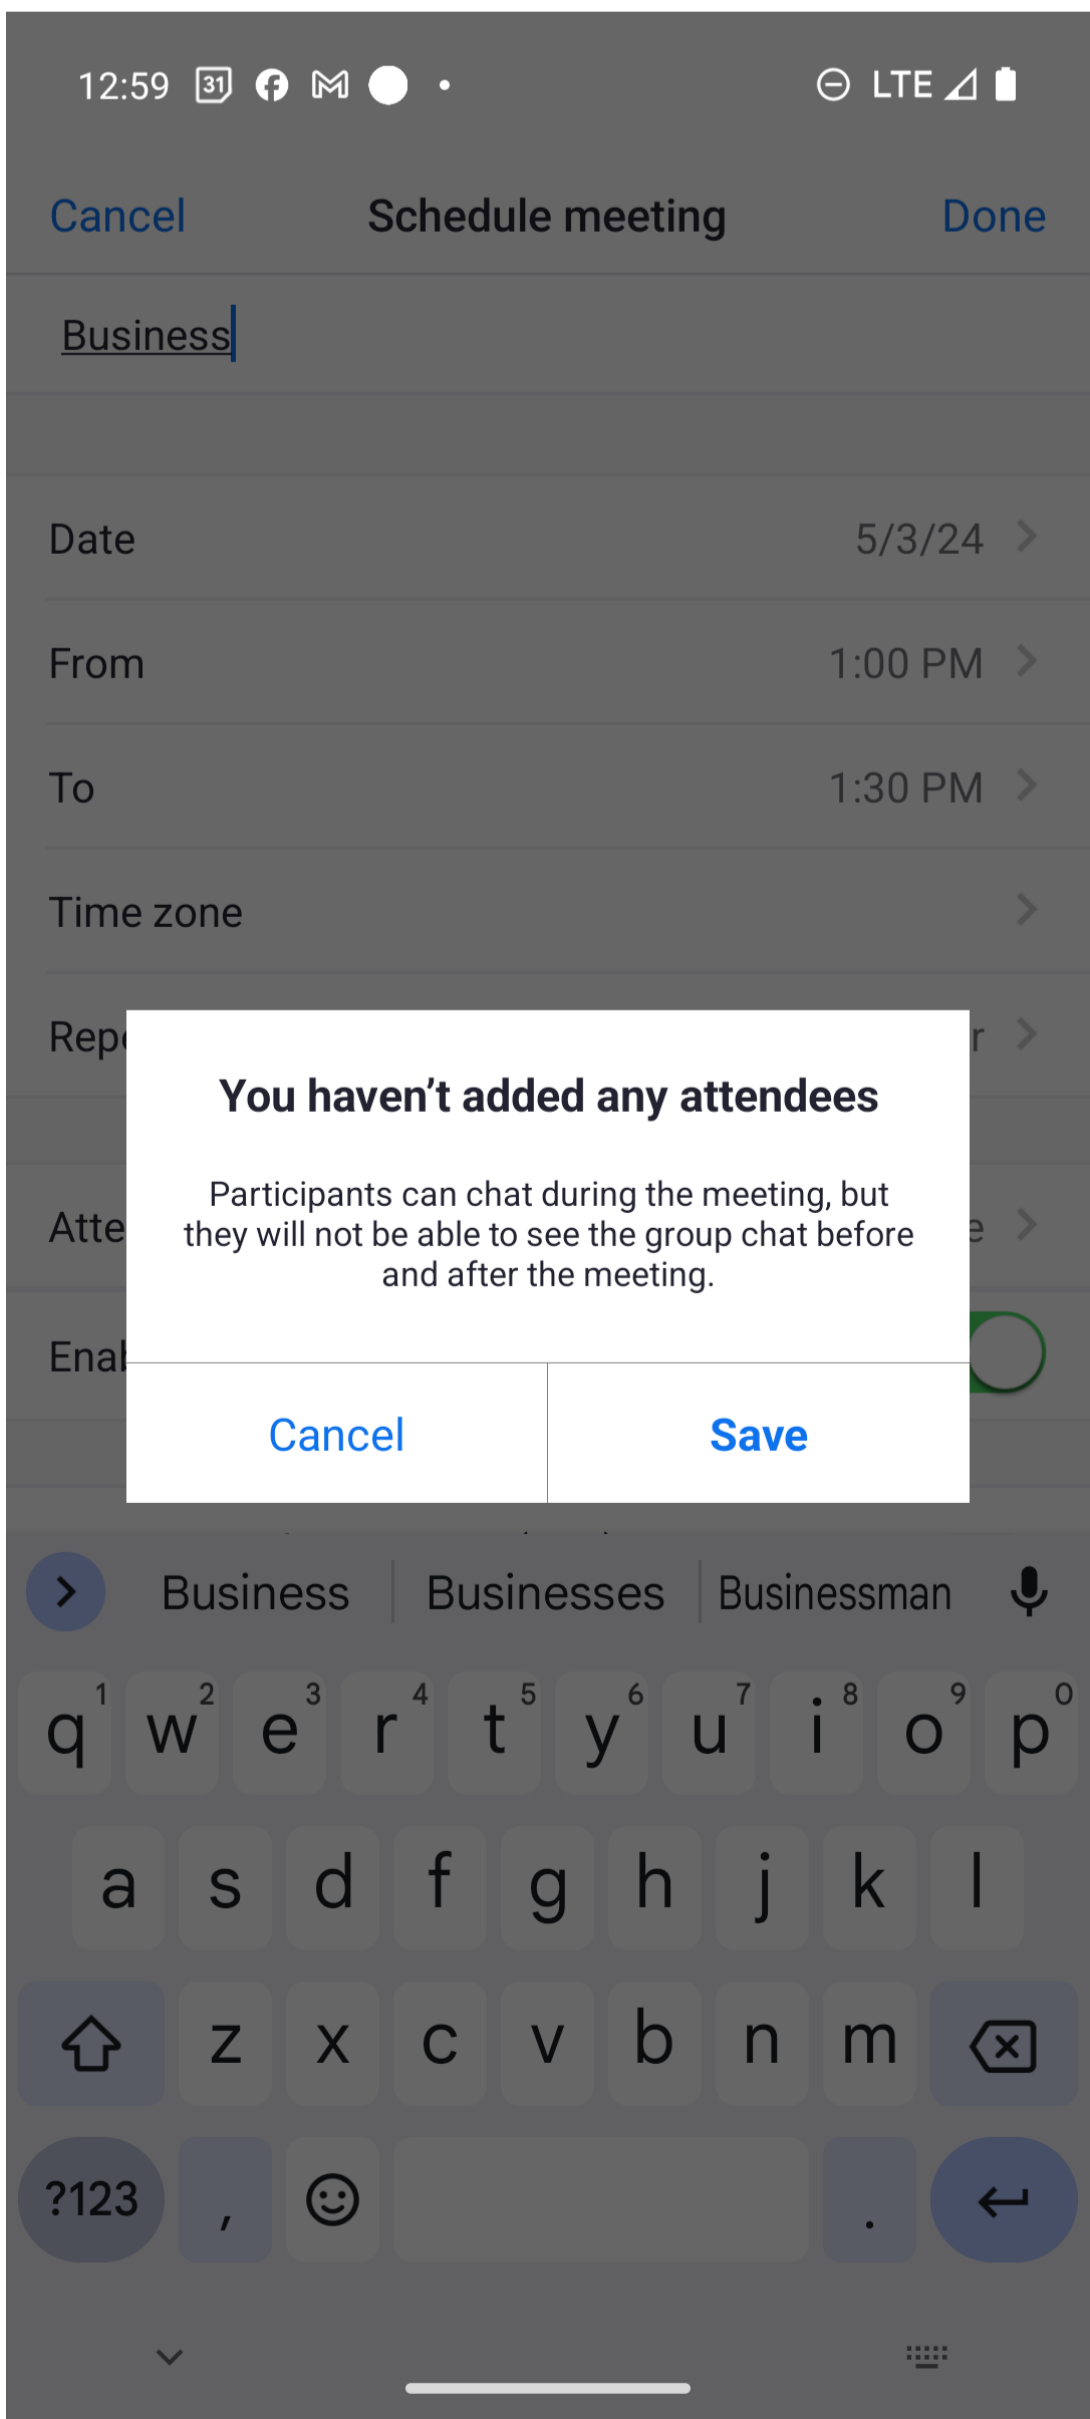

Step 5

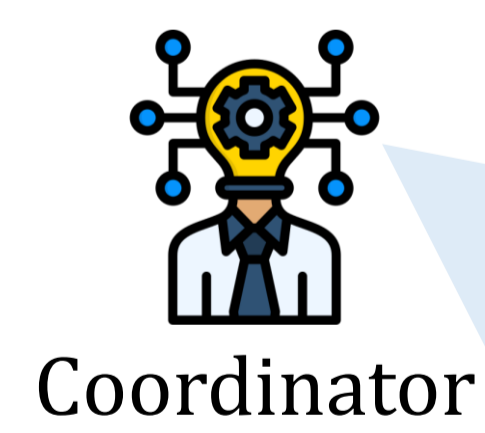

<think>This is a screenshot a pop-up message indicating that no attendees have been added. The options to 'Cancel' or 'Save' the meeting are presented. I am choosing to save the meeting despite not having added any attendees because I need to finalize the scheduling process. This action allows me to proceed with sending out invitations via Tumblr and setting an alarm for the meeting time.</think>  
<answer>Save the meeting without adding attendees.</answer>

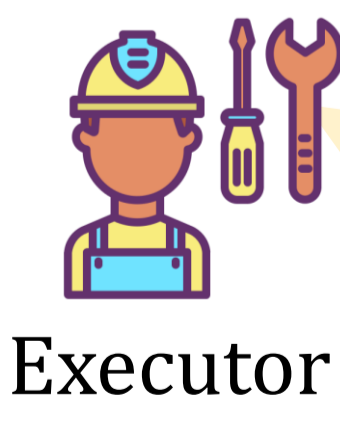

<think>The user wants to save the meeting without adding attendees. The current screen shows a dialog box with the option to 'Save' or 'Cancel'. Since the user's goal is to save the meeting without adding attendees, the appropriate action is to click the 'Save' button.</think>  
<answer>CLICK: (756, 1422)</answer>

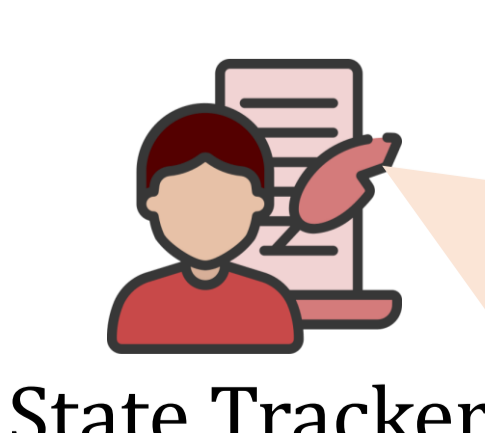

The Zoom app has been accessed to organize a business meeting with saltyfunswweets, and the meeting has been scheduled with all necessary details confirmed and saved.

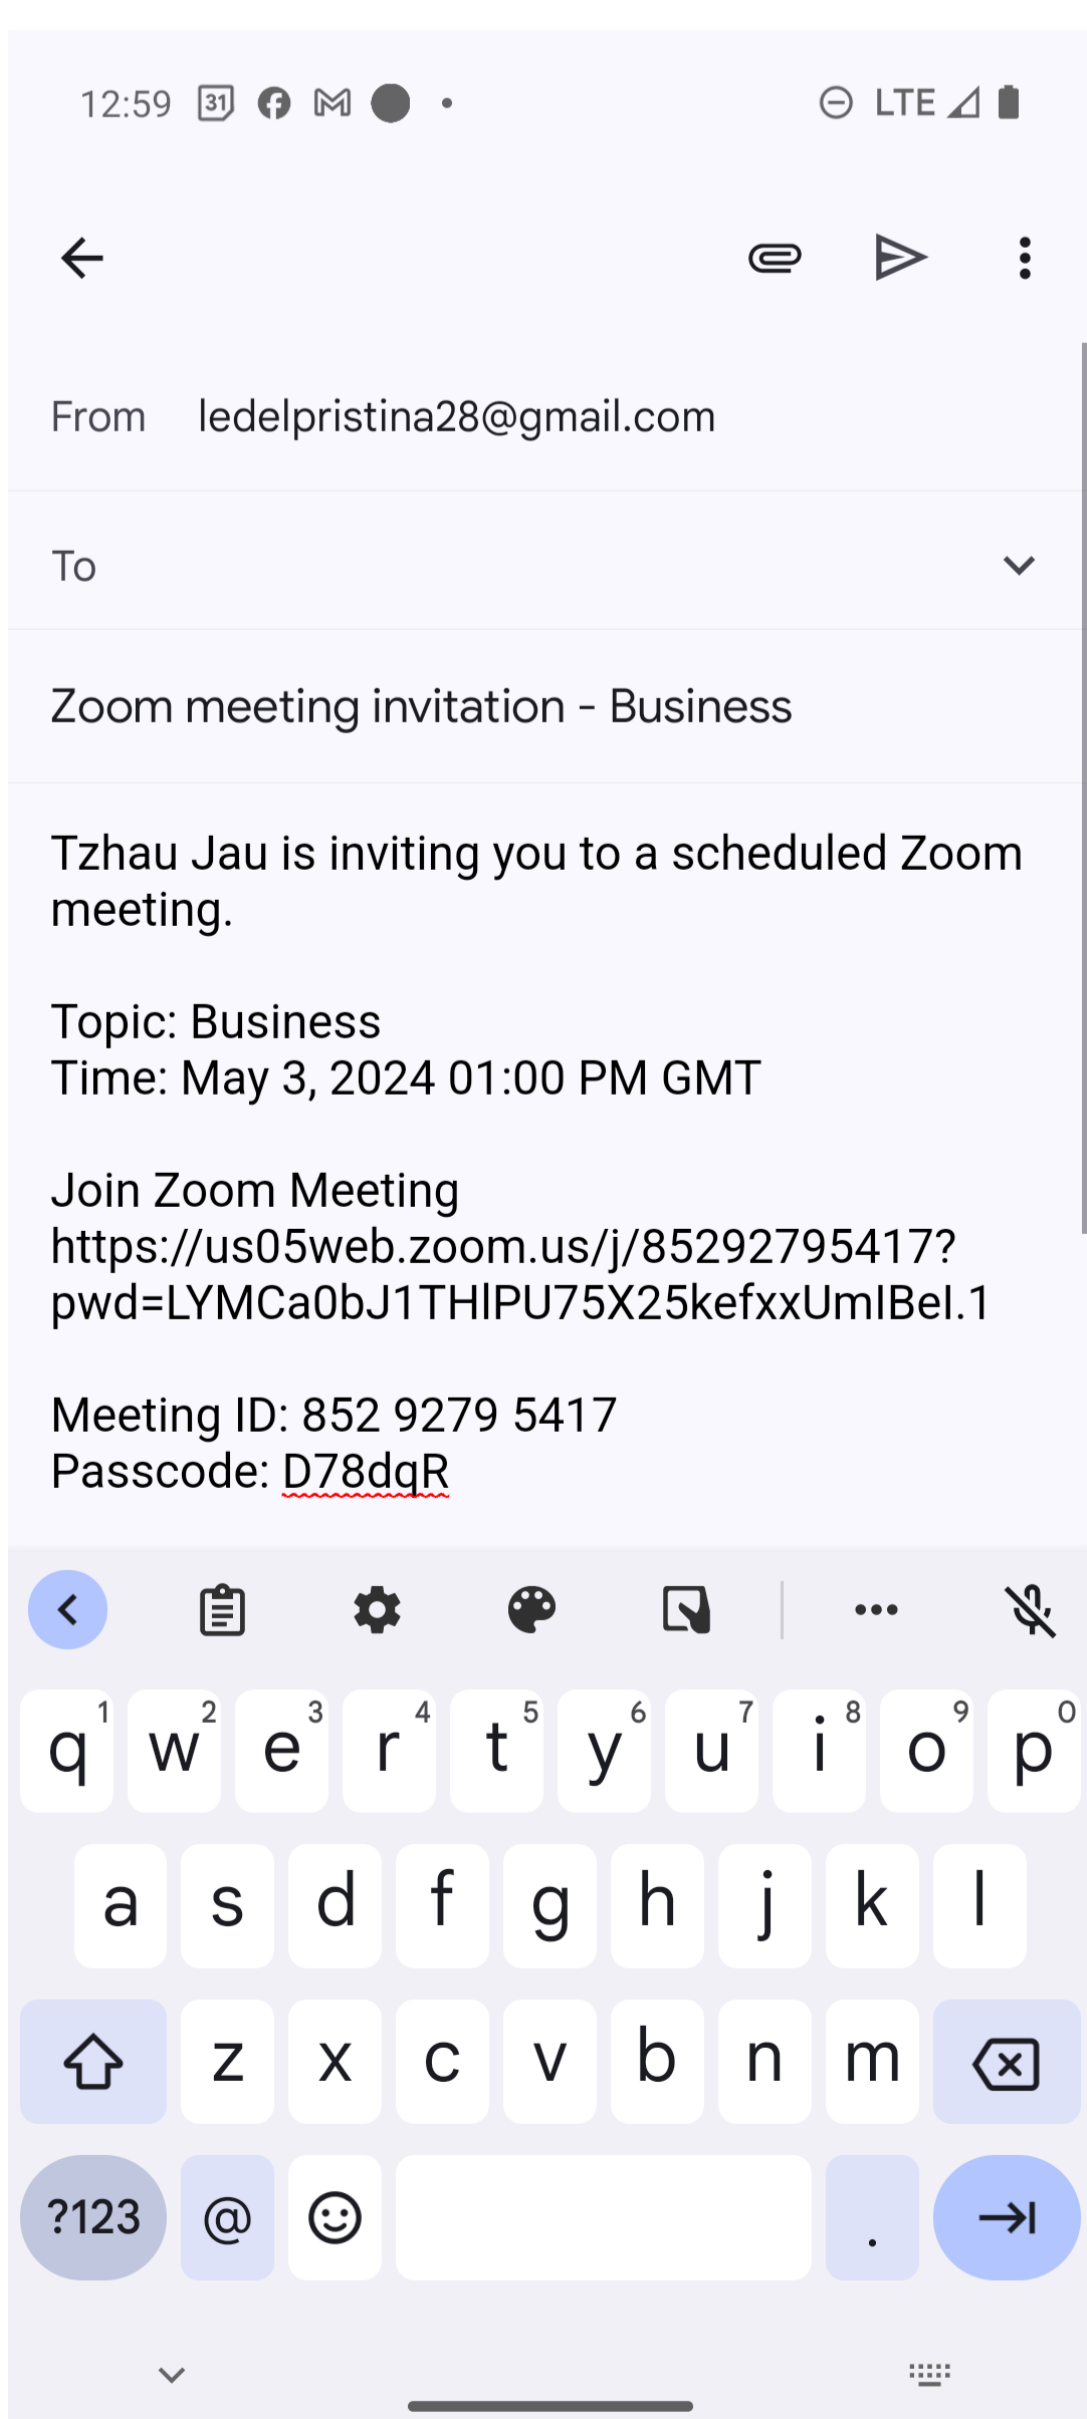

Step 6

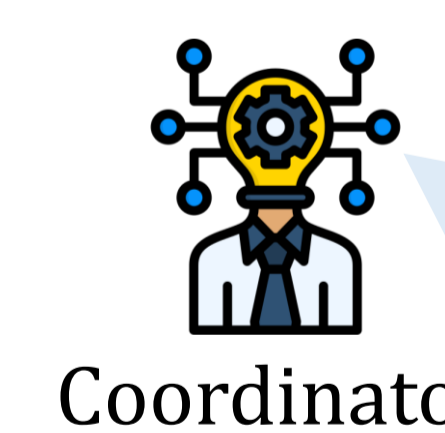

<think>I am pressing the home button to exit the email app and proceed to the next steps in my task. Since the meeting details are confirmed and saved, I will now send out invitations via Tumblr and set an alarm for the meeting using the Clock app. This action allows me to efficiently continue organizing the meeting.</think>  
<answer>Return to the home screen.</answer>

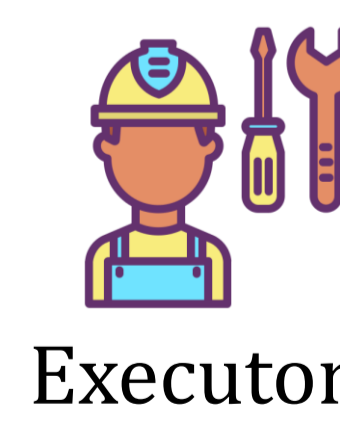

<think>The user wants to return to the home screen. The current screen shows an email containing a Zoom meeting invitation. The email includes details such as the meeting topic, date, time, and a link to join the meeting, along with the meeting ID and passcode.</think>  
<answer>PRESS\_HOME</answer>

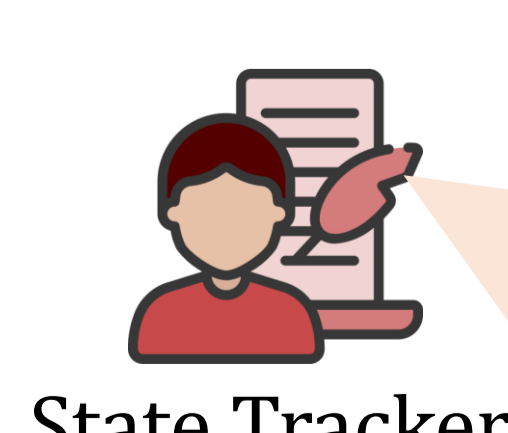

The Zoom app has been accessed to organize a business meeting with saltyfunswweets. The meeting has been scheduled by selecting the appropriate options and entering the necessary details. The setup has been confirmed by finalizing the scheduling process.

# User Instruction

Organize a business meeting with saltyfunsweets using ZOOM Cloud Meetings, send out the meeting invitations via Tumblr, and set an alarm clock for the meeting time using the Clock app.

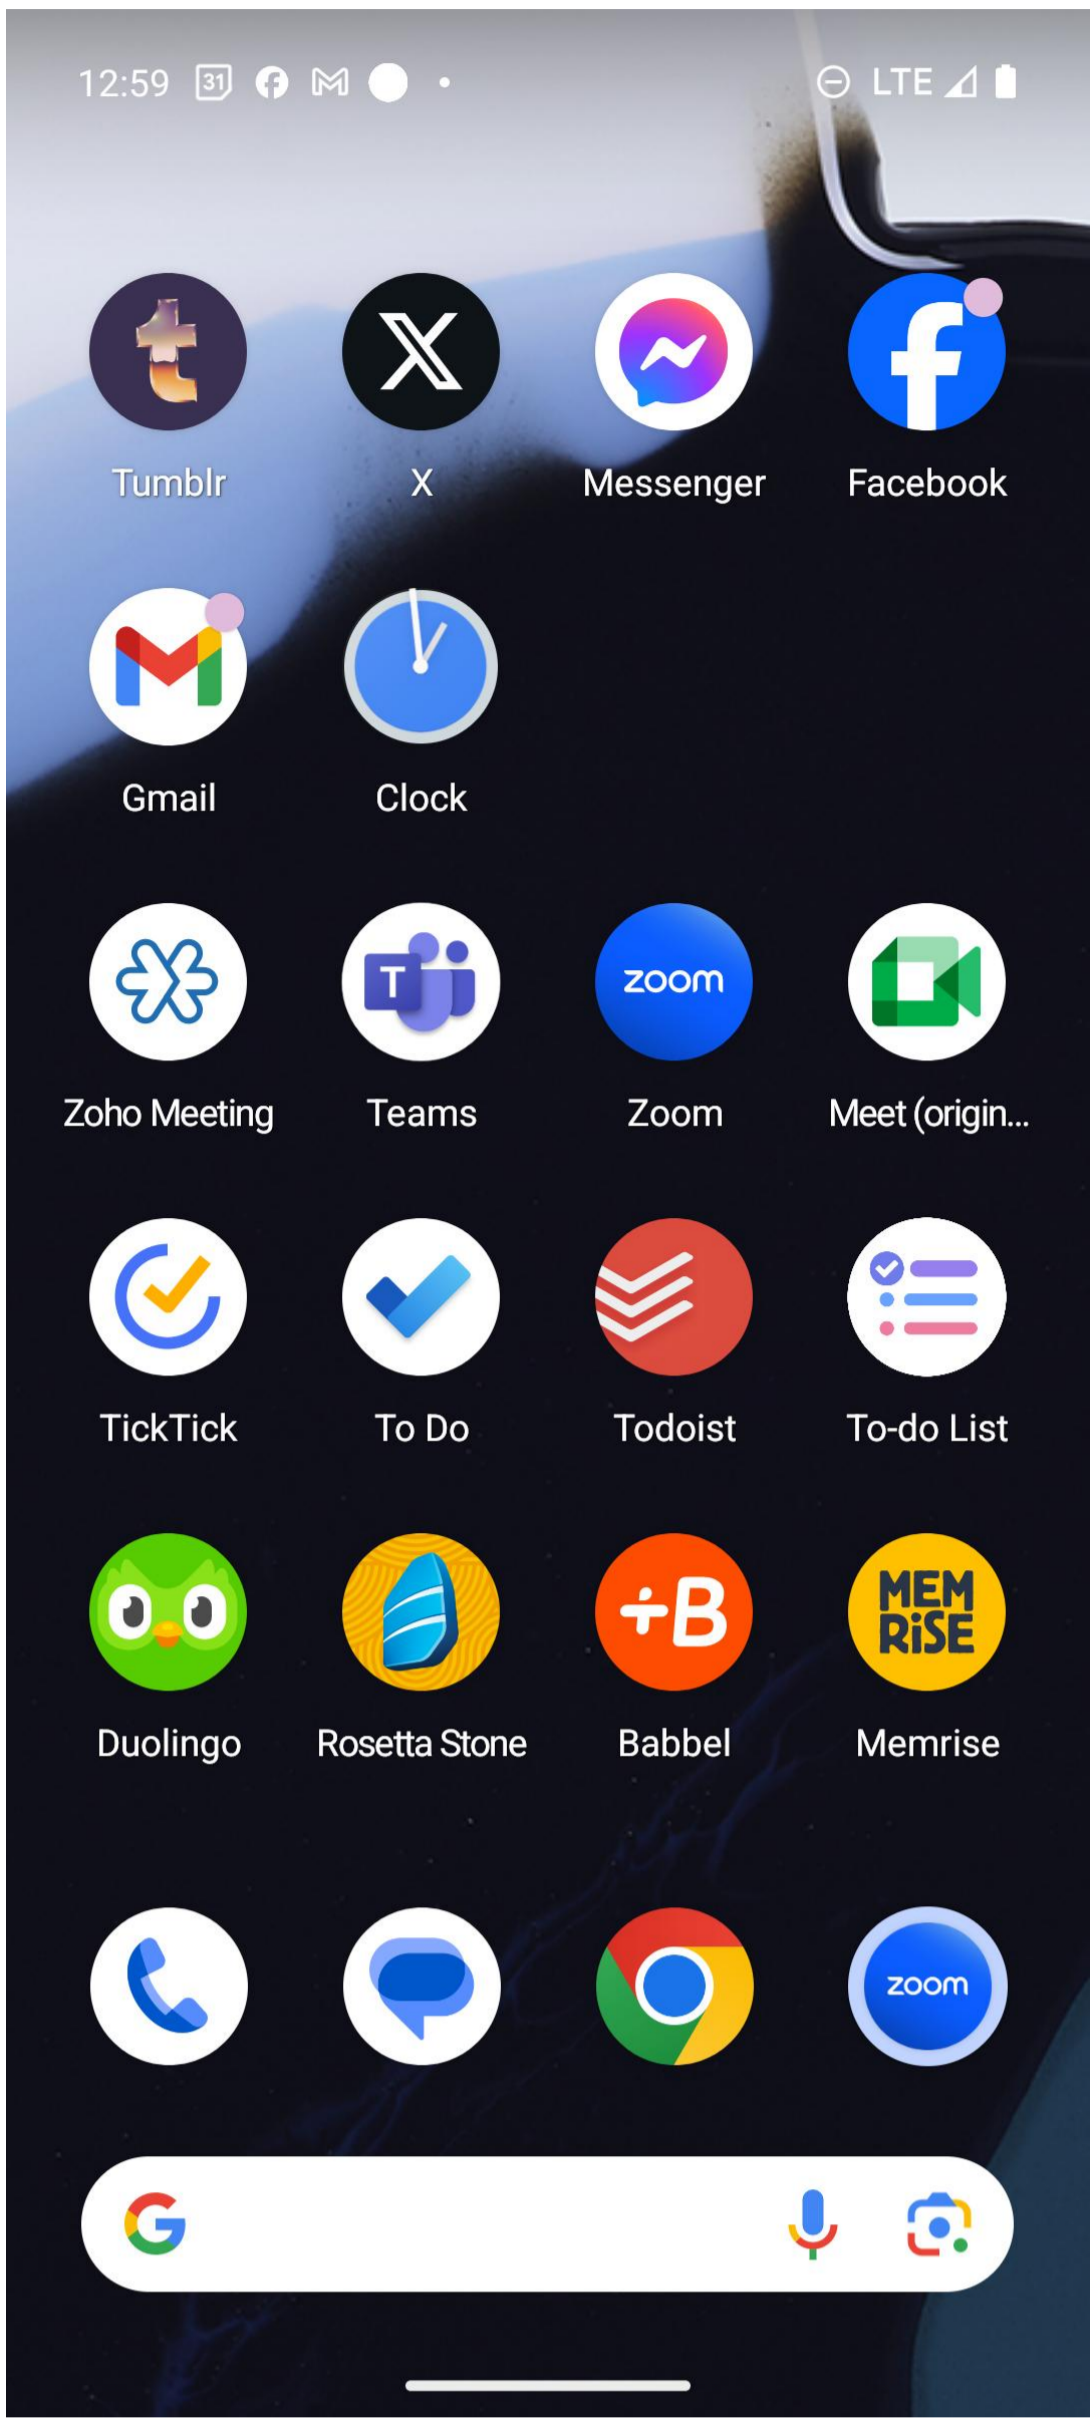

Step 7

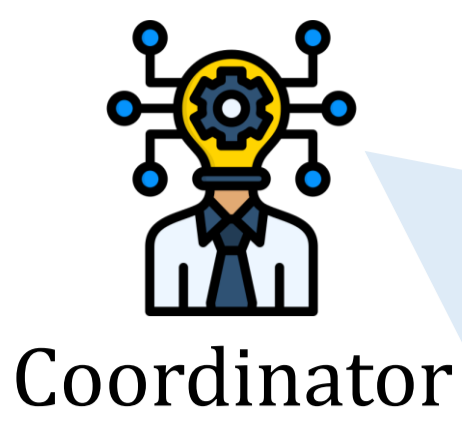

Coordinator

<think>I am selecting the Zoom app to ensure that the business meeting details with saltyfunsweets are finalized and to proceed with sending out invitations via Tumblr. This action is appropriate as it confirms the meeting setup before moving on to the next task of sending invitations.</think>  
<answer>**Open the Zoom app.**</answer>

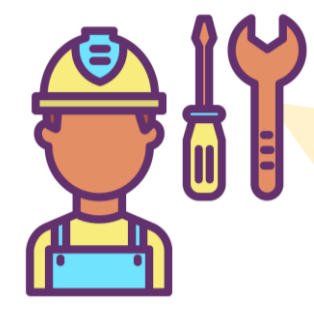

Executor

<think>The user wants to open the Zoom app. The Zoom app icon is visible on the screen, so the next step is to click on it to open the app.</think>  
<answer>**CLICK: (669, 976)**</answer>

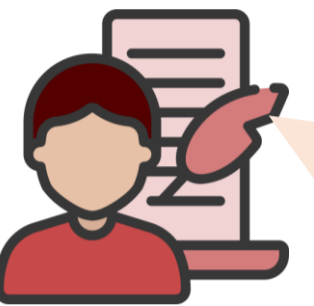

State Tracker

The Zoom app has been accessed, and a business meeting with saltyfunsweets has been scheduled, with all necessary details confirmed and saved. The process has progressed to the point where the meeting setup is complete.

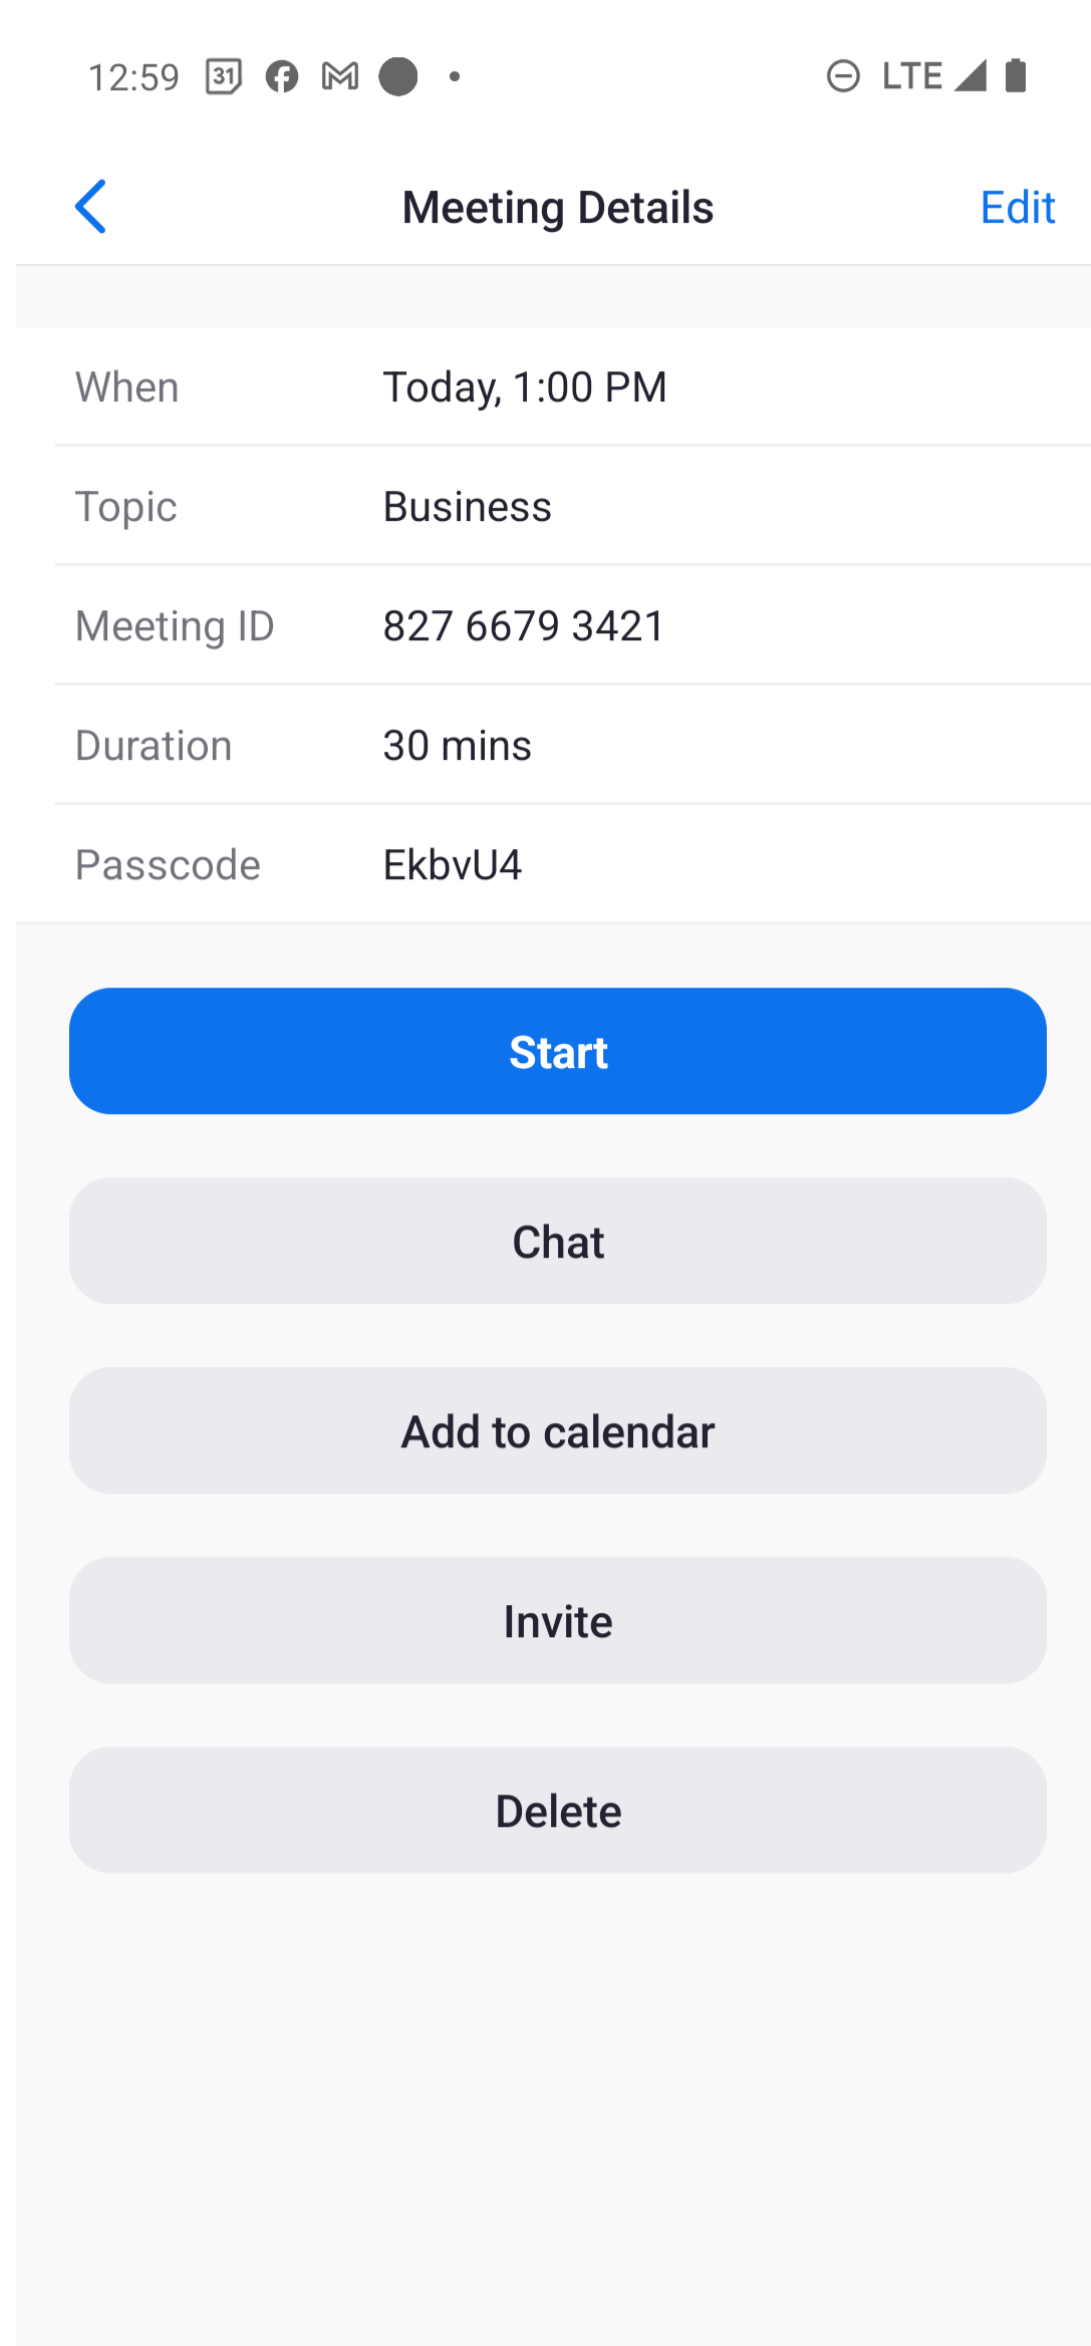

Step 8

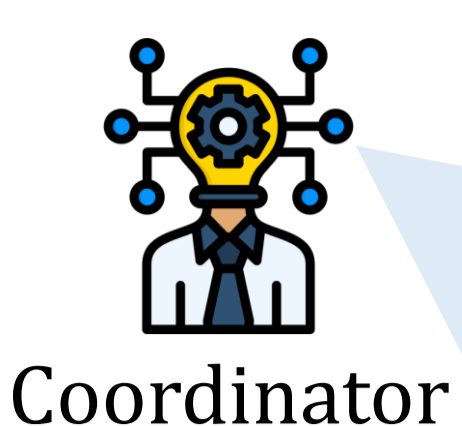

Coordinator

<think>I am choosing to click on the 'Invite' button to send out the meeting invitations for the business meeting with saltyfunsweets. By doing this, I am progressing towards completing the task of organizing the meeting and sending out invitations.</think>  
<answer>**Select the 'Invite' option.**</answer>

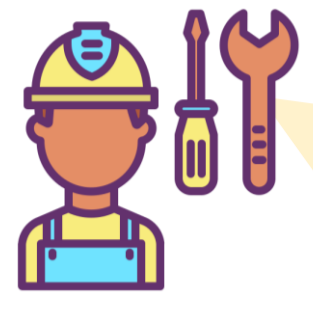

Executor

<think>The user wants to Select the 'Invite' option.The 'Invite' button is visible on the screen, which is the appropriate action to share the meeting details with the necessary participants. This aligns with the goal of organizing the meeting and ensuring all participants receive the invitation to join the Zoom meeting.</think>  
<answer>**CLICK: (546, 1616)**</answer>

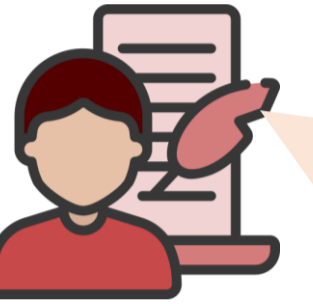

State Tracker

The business meeting with saltyfunsweets has been organized using the Zoom app. The meeting details have been scheduled and saved, and the process of sending out invitations via Tumblr has been initiated by selecting the 'Invite' option.

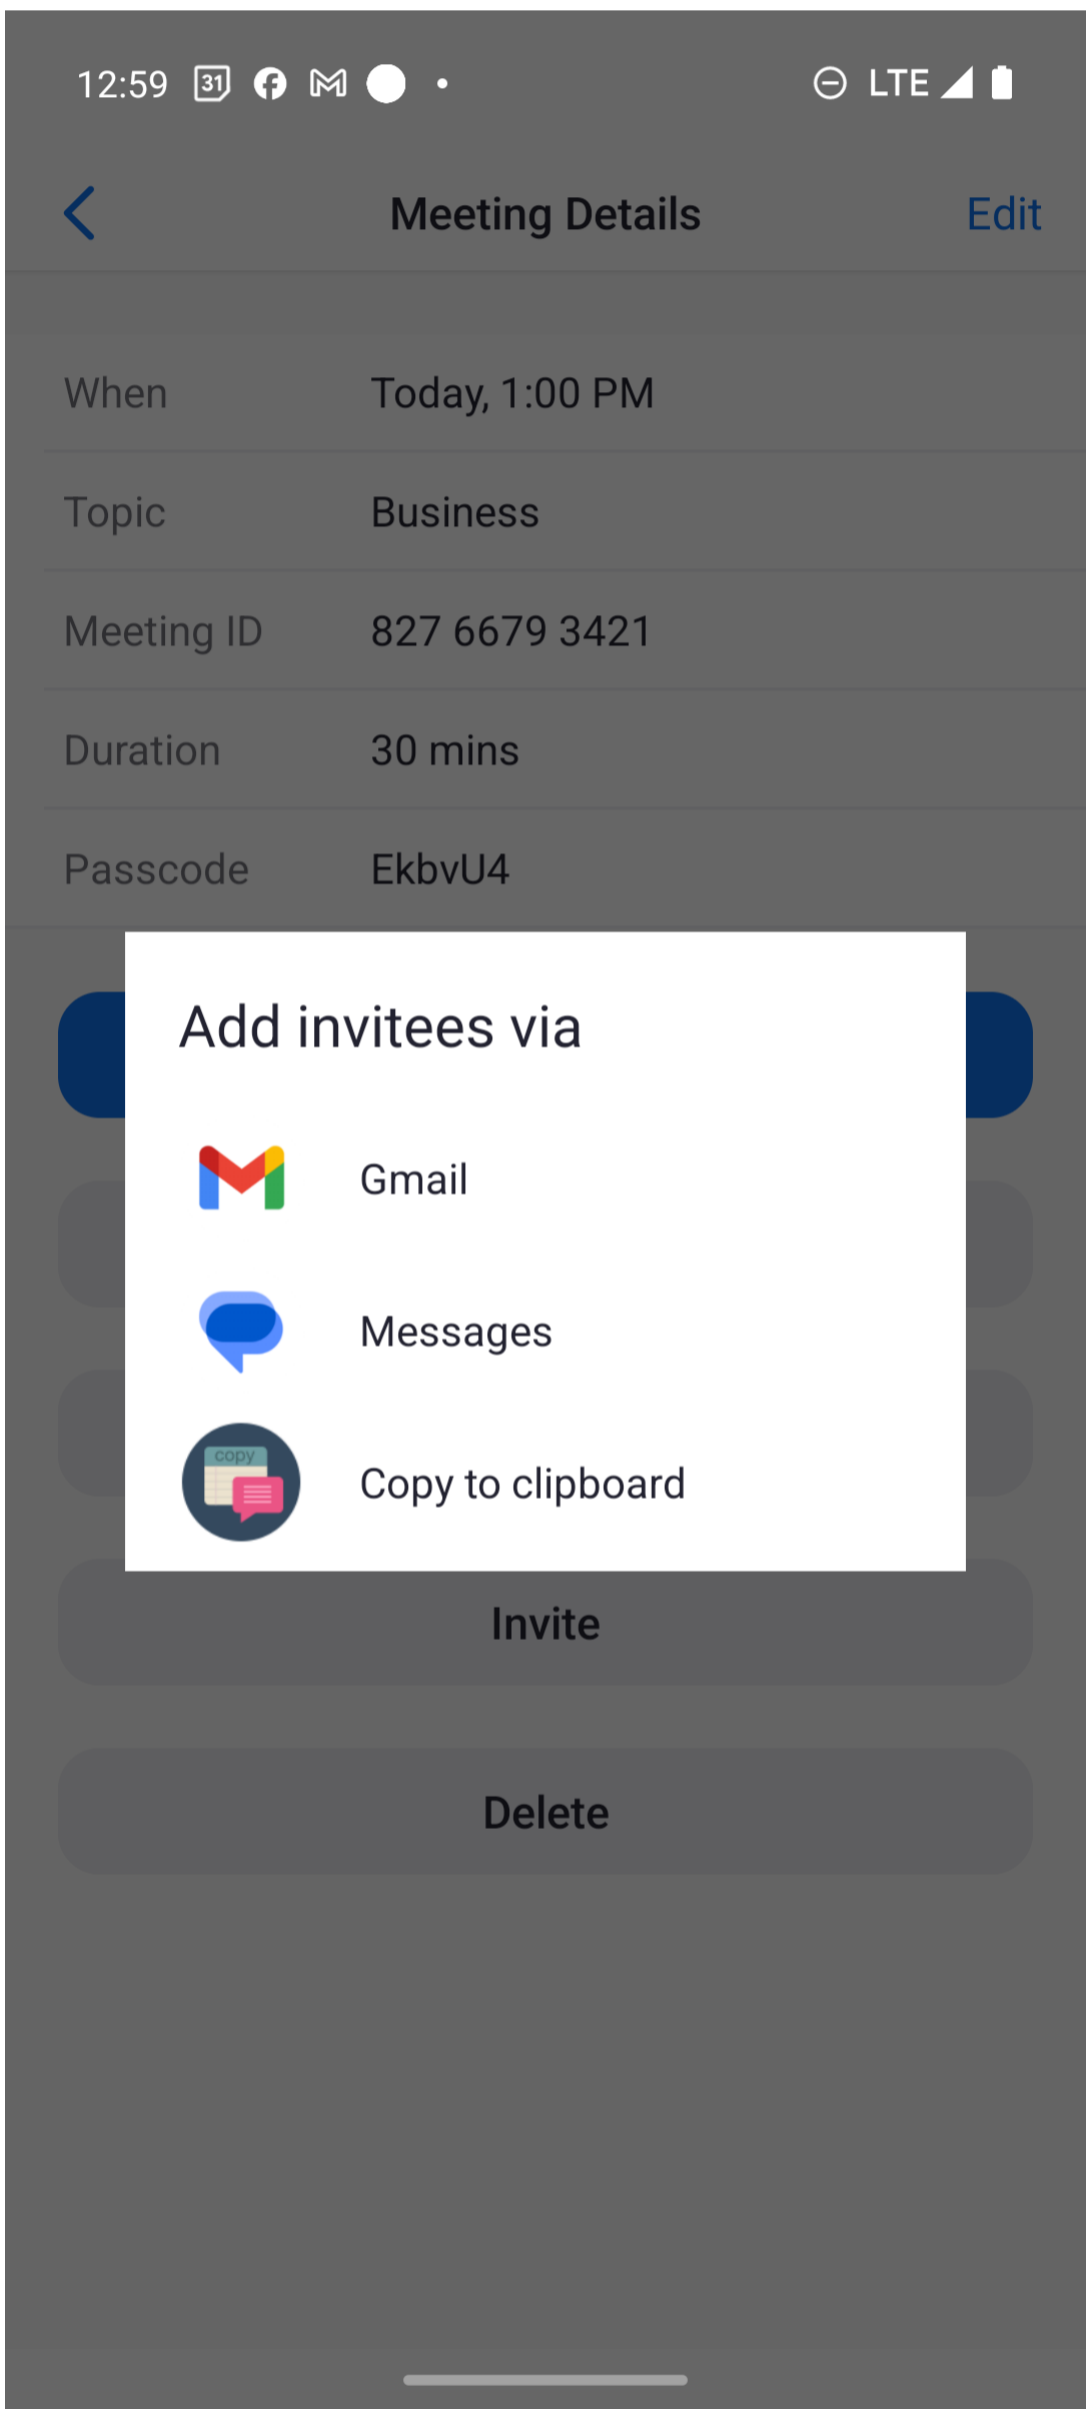

Step 9

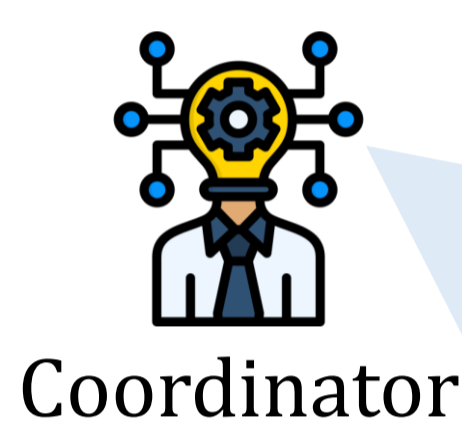

Coordinator

This is a screenshot of a Zoom meeting details screen showing options to add invitees via different apps or copy the meeting link to the clipboard. The user is prompted to choose how to send the meeting invitation.I am choosing to copy the meeting link to the clipboard so I can easily paste it into the Tumblr app to send out the meeting invitations. This allows me to efficiently share the meeting details with the intended recipients.</think>  
<answer>**Copy the meeting link to the clipboard.**</answer>

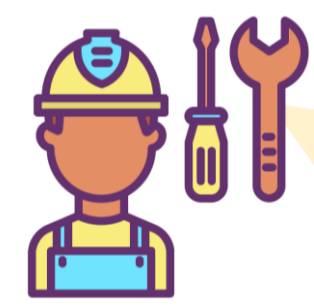

Executor

<think>The user wants to copy the meeting link to the clipboard. The current screen shows a pop-up with options to add invitees via Gmail, Messages, or to copy the link to the clipboard. The 'Copy to clipboard' option is available, which is the action needed to fulfill the user's request.</think>  
<answer>**CLICK: (525, 1476)**</answer>

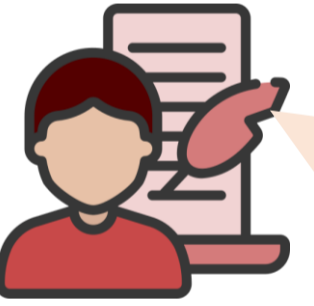

State Tracker

The Zoom app has been used to schedule a business meeting with saltyfunsweets, ensuring all necessary details are finalized. The meeting setup has been confirmed and saved, and the meeting details have been copied to the clipboard for sharing via Tumblr.

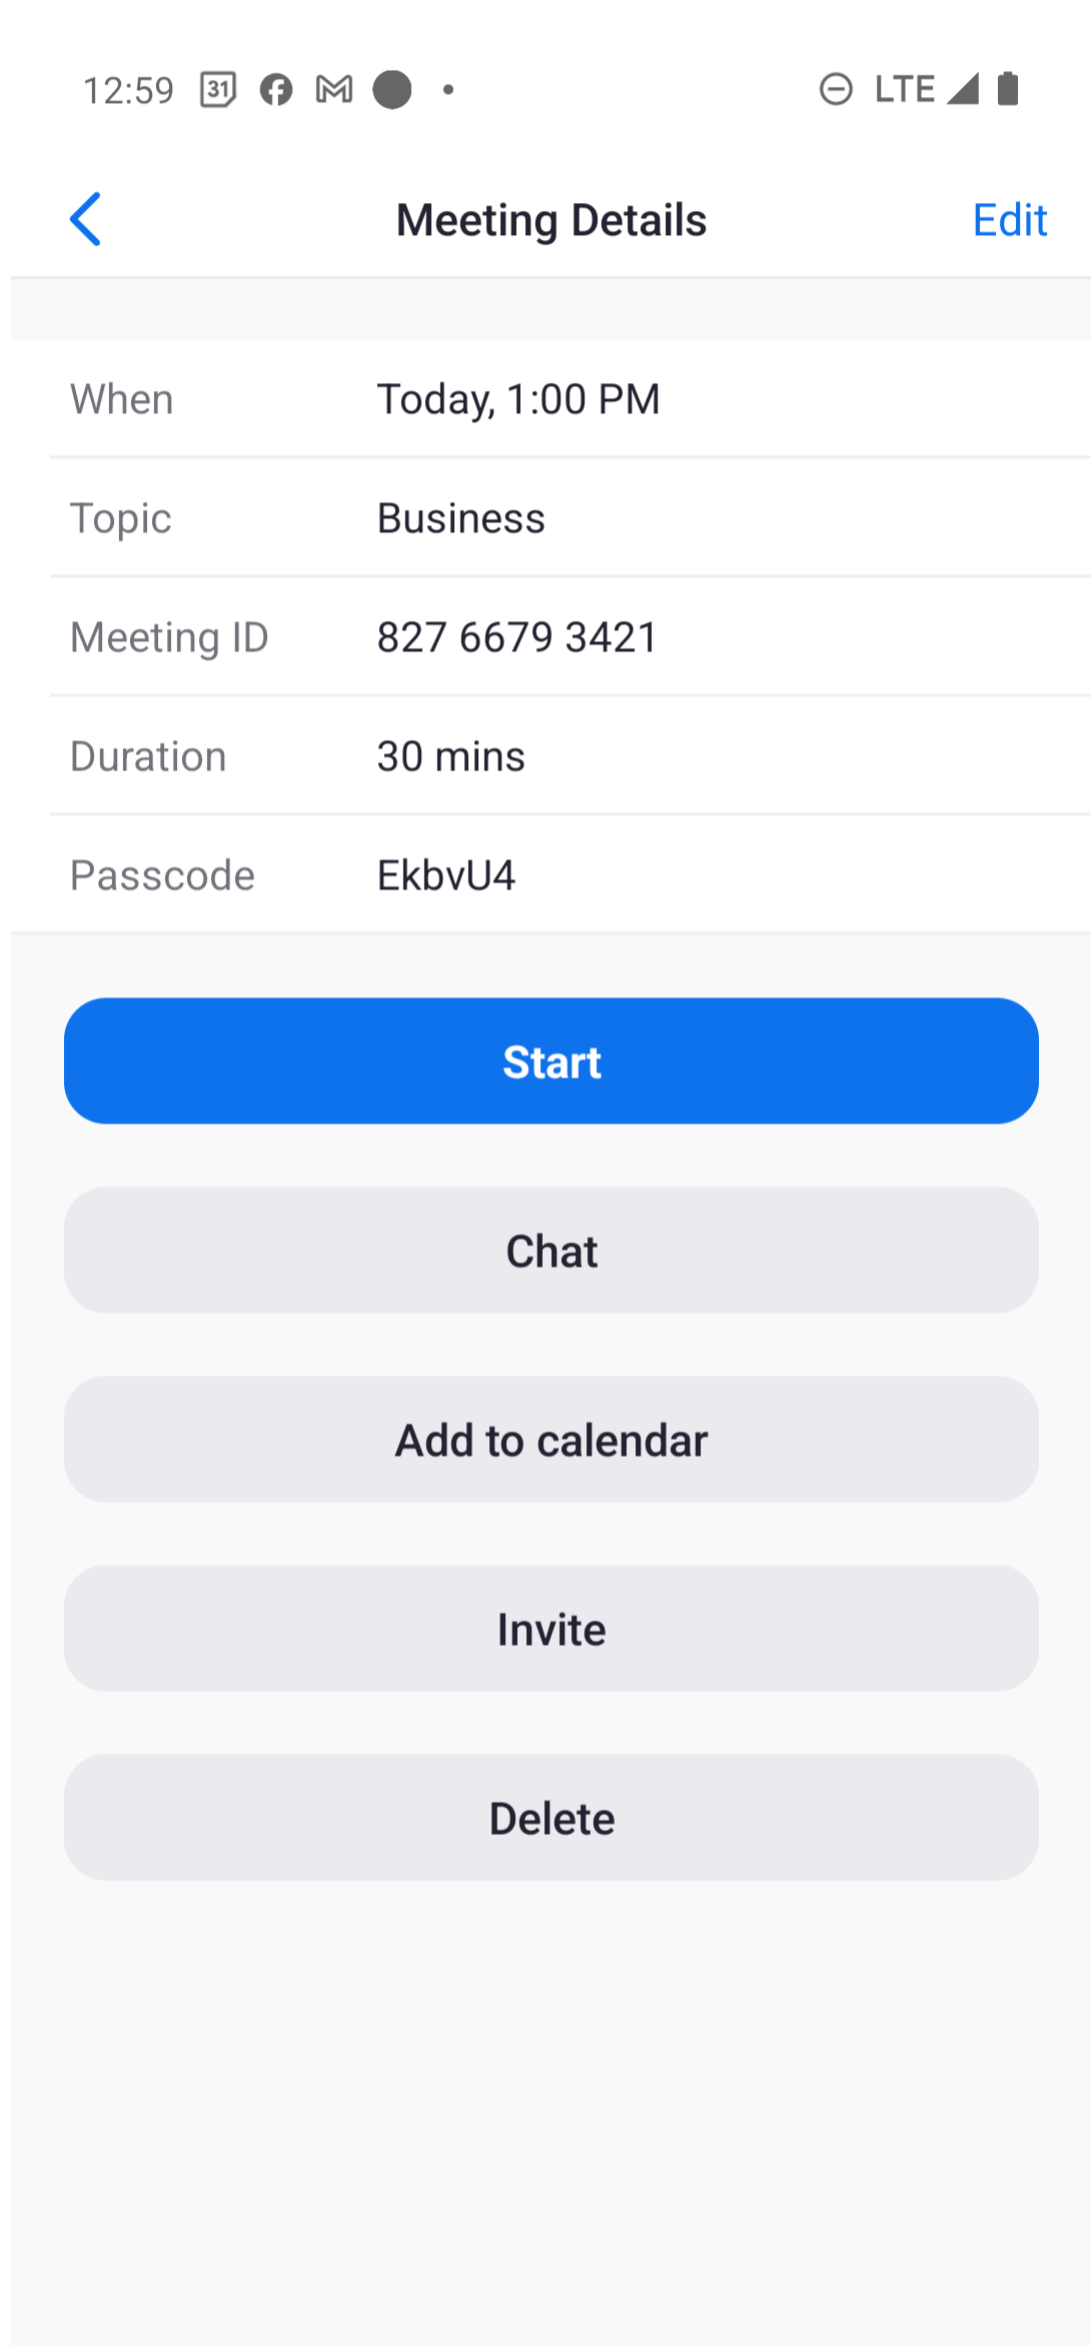

Step 10

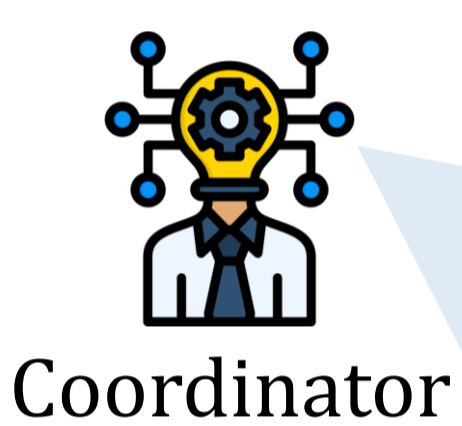

Coordinator

<think>I am pressing the home button to exit the Zoom app and proceed to the next steps of the task. By doing this, I can open the Tumblr app to send out the meeting invitations and then set an alarm using the Clock app. This ensures that I efficiently manage my time and complete all necessary preparations for the meeting. </think>  
<answer>**Return to the home screen.**</answer>

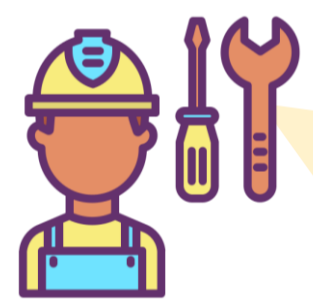

Executor

<think> The user wants to return to the home screen. The current screen shows a Zoom meeting details page showing the meeting time, topic, ID, duration, and passcode, with options to start, chat, add to calendar, invite, or delete the meeting. I should directly return home. </think>  
<answer>**PRESS\_HOME**</answer>

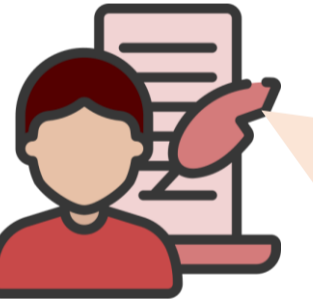

State Tracker

The business meeting with saltyfunsweets has been scheduled using the Zoom app, with the meeting details confirmed and saved. The meeting information has been copied to the clipboard in preparation for sharing via Tumblr.

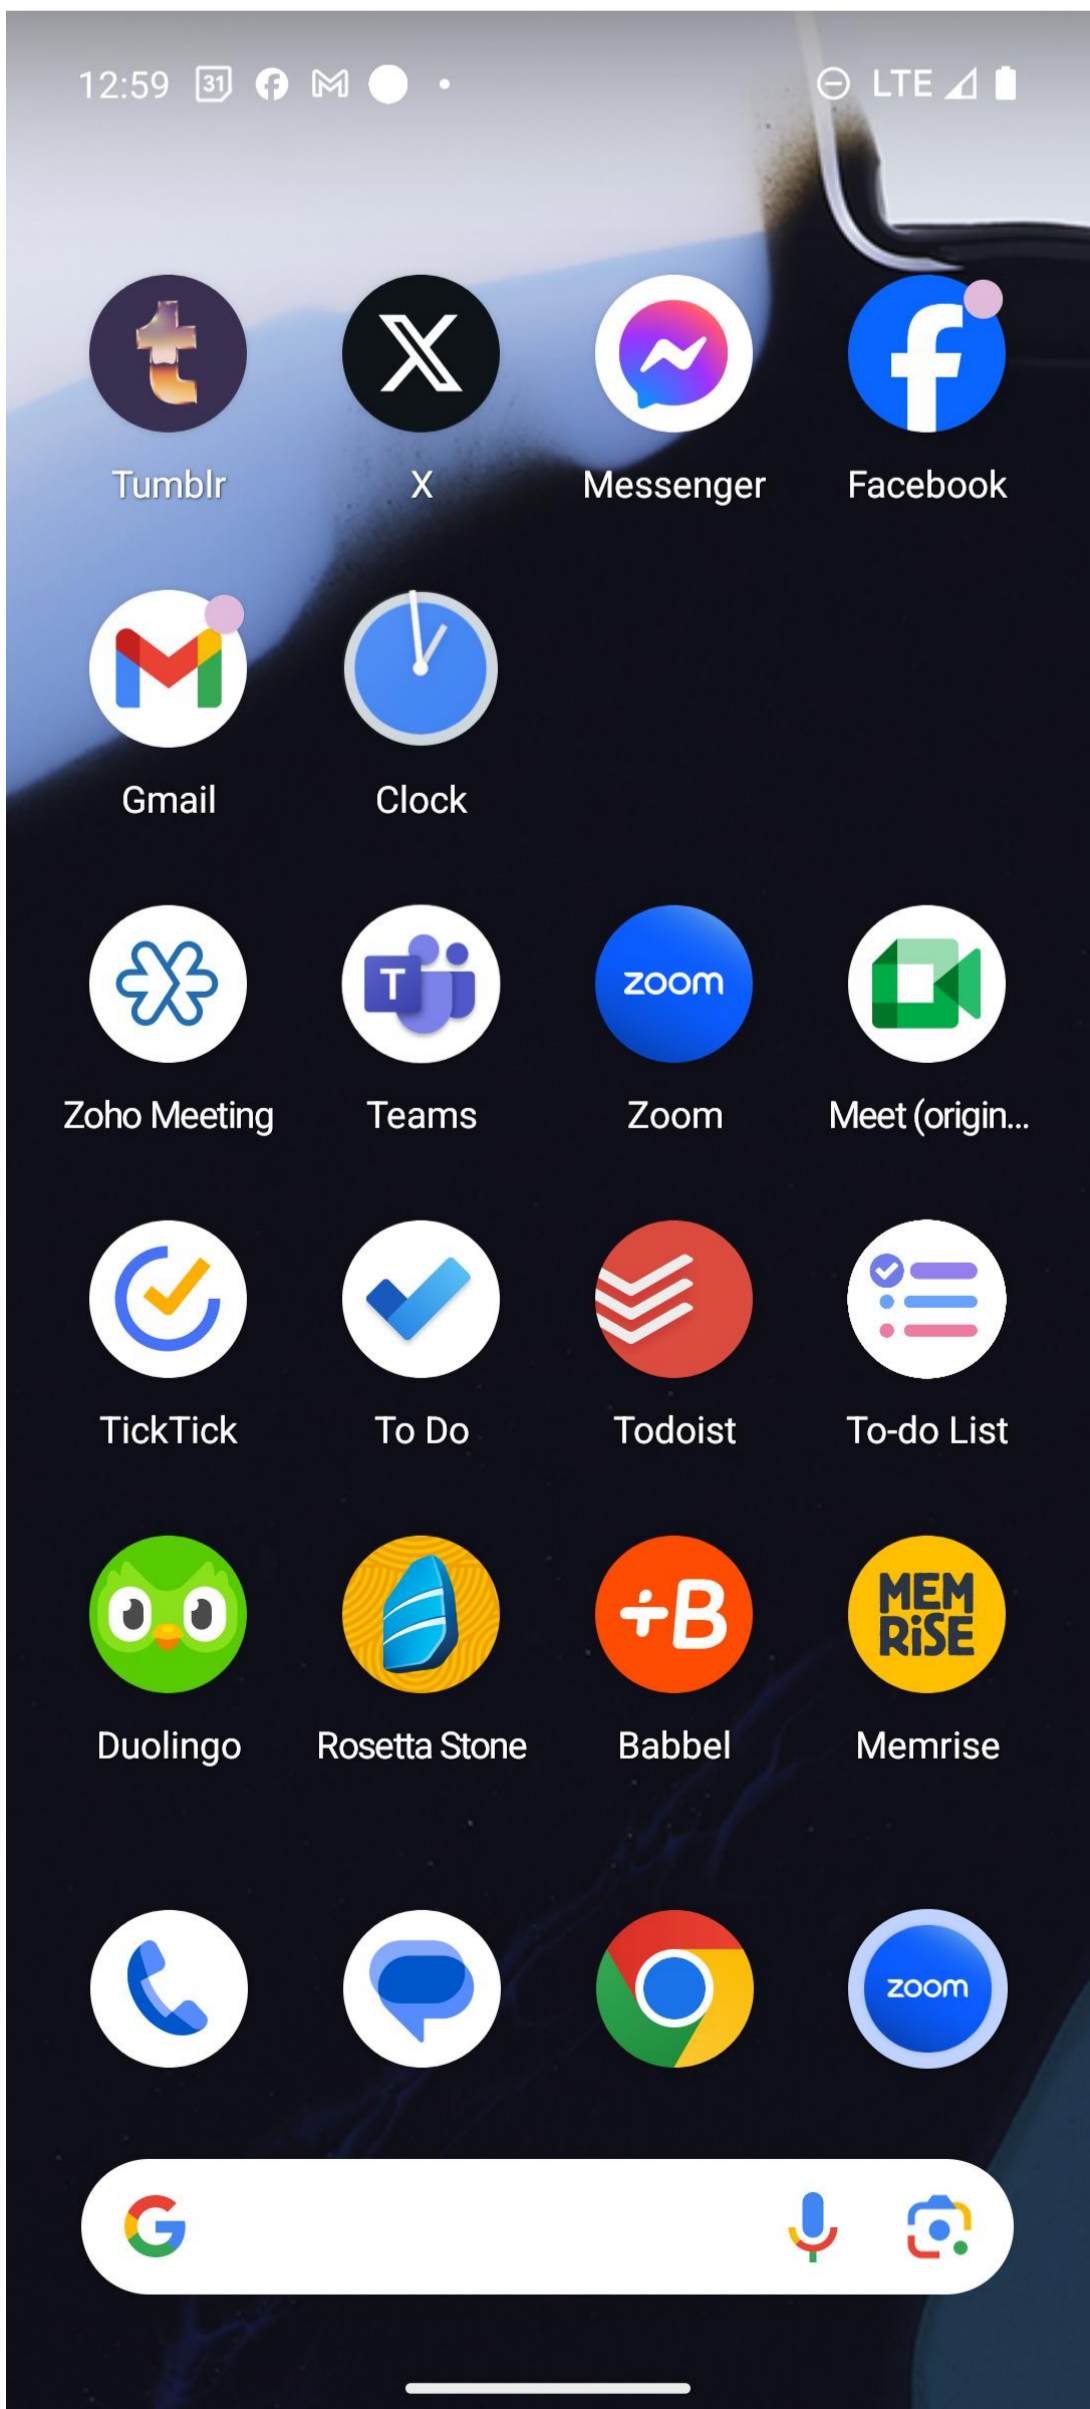

Step 11

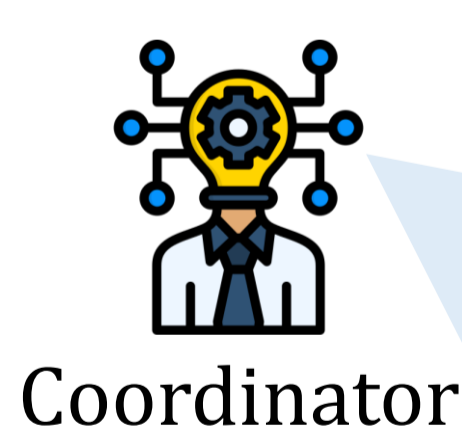

Coordinator

<think>I am opening the Tumblr app to send out the meeting invitations for the business meeting with saltyfunsweets. This action is appropriate because I have already copied the meeting link and now need to use Tumblr to distribute the invitations. By opening Tumblr, I can paste the link and send it to the intended recipients, ensuring they receive the meeting details promptly.</think>  
<answer>**Open the Tumblr app.**</answer>

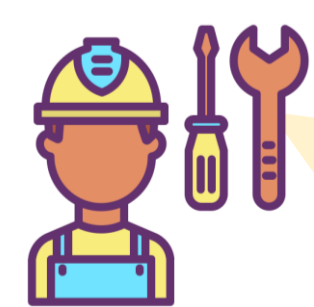

Executor

<think>The user wants to open the Tumblr app to send out meeting invitations. The Tumblr app icon is visible on the screen, and the next step is to click on it to open the app.</think>\n<answer>**CLICK: (161, 357)**</answer>

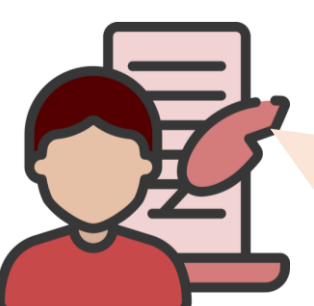

State Tracker

The Zoom app has been used to schedule a business meeting with saltyfunsweets, and the meeting details have been saved. The meeting details are copied to the clipboard in preparation for sharing on Tumblr, and the Tumblr app has been accessed to proceed with sending out the meeting invitations.

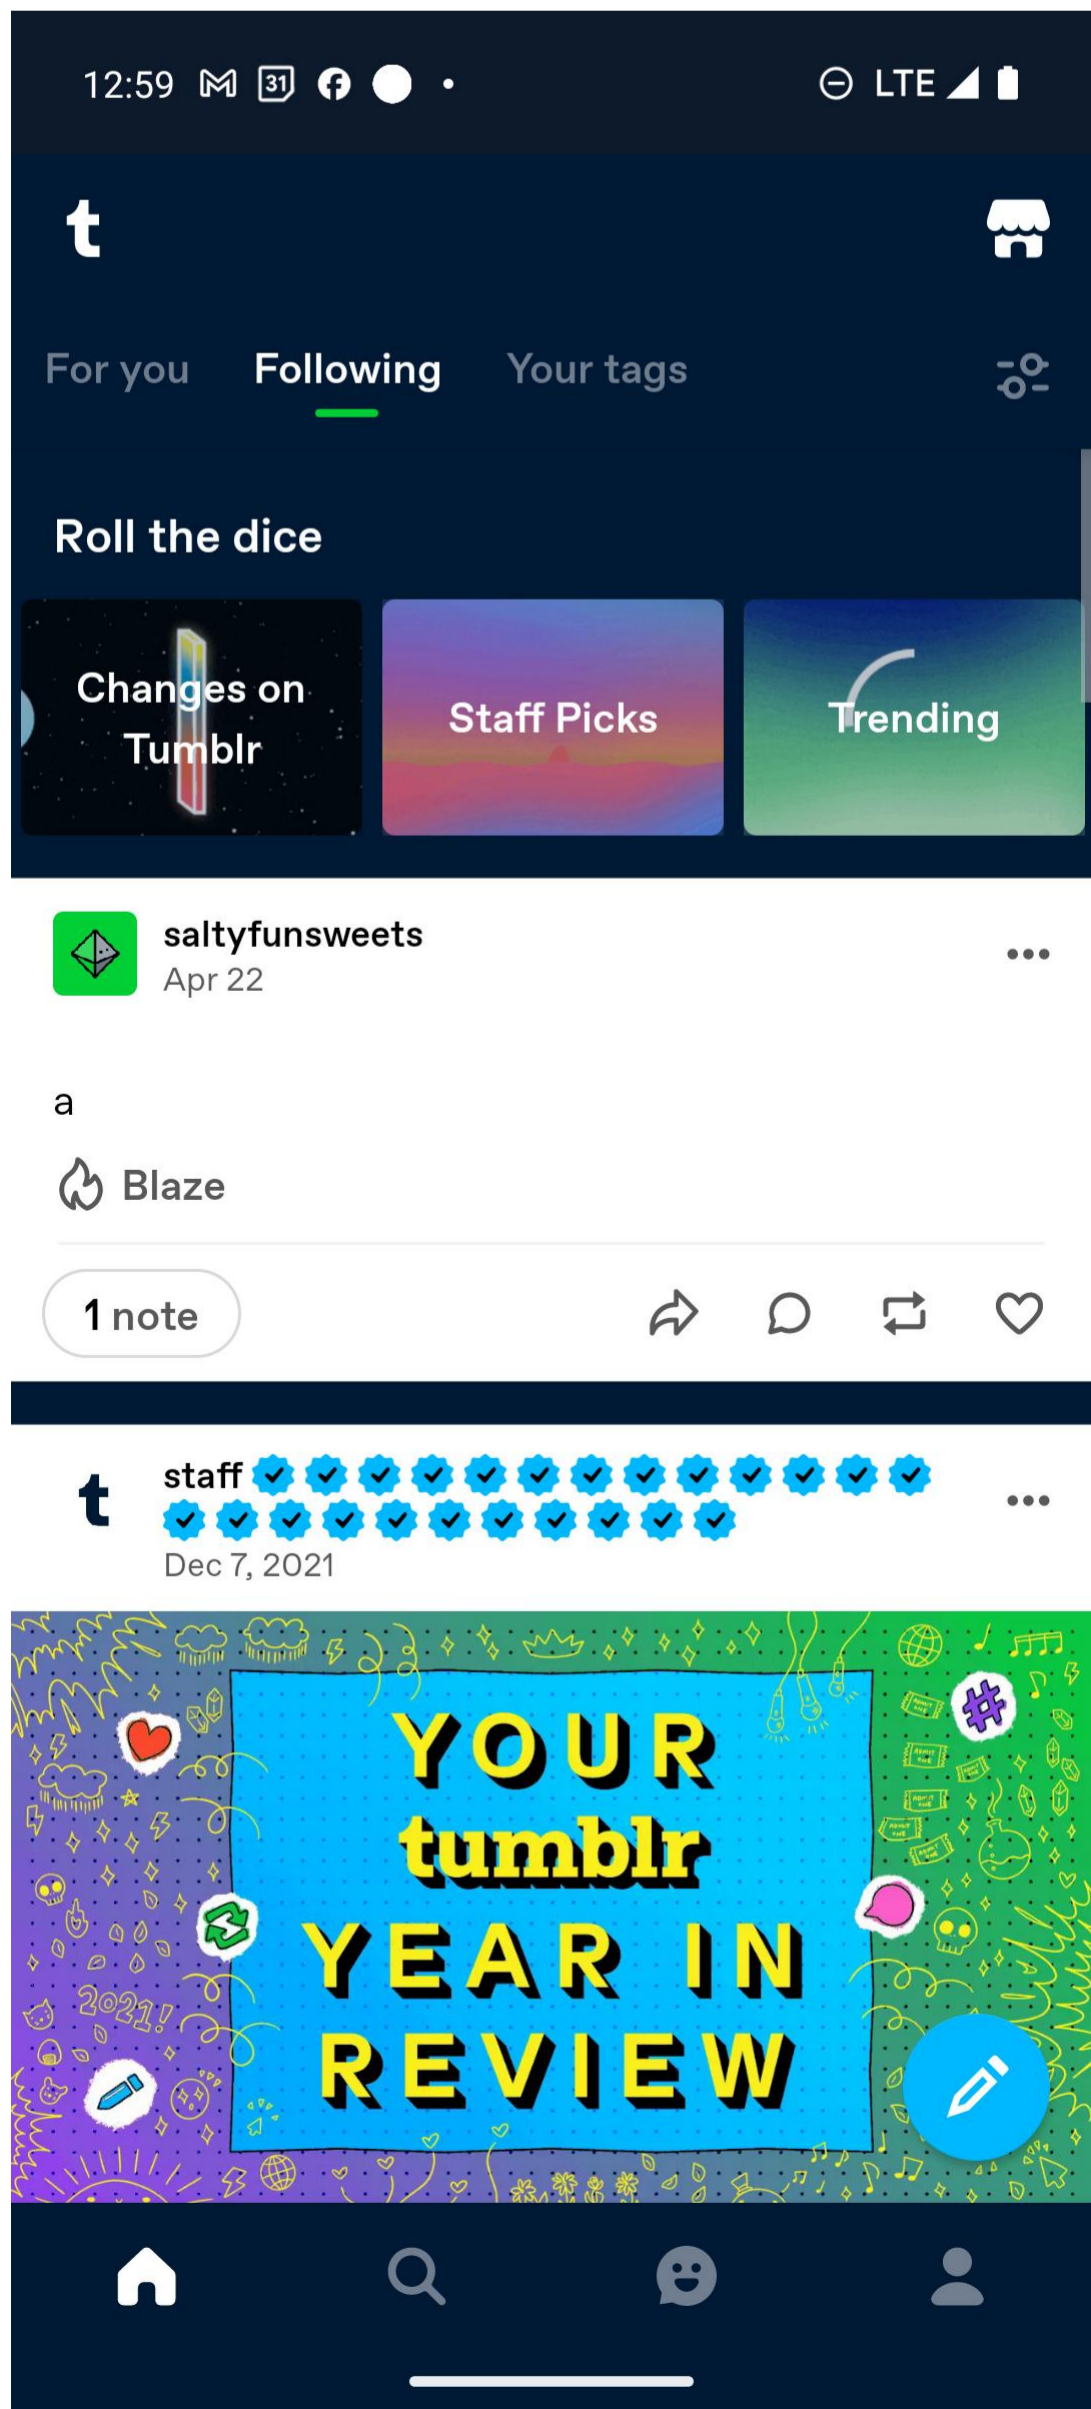

Step 12

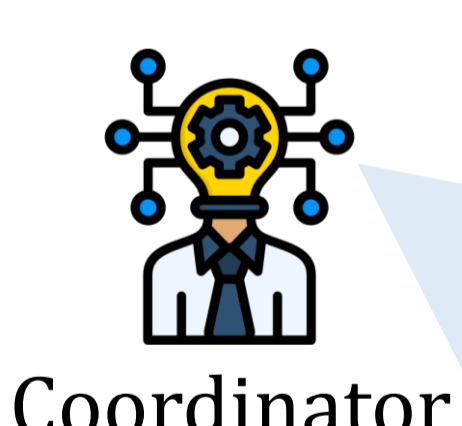

Coordinator

<think>This is a screenshot of the Tumblr app displaying the 'Following' feed, showing posts from users and options. The interface includes navigation icons at the bottom for different sections of the app. I am selecting the messaging icon to access the direct messages section of Tumblr. </think>  
<answer>**Open the messaging section.**</answer>

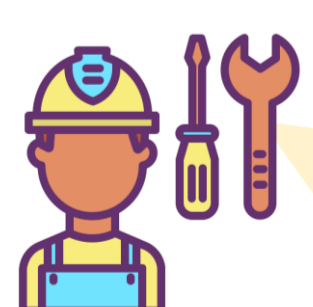

Executor

<think>The user wants to open the messages section. The messages icon is typically represented by a bubble with an smiling face in the bottom of the screen. I need to click on this icon to proceed with sending out the meeting.</think>  
<answer>**CLICK: (671, 1305)**</answer>

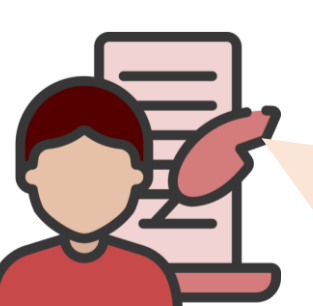

State Tracker

The business meeting with saltyfunsweets has been scheduled using the Zoom app, and the meeting details have been saved. The meeting information was copied to the clipboard to facilitate sharing via Tumblr, and the Tumblr app was accessed to send out the meeting invitations through direct messages.

User Instruction

Organize a business meeting with saltyfunssweets using ZOOM Cloud Meetings, send out the meeting invitations via Tumblr, and set an alarm clock for the meeting time using the Clock app.

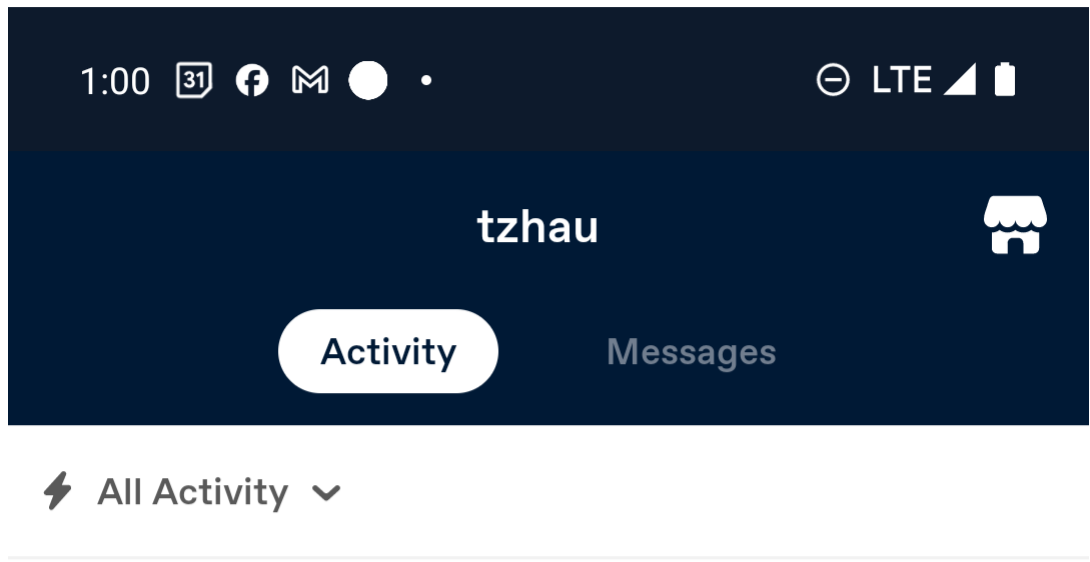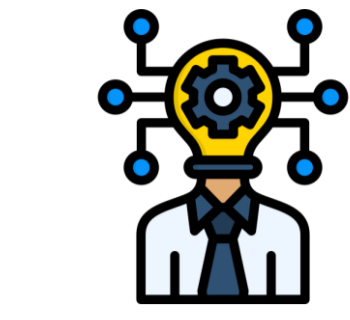

Coordinator

<think>This is a screenshot of the Tumblr app showing the user's profile page with options to view activity and messages. The screen prompts the user to create a post. I am choosing to click on the 'Messages' tab to proceed with sending out meeting invitations. This action is appropriate as it allows me to access the messaging section where I can send the meeting details to the intended recipients.</think>  
<answer>Go to the messages section. </answer>

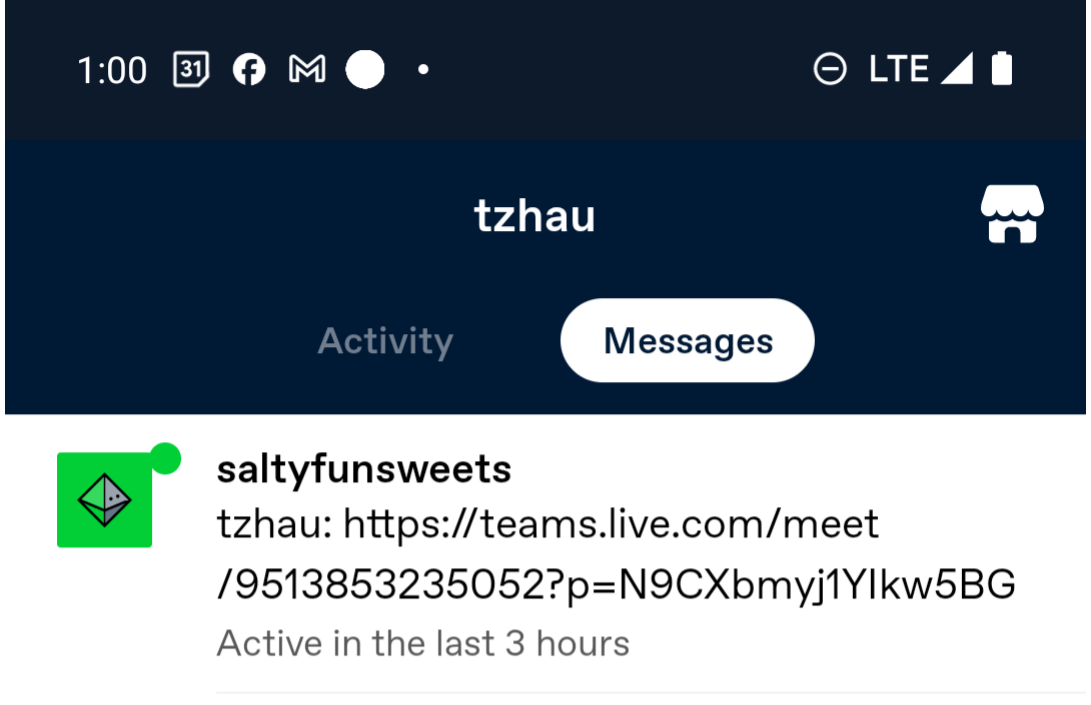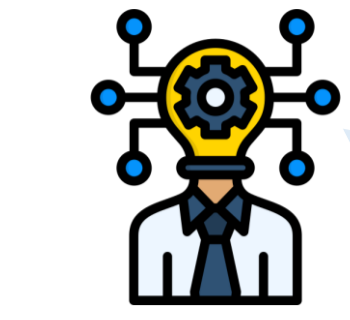

Coordinator

<think>This is a screenshot of a Tumblr messages screen showing a conversation with 'saltyfunssweets' containing a meeting link. The interface displays the message details and the user's activity status.I am selecting the message to view or edit the content, possibly to send additional information or confirm the meeting details. This action is appropriate as it allows me to ensure the meeting invitation is correctly communicated before proceeding to set an alarm.</think>  
<answer>Open the message to view or edit its content. </answer>

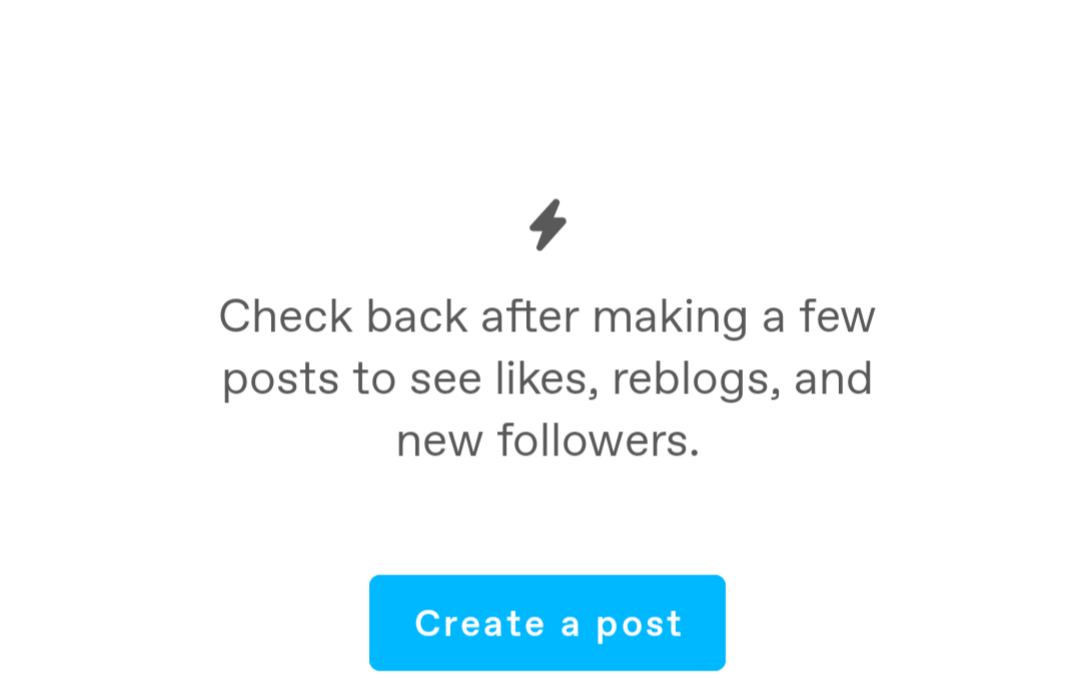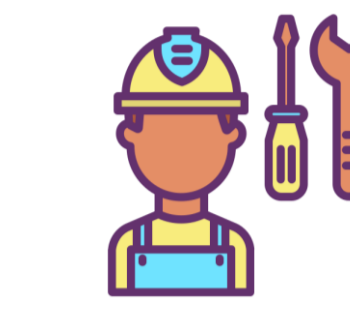

Executor

<think>The user wants to navigate to the messages section. The 'Messages' tab is clearly visible at the top of the screen, indicating it is the target for the user's action.</think>  
<answer>CLICK: (690, 344)</answer>

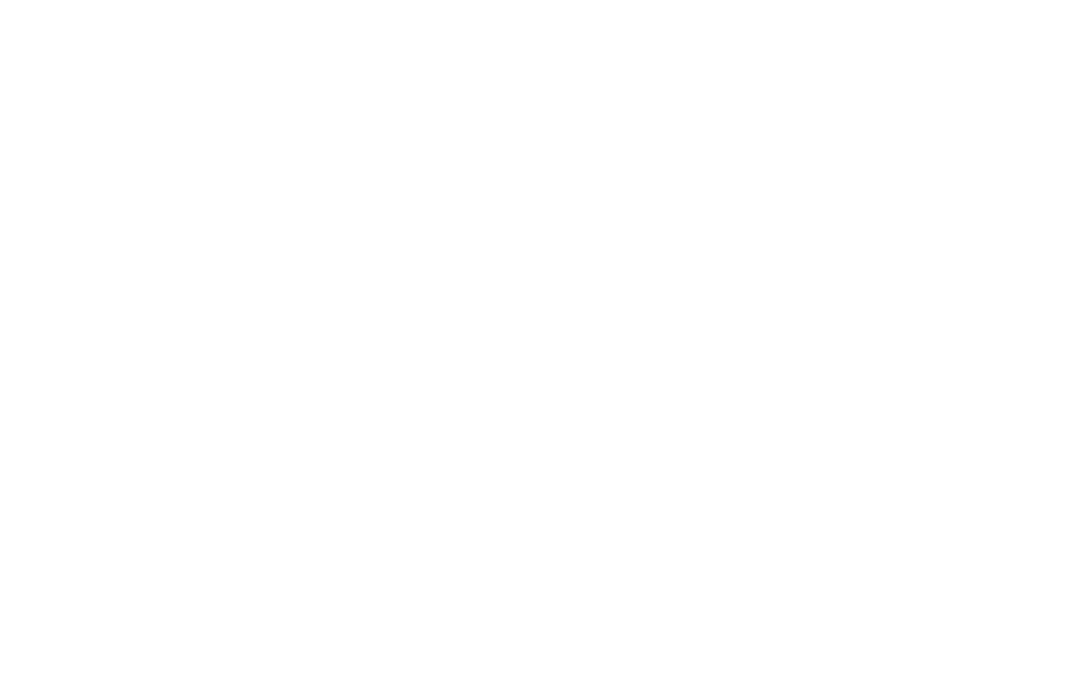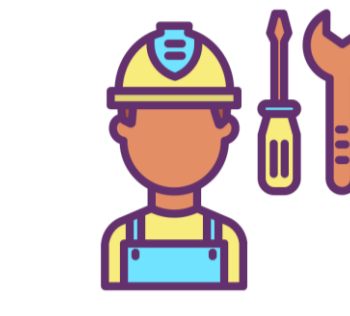

Executor

<think>The user wants to view or edit the content of a message. The message from 'saltyfunssweets' is visible, and it seems to be the one the user wants to interact with. To achieve the goal, I need to click on this message to open it and view or edit its content.</think>  
<answer>CLICK: (376, 473)</answer>

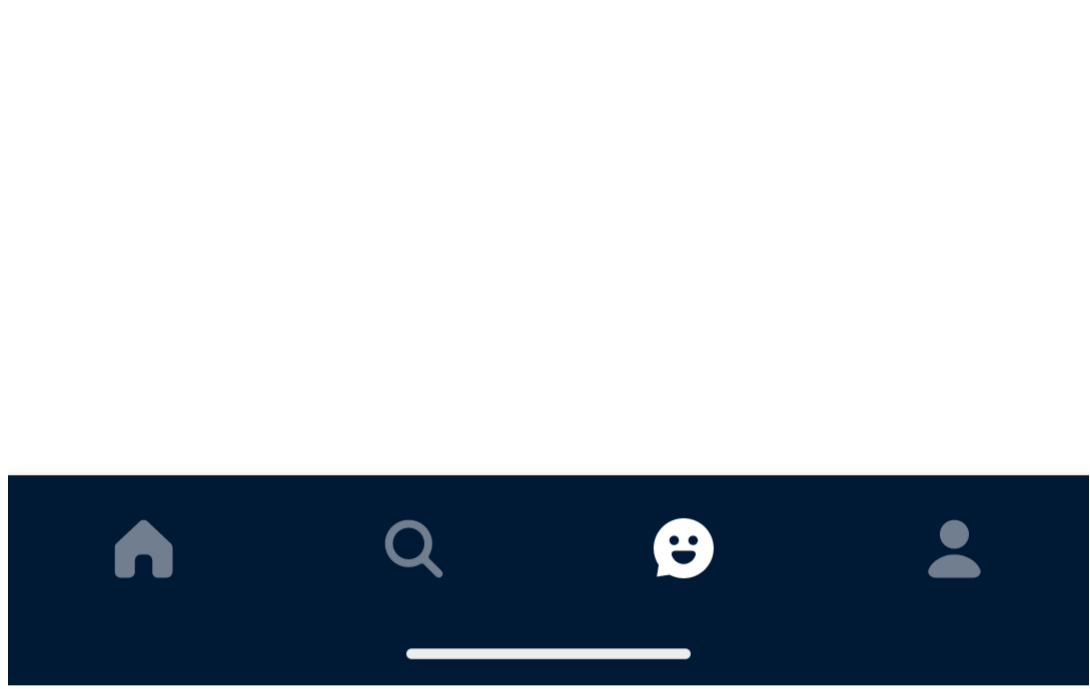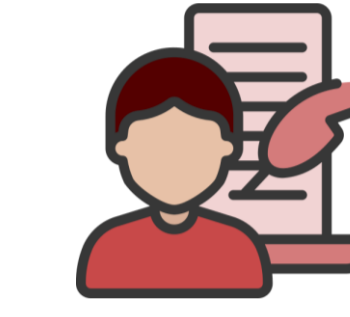

State Tracker

The business meeting with saltyfunssweets has been organized using the Zoom app, with the meeting details confirmed and saved. Invitations are being prepared to be sent out via Tumblr by accessing the messaging section to share the meeting information directly with recipients.

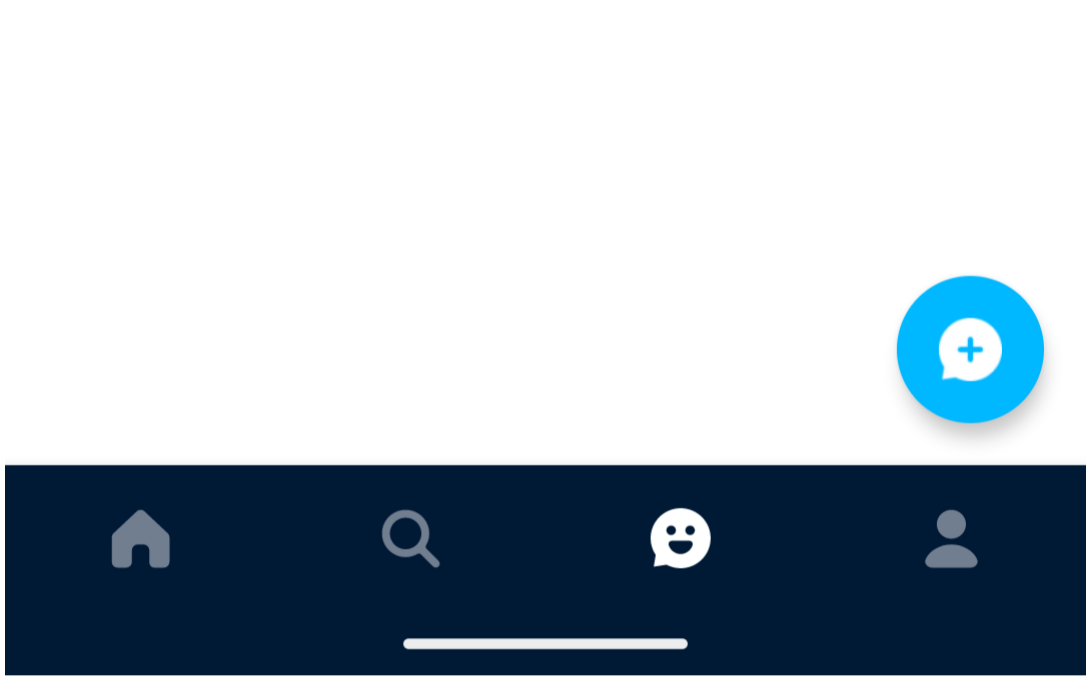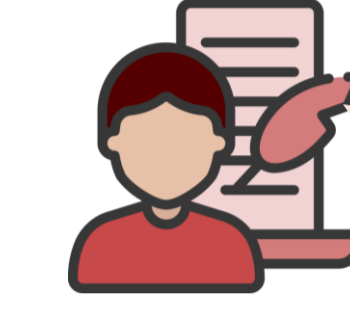

State Tracker

The business meeting with saltyfunssweets has been organized using the Zoom app, with the meeting details saved and ready for distribution. Invitations have been prepared by copying the meeting details to the clipboard, and the Tumblr app has been accessed to send out these invitations via direct messages, ensuring the information reaches the intended recipients.

Step 13

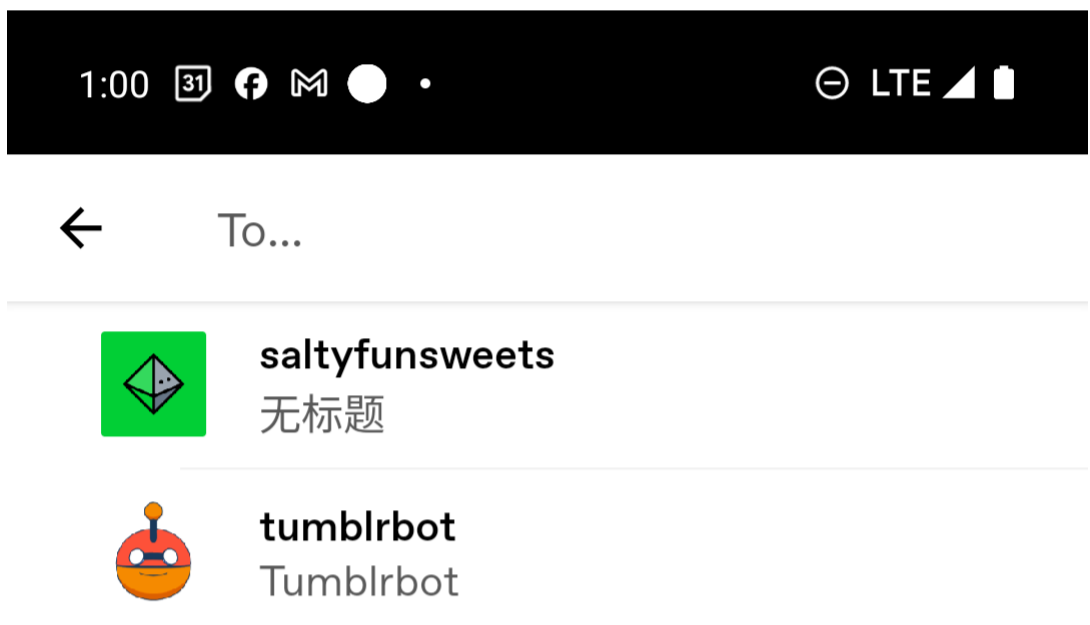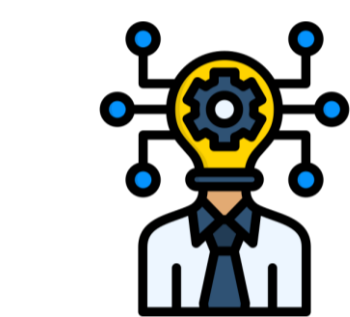

Coordinator

<think>This is a screenshot of a Tumblr app interface showing a list of contacts or messages. The user is in the process of selecting a contact to send a message or invitation.I am selecting the contact 'saltyfunssweets' to proceed with sending the meeting invitation. This action is necessary to ensure that the invitation is sent to the correct recipient, allowing me to organize the business meeting effectively.</think>  
<answer>Select the contact 'saltyfunssweets' to send a message.</answer>

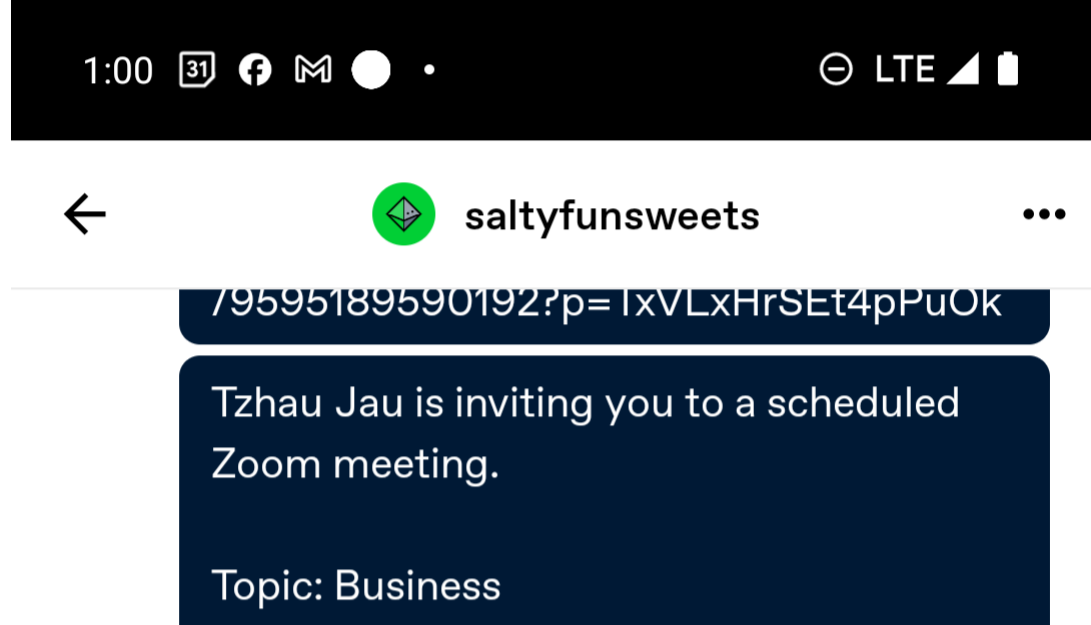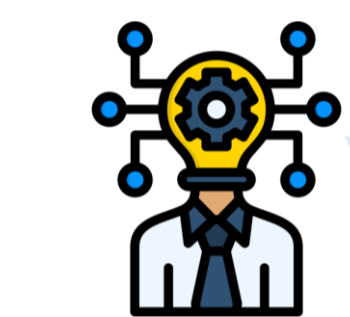

Coordinator

<think>This is a screenshot of a conversation in the Tumblr app with a contact named 'saltyfunssweets'. The message contains details about a scheduled Zoom meeting, including the topic, time, and meeting link.I am preparing to send a message to 'saltyfunssweets' to confirm the meeting details and ensure they have all the necessary information.</think>  
<answer>Tap on the message input field to start typing a message.</answer>

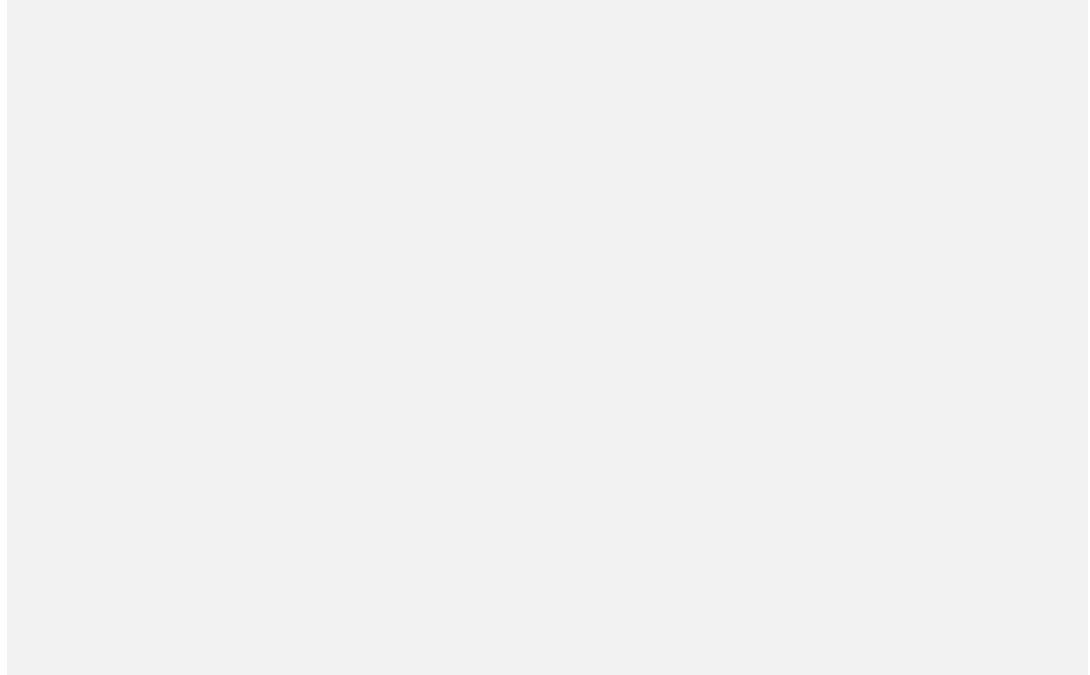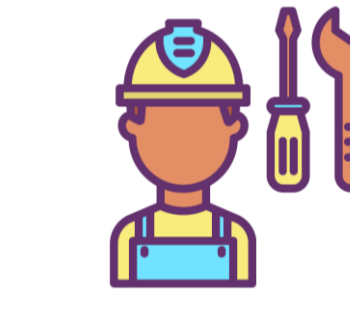

Executor

<think>The user wants to select the contact 'saltyfunssweets' to send a message. The contact is clearly visible in the list, and I need to click on it to proceed with the message composition process.</think>  
<answer>CLICK: (404, 344)</answer>

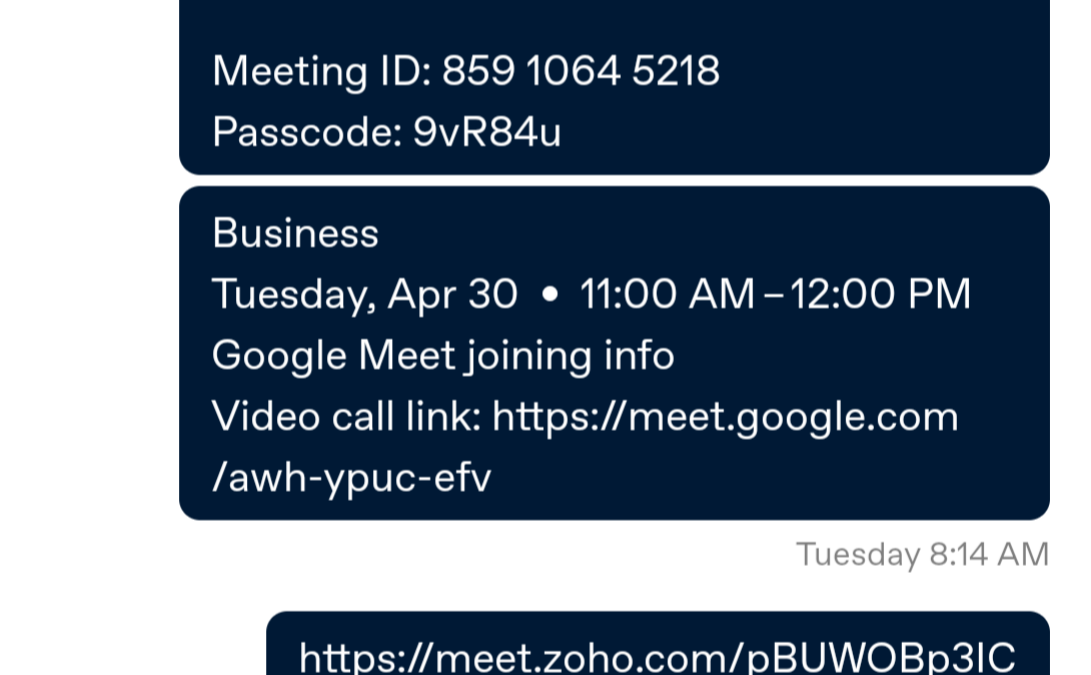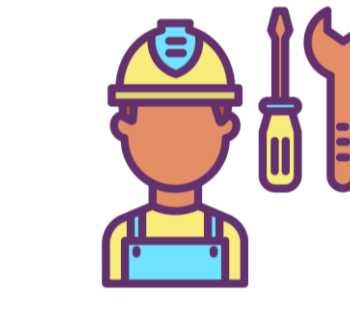

Executor

<think>The user wants to start typing a message in the chat. The message input field is located at the bottom of the screen, and it is the area where the user can type their message. The instruction is to tap on this field to activate it for typing.</think>  
<answer>CLICK: (380, 2156)</answer>

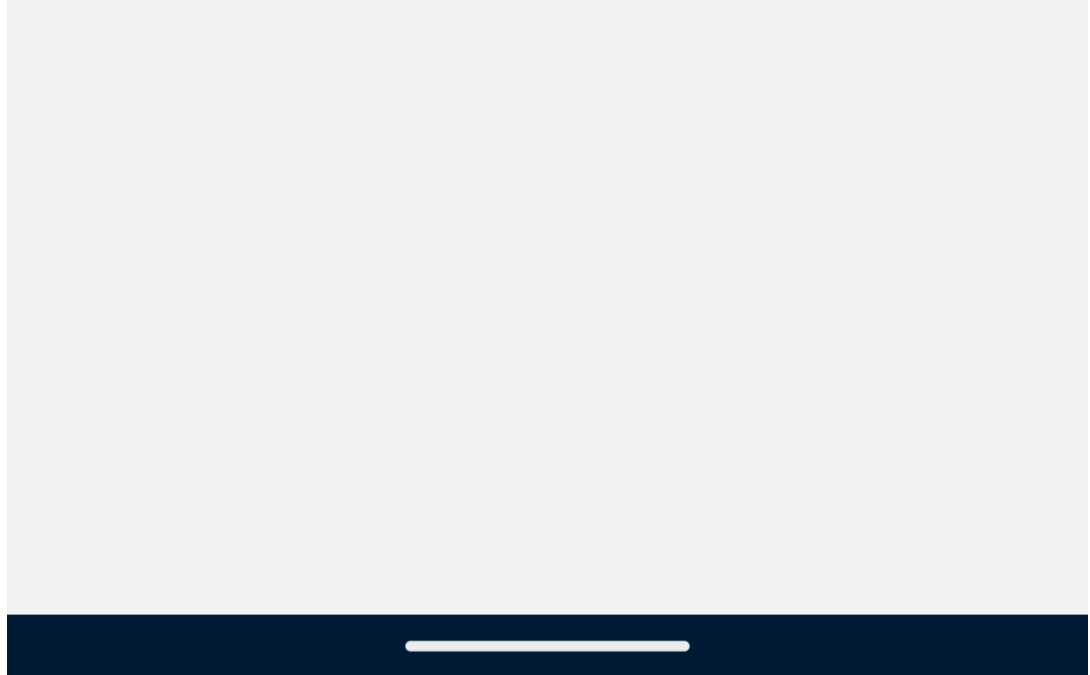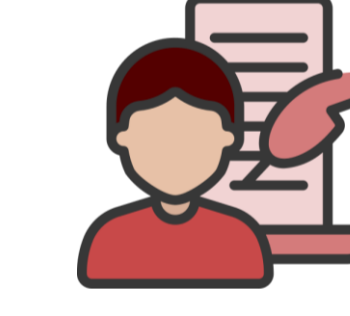

State Tracker

A business meeting has been scheduled using the Zoom app, and the meeting details have been saved. The invitation for the meeting has been sent to saltyfunssweets via direct message on Tumblr, ensuring the recipient receives the necessary information.

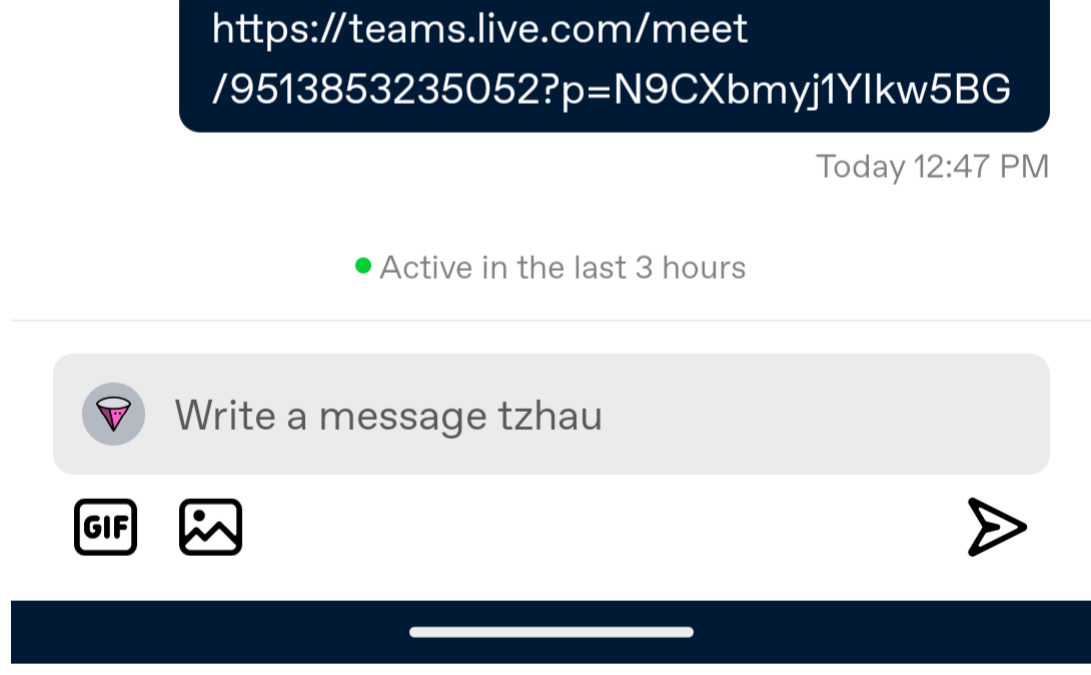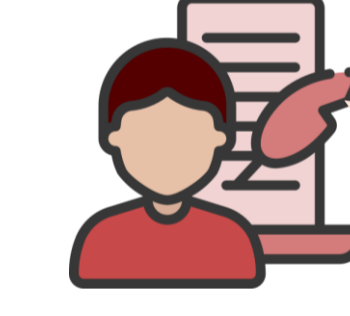

State Tracker

A business meeting with saltyfunssweets has been scheduled using Zoom, and the meeting details have been saved. Invitations have been sent out via direct message on Tumblr, ensuring the recipient has all necessary information for the meeting.

Step 15

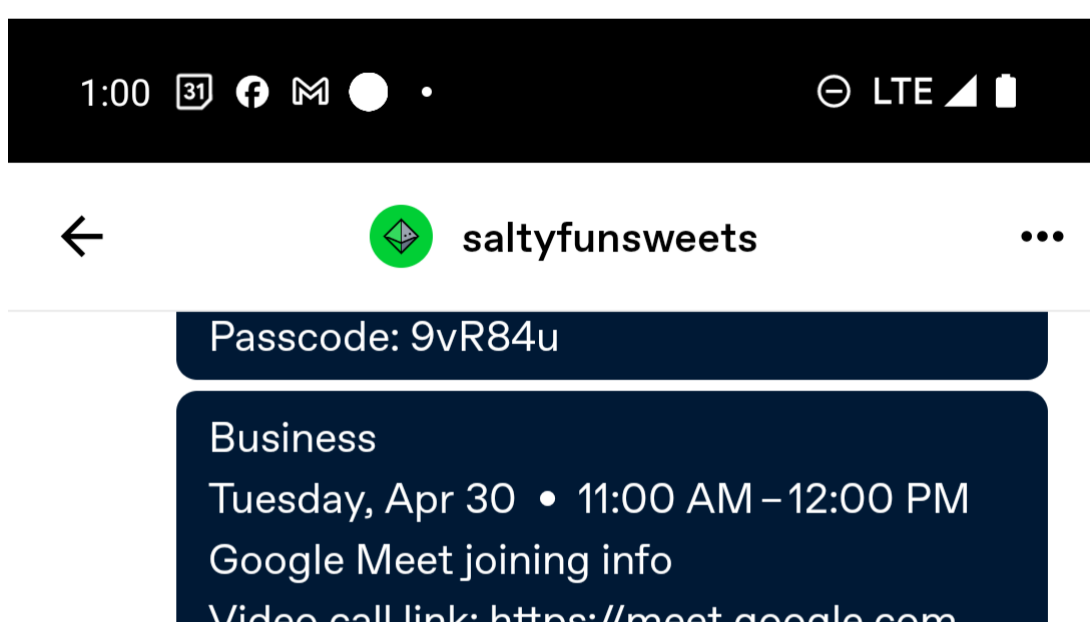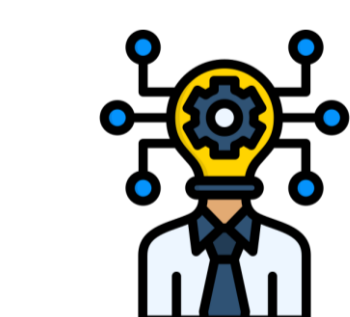

Coordinator

<think>I want to correct or complete the partially typed message in the input field to ensure clear communication with saltyfunssweets. By selecting the suggested text, I can quickly finalize my message, making the conversation more efficient and reducing the chance of errors. </think>  
<answer>Select suggested text to complete the message.</answer>

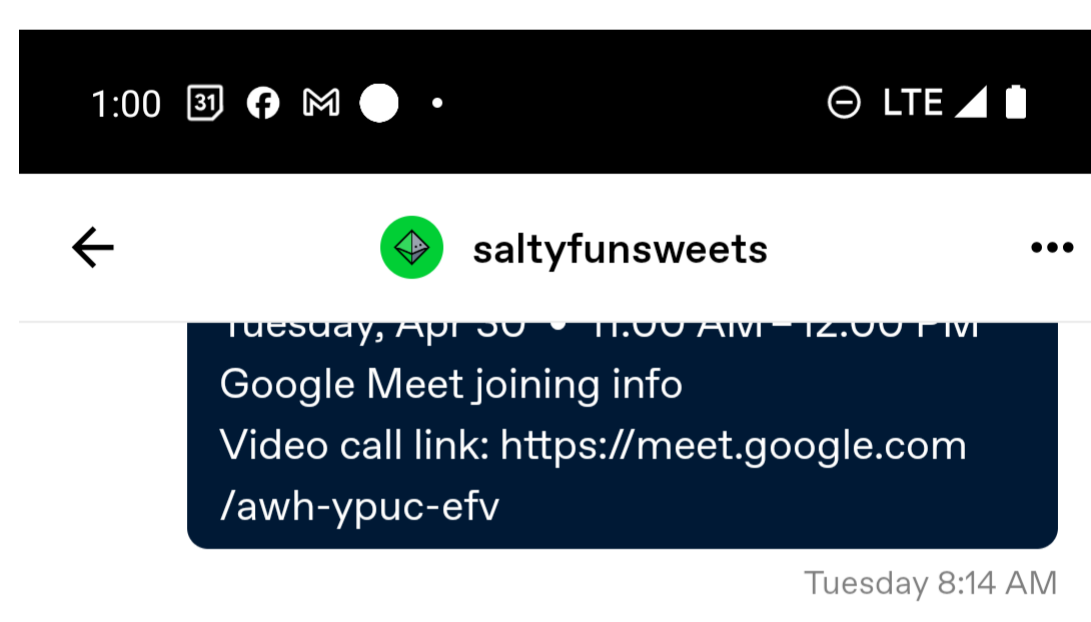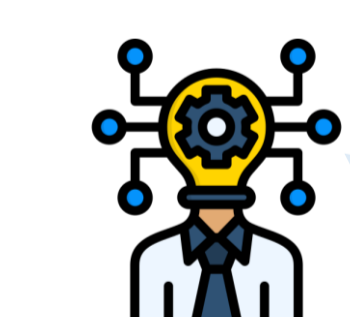

Coordinator

<think>This is a screenshot of a messaging app conversation with 'saltyfunssweets' where a meeting ID and passcode are being shared. The user is preparing to send this information to complete the task of organizing a business meeting.I am sending the meeting details to 'saltyfunssweets' to ensure they have all the necessary information to join the meeting. </think>  
<answer>Send the message containing the meeting details.</answer>

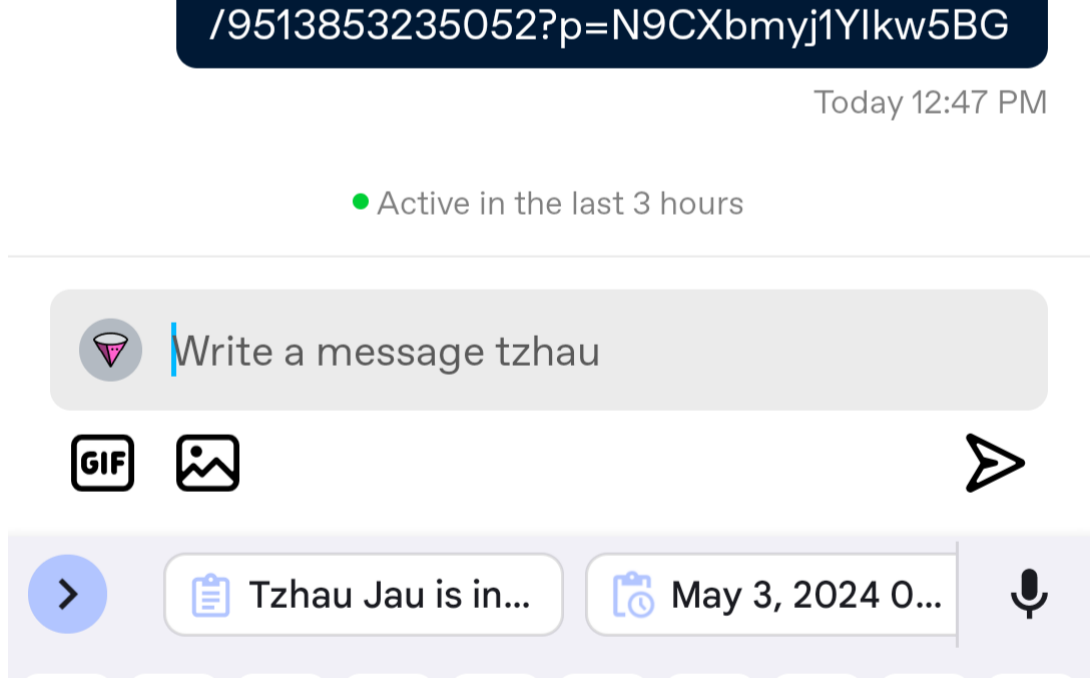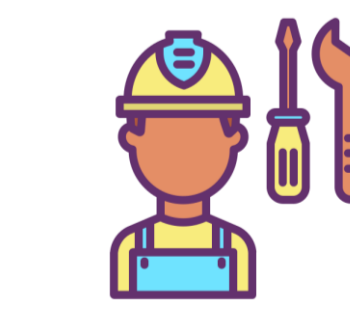

Executor

<think>The user wants to Select suggested text. The screen shows details of a scheduled business meeting with links to various video call platforms. The message input field is active with a partially typed message, and suggestions are displayed above the keyboard.</think>  
<answer>CLICK: (326, 655)</answer>

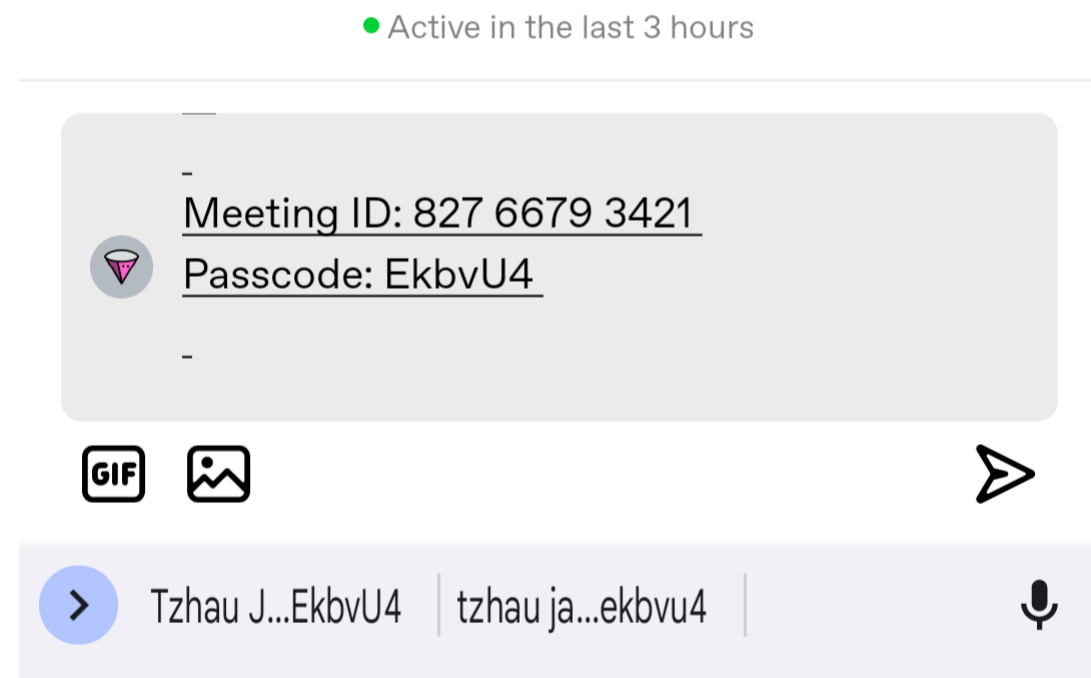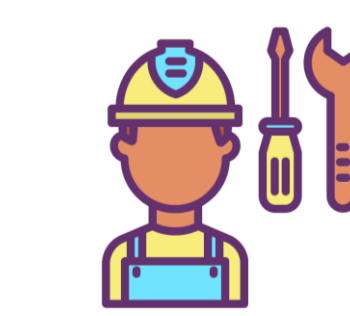

Executor

<think>The user wants to send a message containing the meeting details. The message is already typed in the input field, and the send button is visible. The next step is to click the send button to send the message.</think>  
<answer>CLICK: (994, 1446)</answer>

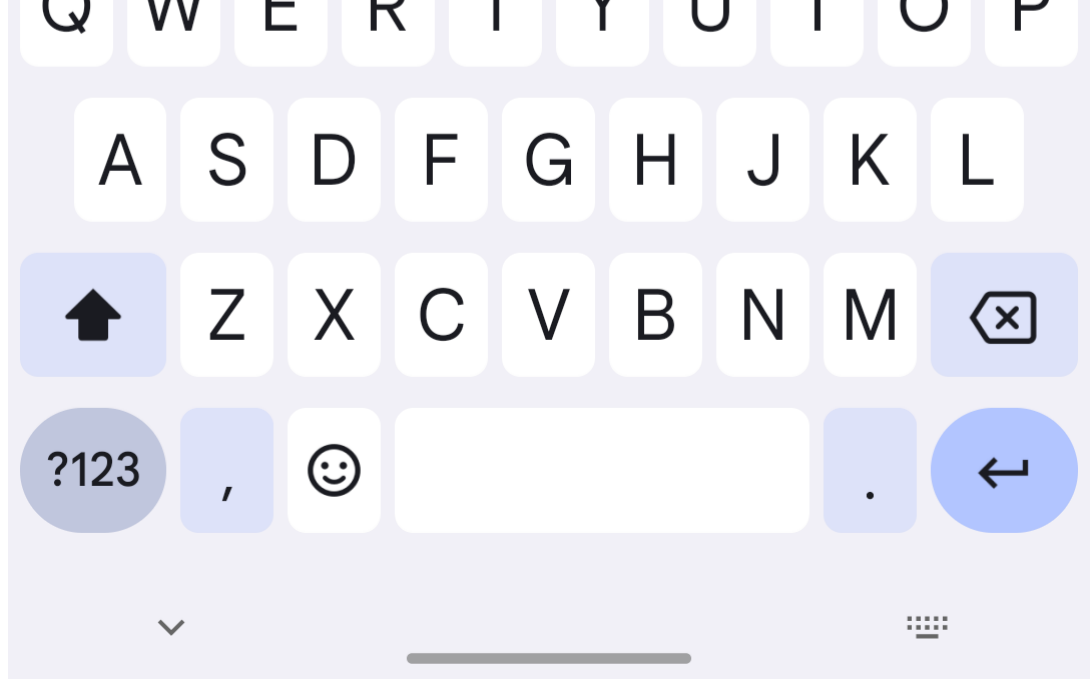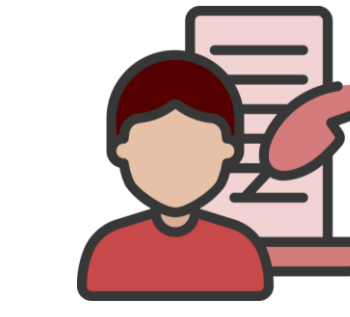

State Tracker

A business meeting with saltyfunssweets has been organized using the Zoom app, with the meeting details scheduled and saved. Invitations have been sent out via Tumblr's direct messaging feature to ensure the recipient receives the necessary information. The process of setting a reminder for the meeting is in progress, with the message input field selected for further action.

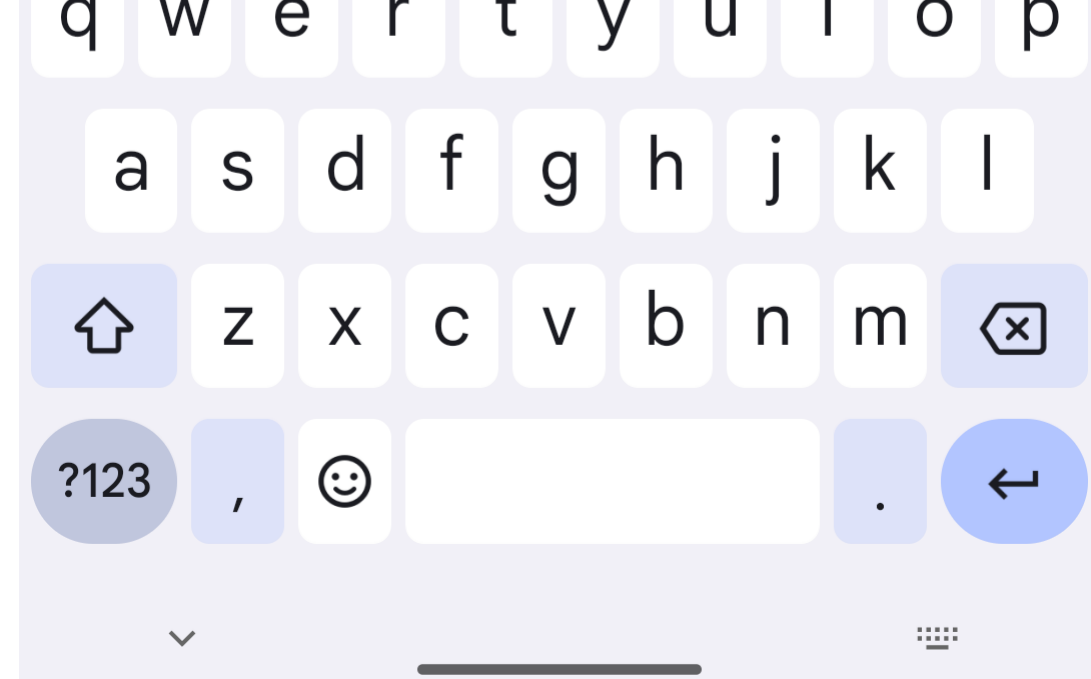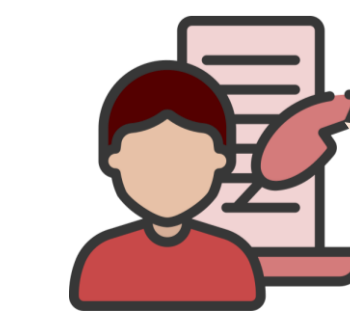

State Tracker

A business meeting has been organized using the Zoom app, with the meeting details confirmed and saved. Invitations have been sent to saltyfunssweets via direct message on Tumblr, ensuring the recipient has the necessary information to join the meeting.

Step 17

Step 18

User Instruction

Organize a business meeting with saltyfunssweets using ZOOM Cloud Meetings, send out the meeting invitations via Tumblr, and set an alarm clock for the meeting time using the Clock app.

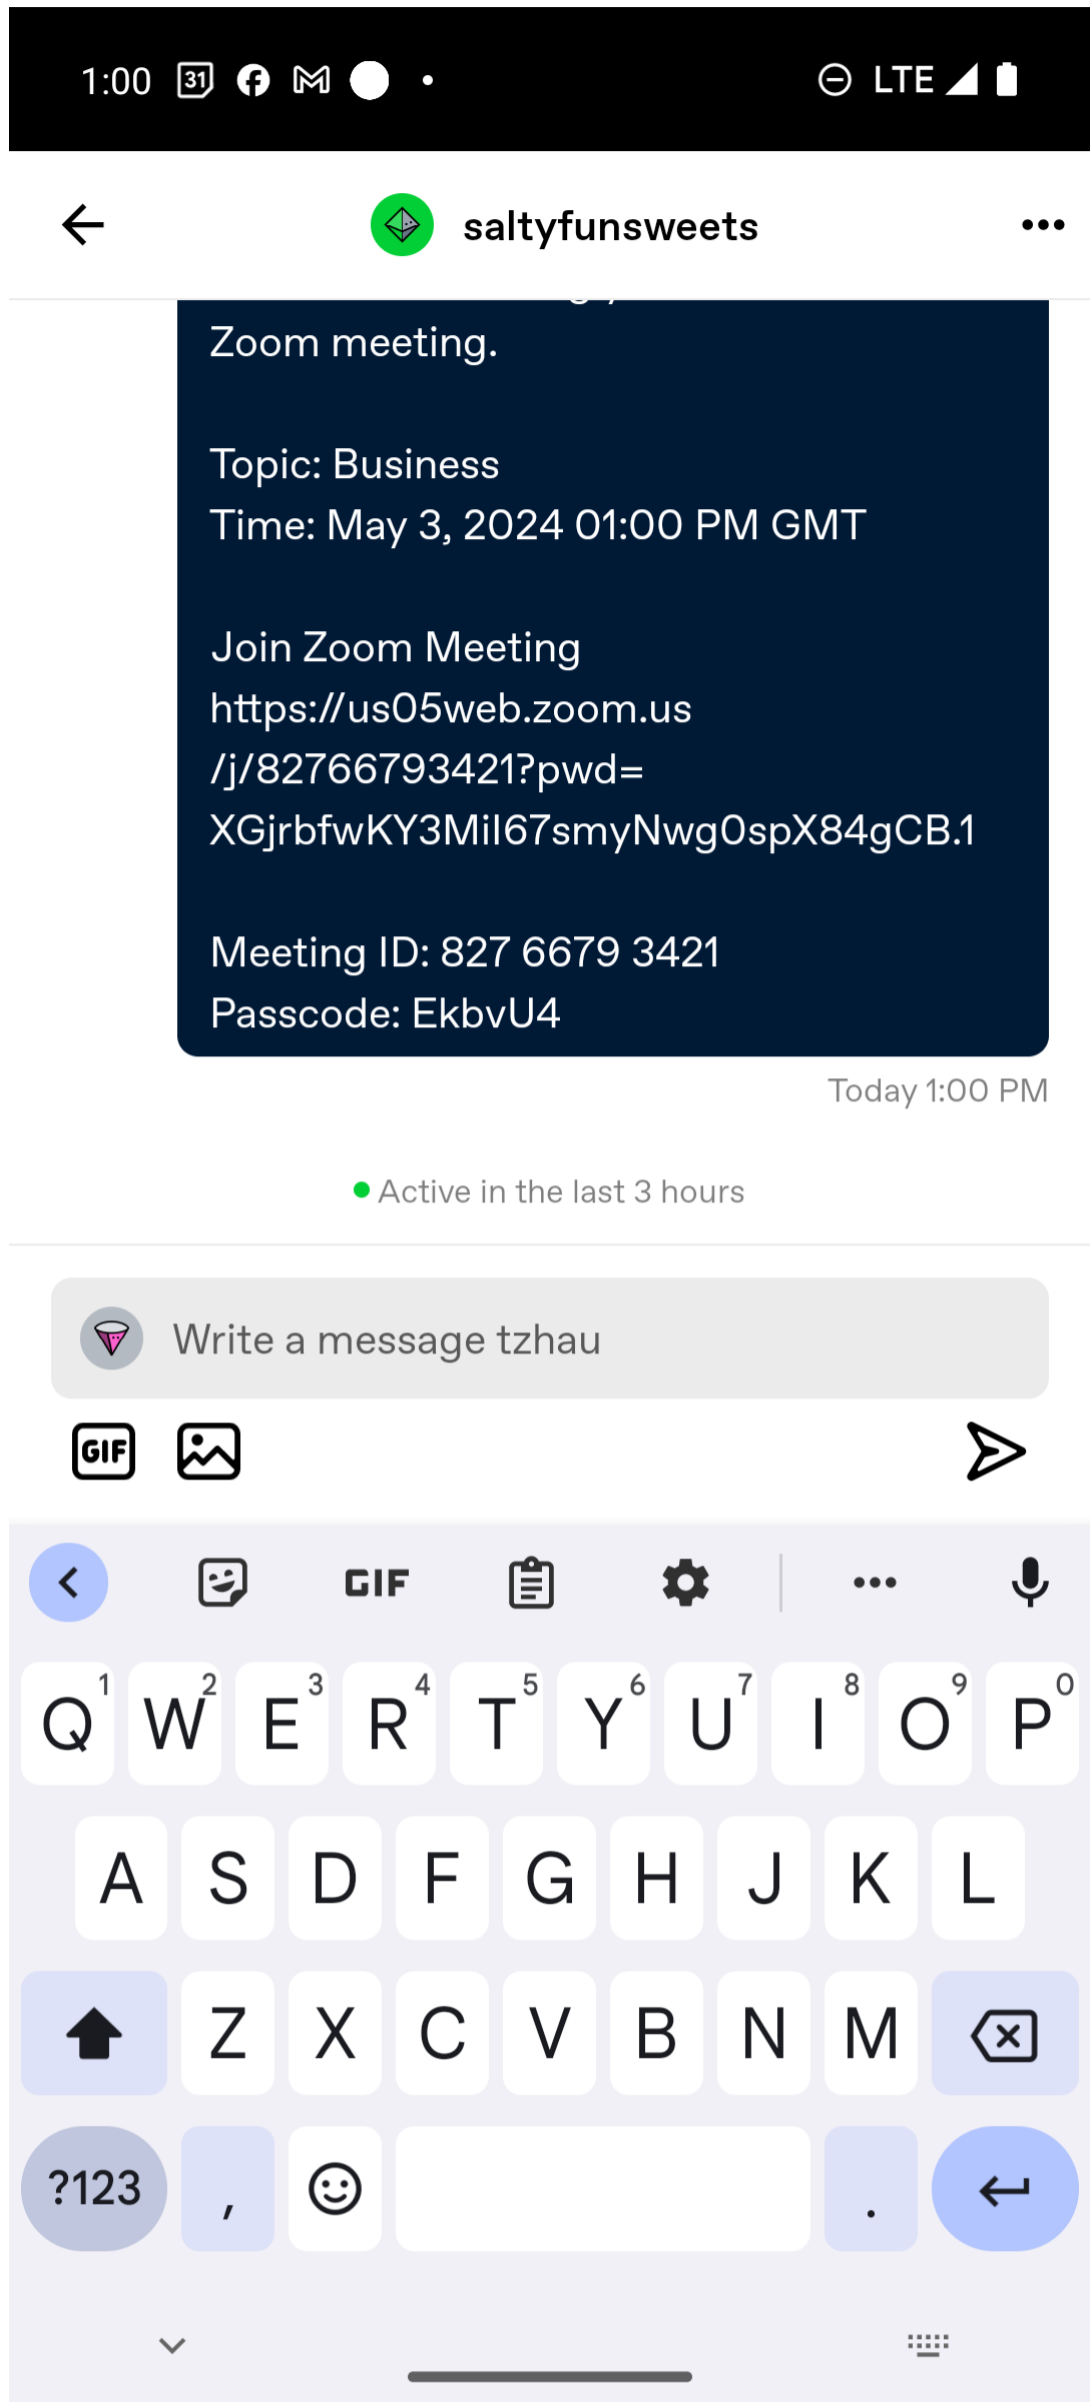

Step 19

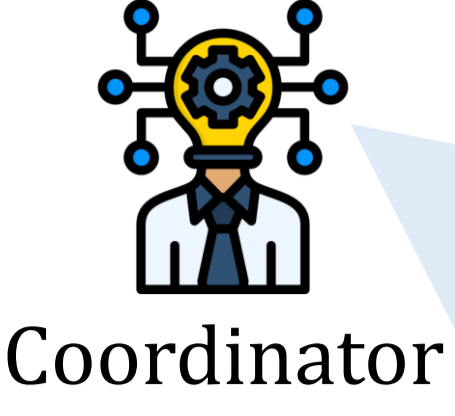

<think>This is a screenshot of a messaging app displaying a Zoom meeting invitation sent to 'saltyfunssweets'. The message includes the meeting topic, time, and details such as the Zoom link and passcode.I am pressing the home button to exit the messaging app and proceed to the Clock app. This action is necessary to set an alarm for the meeting time, ensuring I am reminded of the meeting at the specified time.</think>  
<answer>Return to the home screen.</answer>

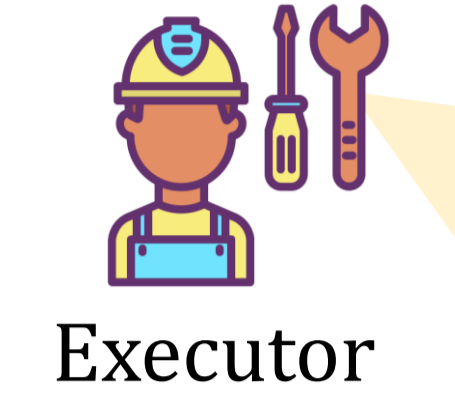

<think>The user wants to return to the home screen. The current screen is a messaging app, and there is no direct button to return to the home screen visible on the screen. The most likely way to return to the home screen is by pressing the home button on the device.</think>  
<answer>PRESS\_HOME</answer>

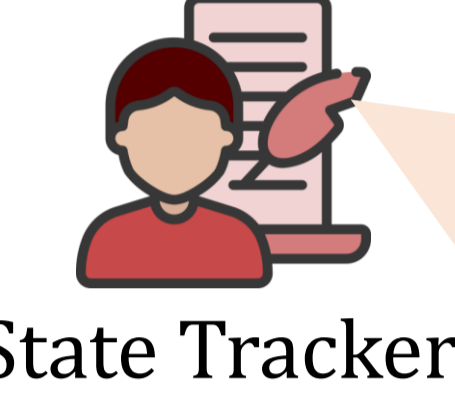

The business meeting with saltyfunssweets has been organized using the Zoom app, with the meeting details copied and sent via Tumblr direct messages. The invitation has been successfully communicated, ensuring the recipient has the necessary information to join the meeting.

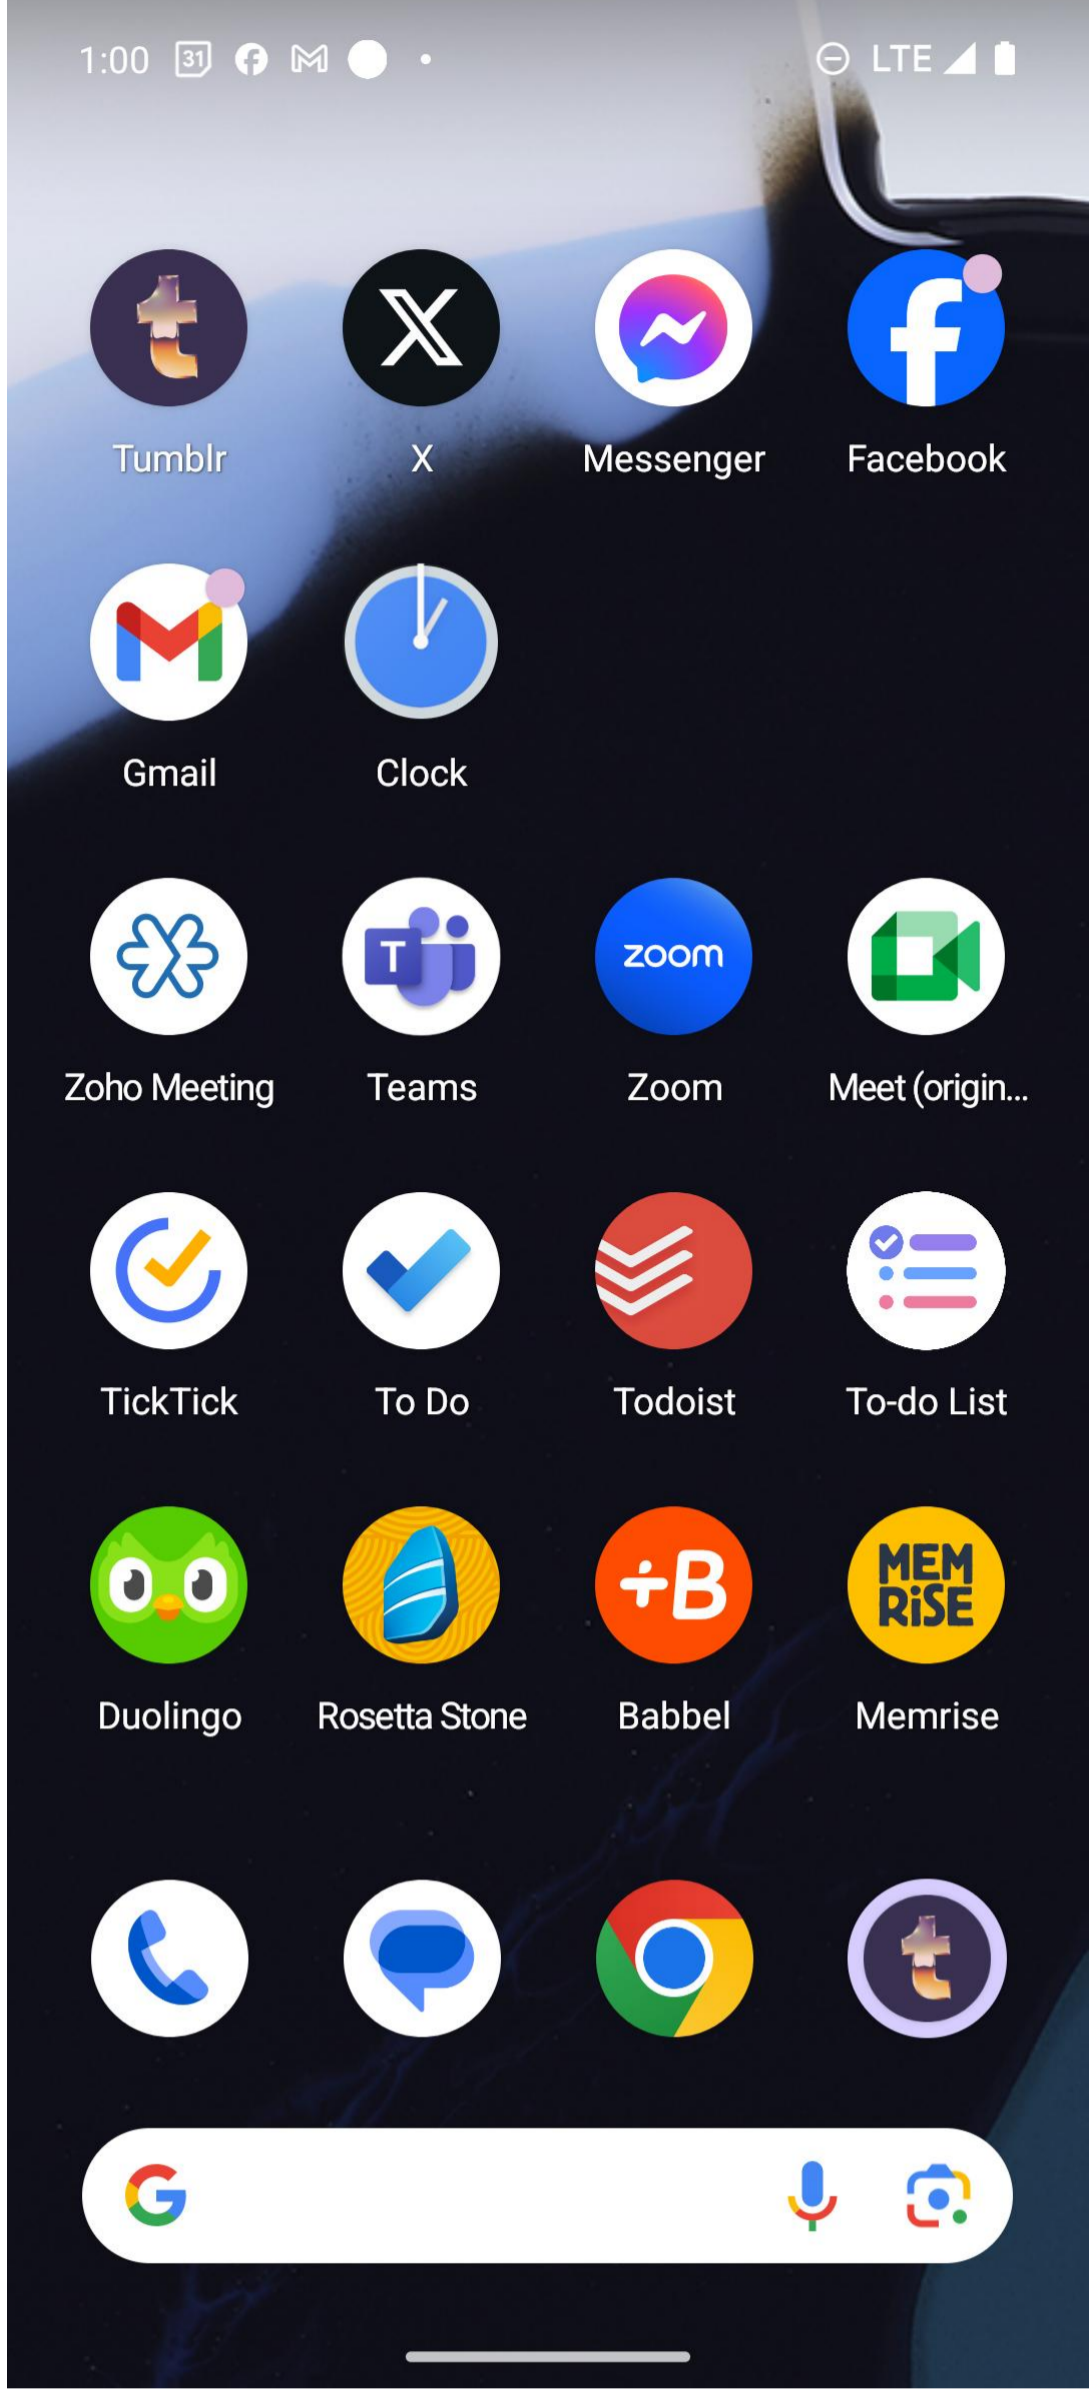

Step 20

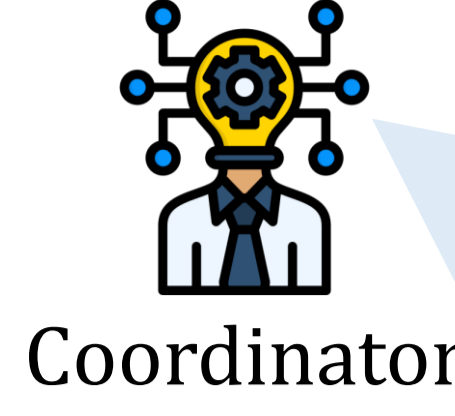

<think>I am selecting the Clock app to proceed with setting an alarm for the business meeting. This action is necessary to ensure I am reminded of the meeting time, completing the final step of organizing the meeting after sending the invitation.</think>  
<answer>Open the Clock app. </answer>

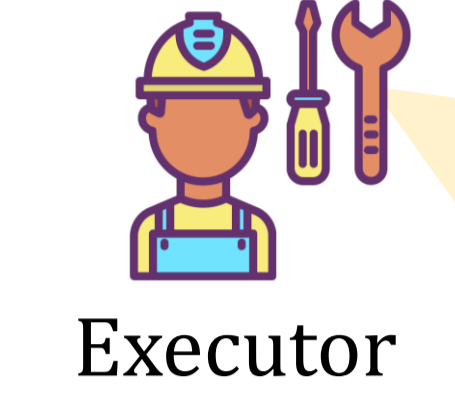

<think>The user wants to open the Clock app. The Clock app is visible on the screen, which is the appropriate app to use for setting an alarm. The next step is to open the Clock app to proceed with setting the alarm.</think>  
<answer>CLICK: (404, 663)</answer>

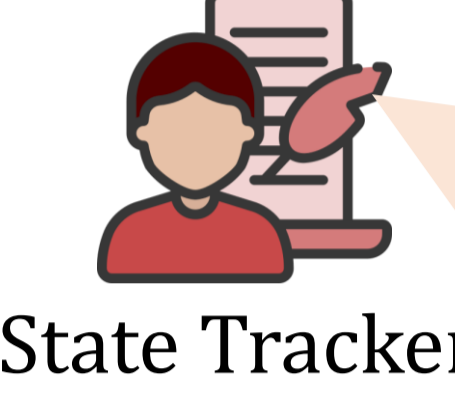

A business meeting with saltyfunssweets has been organized using the Zoom app, and the meeting details have been sent via direct message on Tumblr. The meeting has been scheduled, saved, and the necessary information has been communicated to the recipient, ensuring all participants have the required details for the meeting.

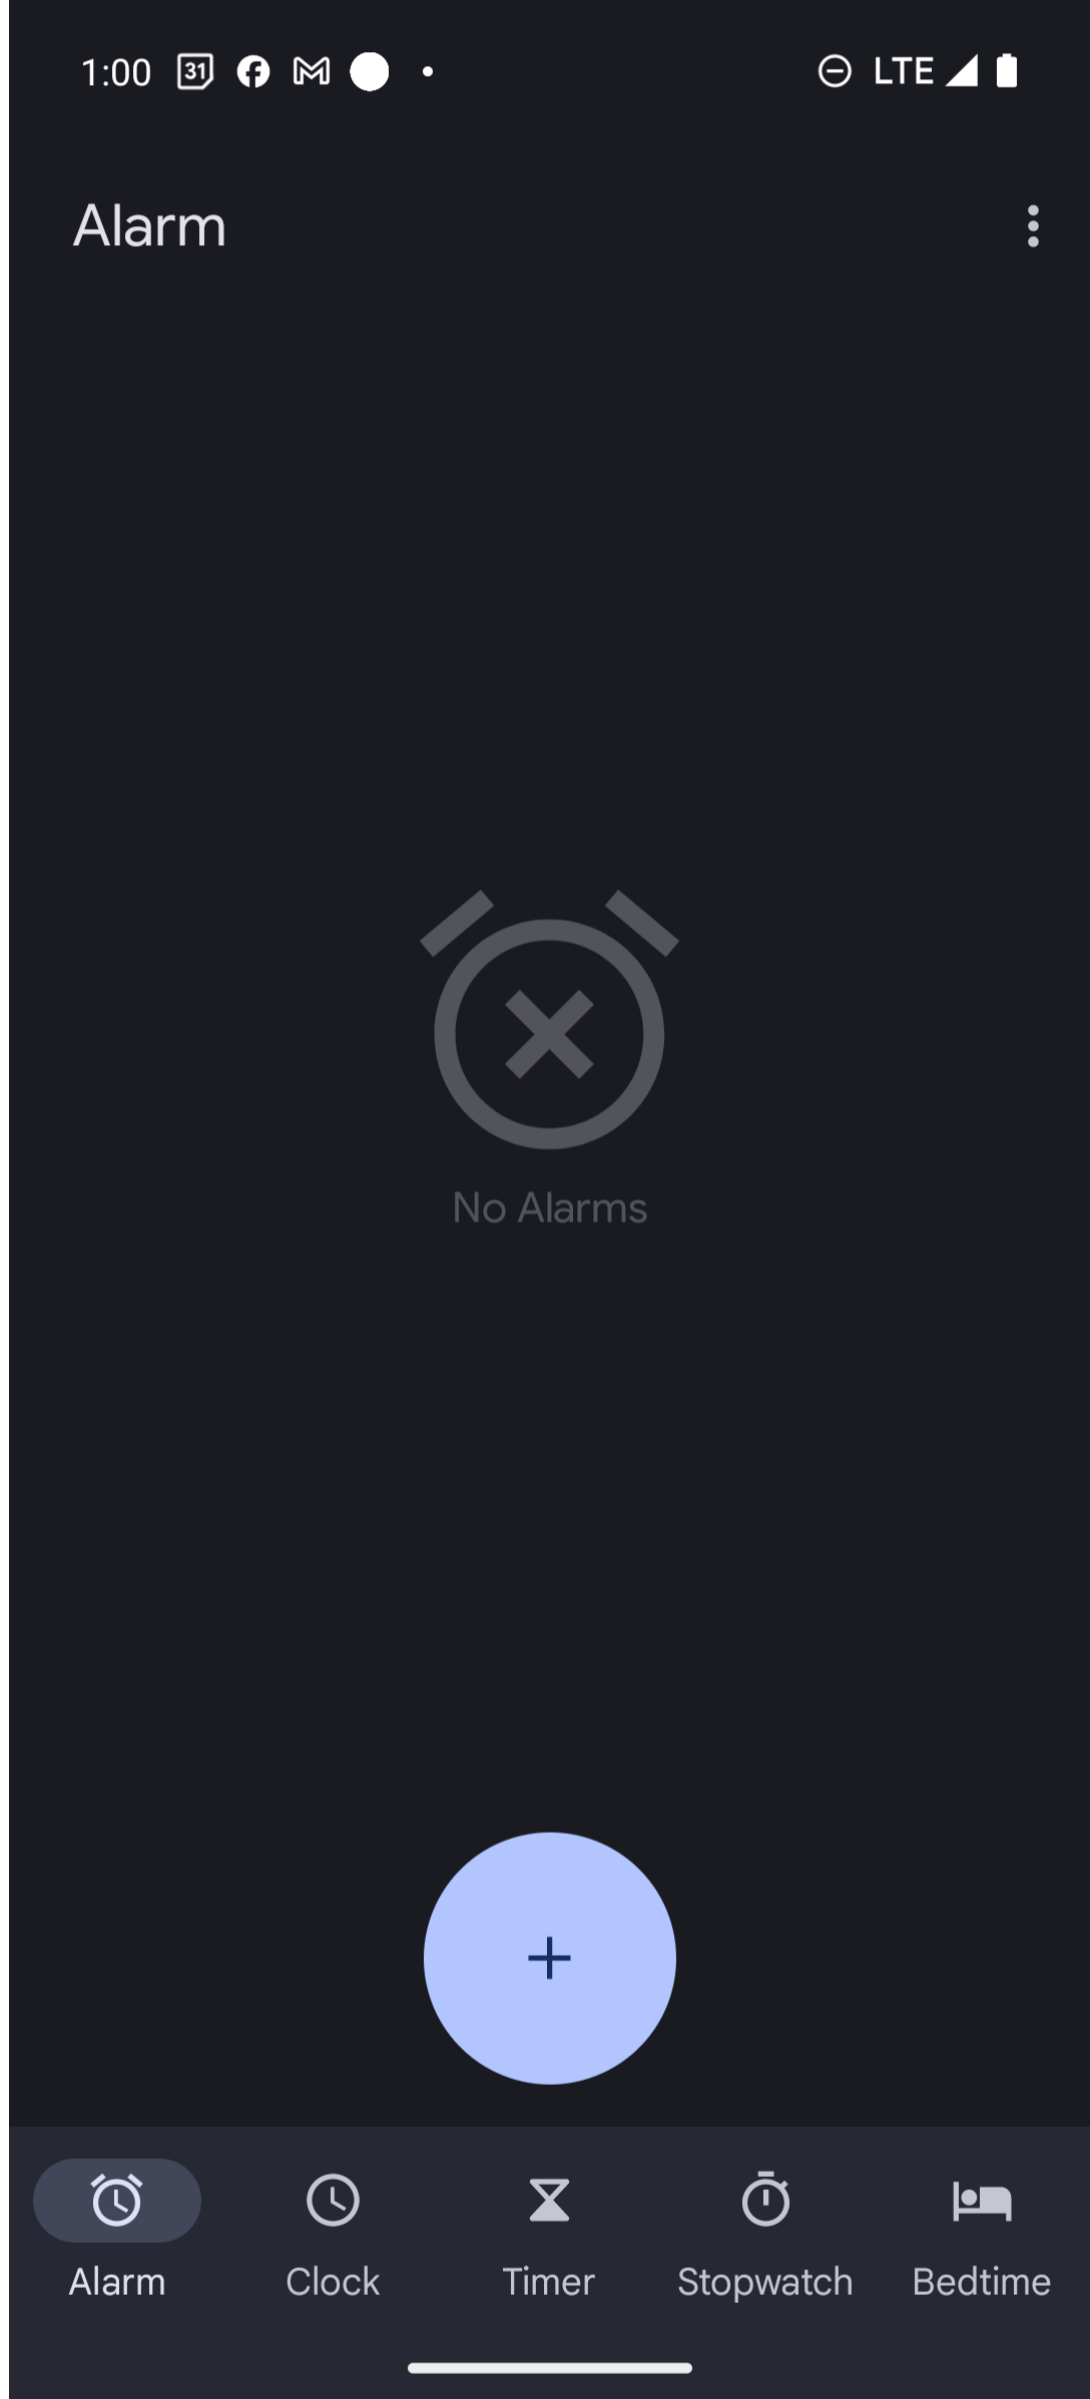

Step 21

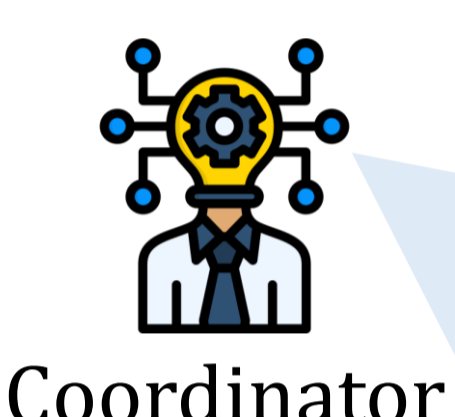

<think>This is a screenshot of the Alarm section in the Clock app on an Android phone. It shows no alarms set, with a prominent plus button to add a new alarm.I am choosing to tap the plus button to set a new alarm for the business meeting. This action is appropriate because I need to ensure I am reminded of the meeting time, and adding an alarm is the next logical step after sending the meeting invitation.</think>  
<answer>Tap the plus button to add a new alarm. </answer>

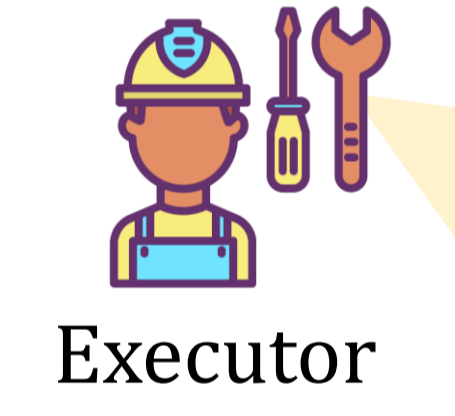

<think>The user wants to add a new alarm. The screen shows a large blue plus button in the center, which is typically used to add new items, such as alarms. This button is the most likely target for the user's instruction to add a new alarm.</think>  
<answer>CLICK: (532, 1963)</answer>

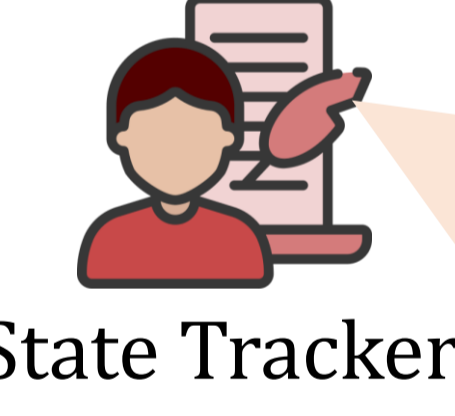

A business meeting with saltyfunssweets has been organized using the Zoom app, and the meeting details have been successfully sent via direct message on Tumblr. An alarm has also been set using the Clock app to ensure a reminder for the scheduled meeting time.

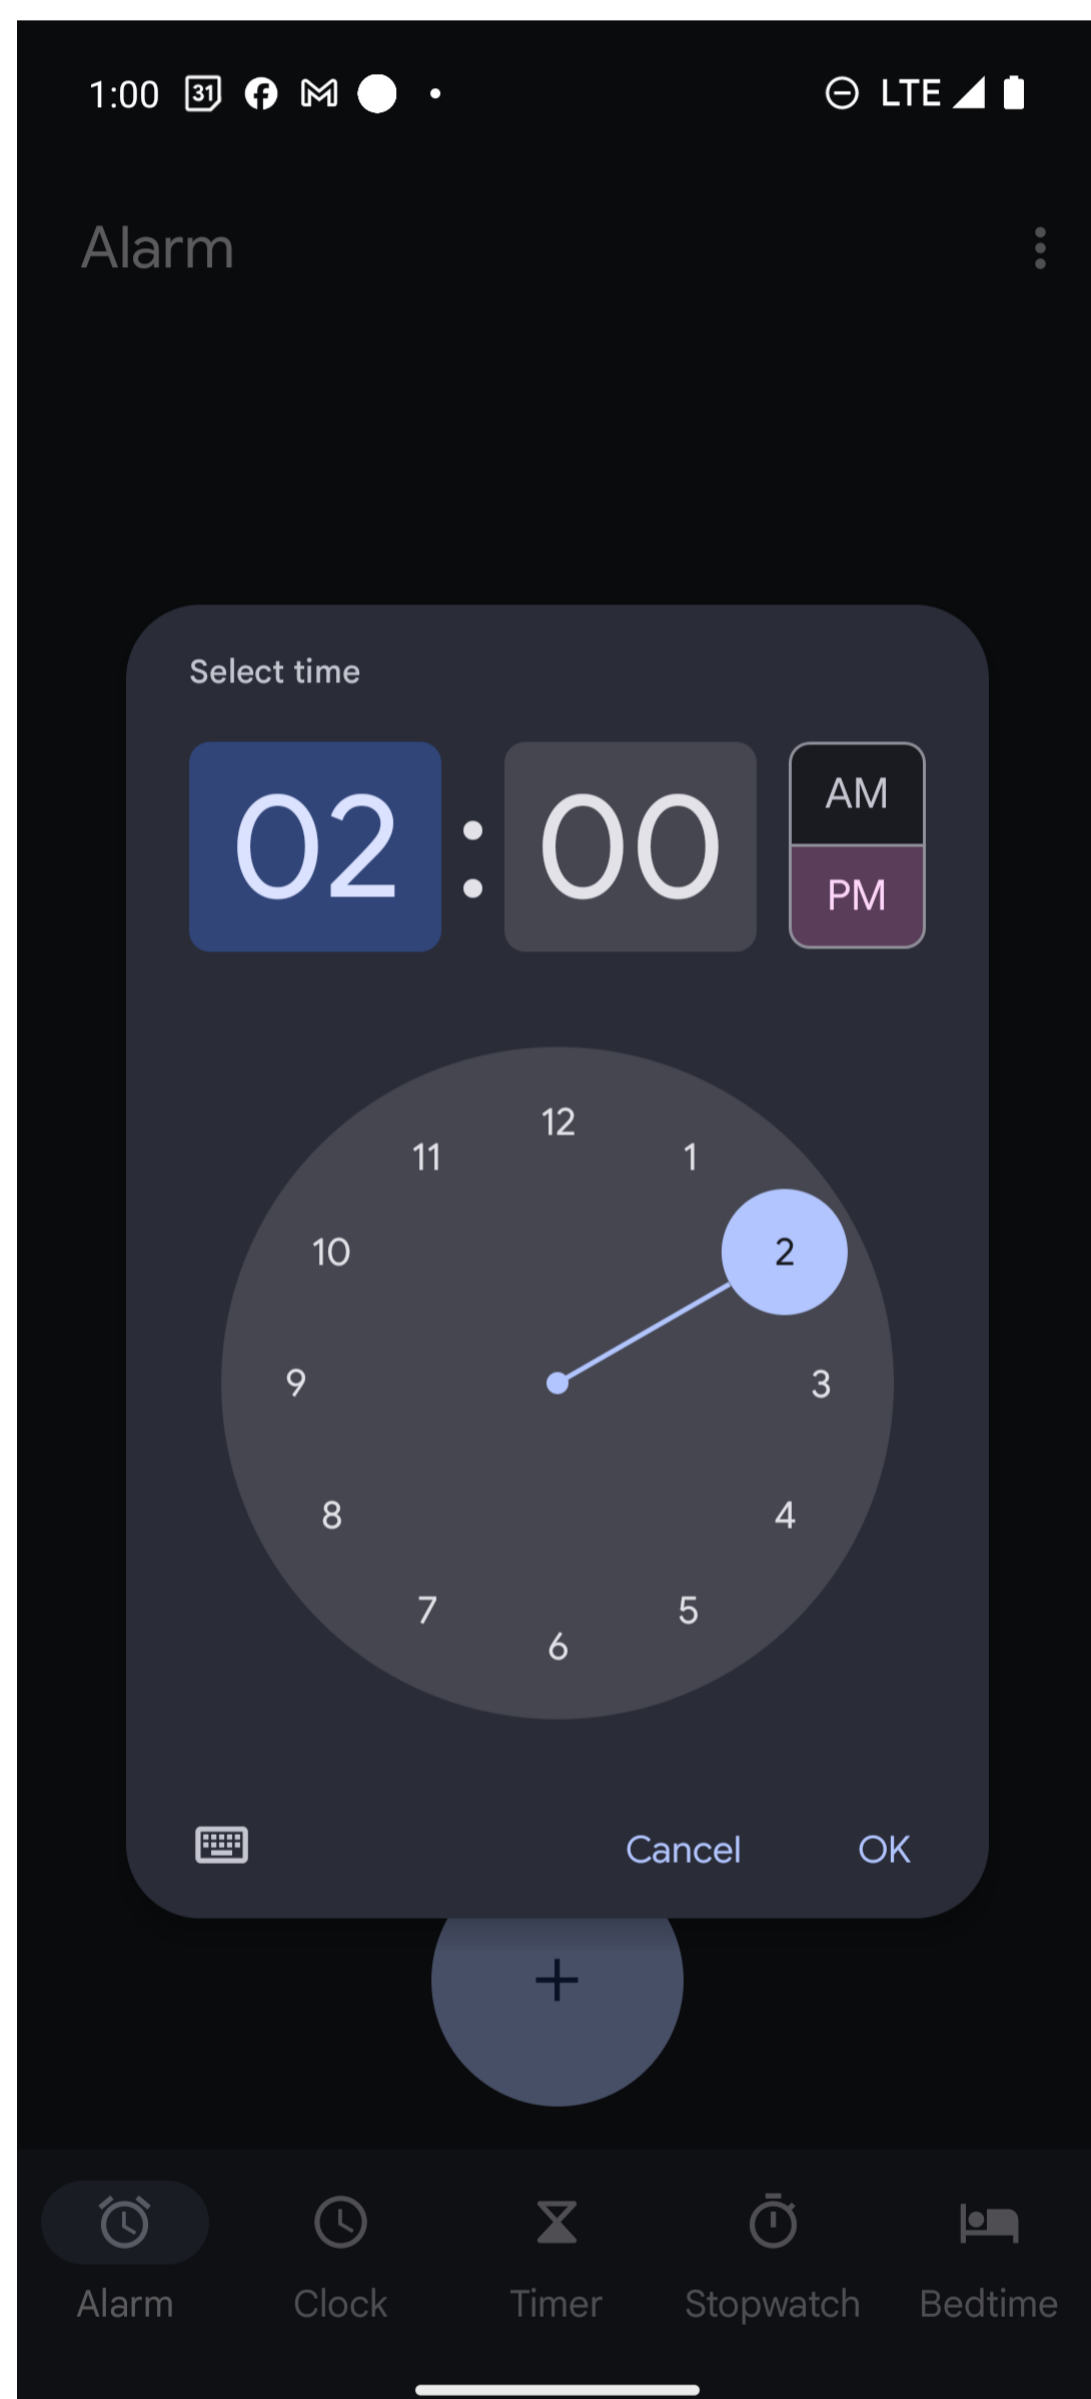

Step 22

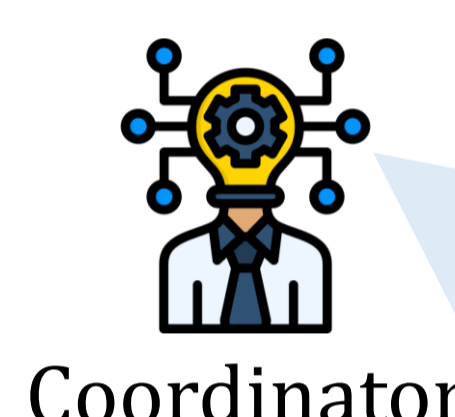

<think>This is a screenshot of the Clock app on an Android phone, displaying the time selection interface for setting an alarm. The user is in the process of setting the hour for the alarm, with the current selection being 2:00 PM.I am selecting the hour for the alarm to ensure it is set correctly for the business meeting. By choosing the appropriate hour, I can finalize the alarm setup, which is crucial for timely reminders.</think>  
<answer>Select the hour for the alarm.</answer>

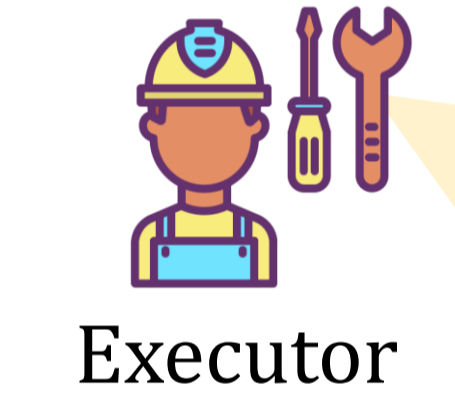

<think>The user wants to set the hour for the alarm. The current time is set to 02:00, and the user needs to change the hour. The clock interface allows for selecting the hour by tapping on the corresponding number on the clock face. The current hour is 2, and the user might want to change it to a different hour. </think>  
<answer>CLICK: (318, 1498)</answer>

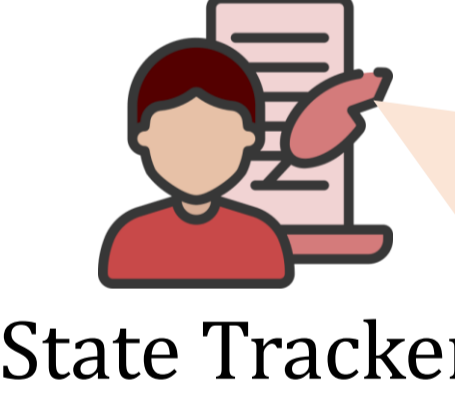

A business meeting has been successfully scheduled using the Zoom app, and the details have been shared with saltyfunssweets via direct message on Tumblr. An alarm has been set using the Clock app to ensure a timely reminder for the meeting.

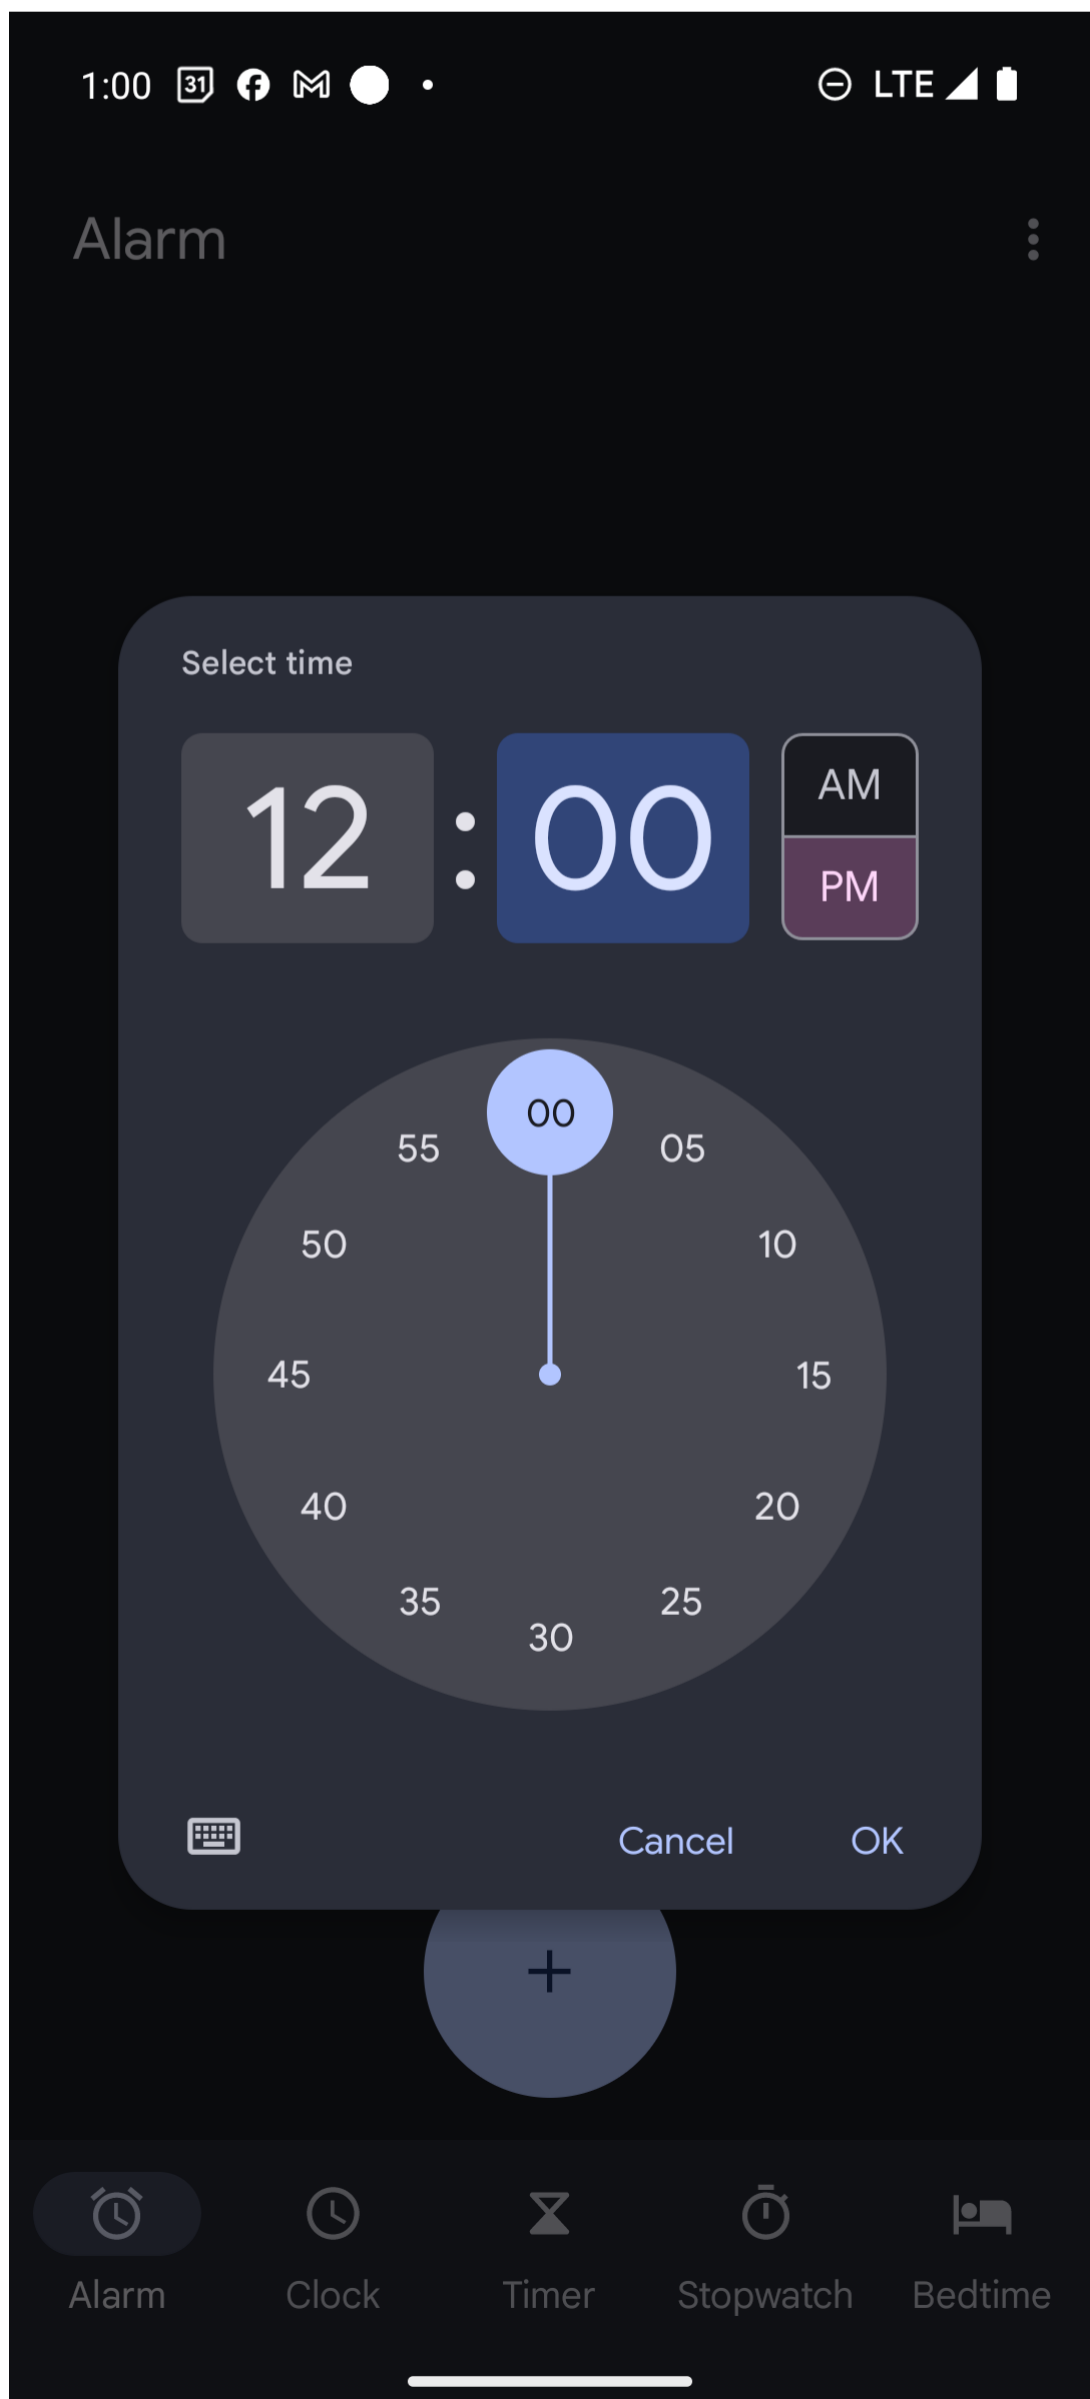

Step 23

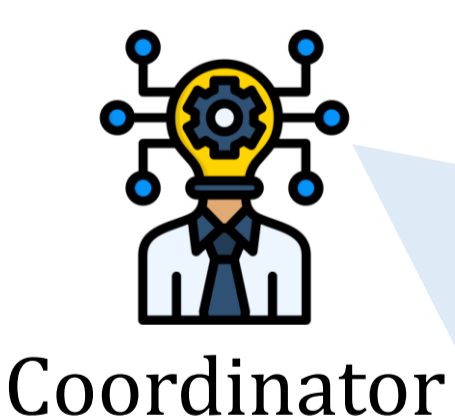

<think>This is a screenshot of the Clock app on an Android phone, displaying the time selection interface for setting an alarm. The user is adjusting the minute hand to set the alarm time. I am scrolling to adjust the minute hand on the clock interface to set the correct time for the alarm.</think>  
<answer>Adjust the minute hand on the clock interface.</answer>

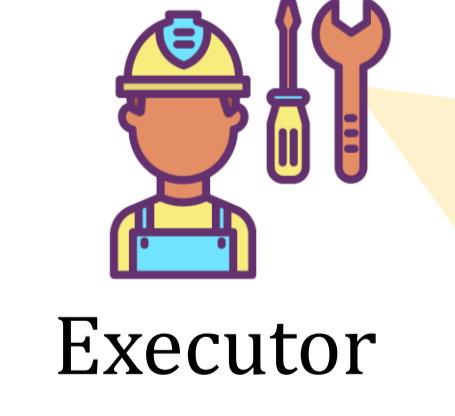

<think>The user wants to adjust the minute hand on the clock interface. The current screen shows a circular dial with numbers representing minutes, and the minute hand is currently at 00. To adjust the minute hand, the user needs to interact with the circular dial. The numbers on the dial represent the minutes, and the user can click on the desired minute to set it.</think>  
<answer>CLICK: (550, 1625)</answer>

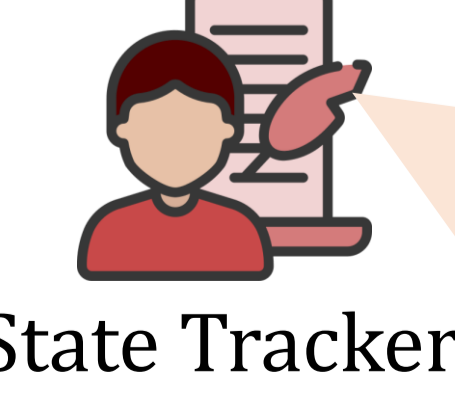

A business meeting with saltyfunssweets has been organized using the Zoom app, and the meeting details have been successfully sent via direct message on Tumblr. An alarm has been set using the Clock app to ensure a timely reminder for the scheduled meeting.

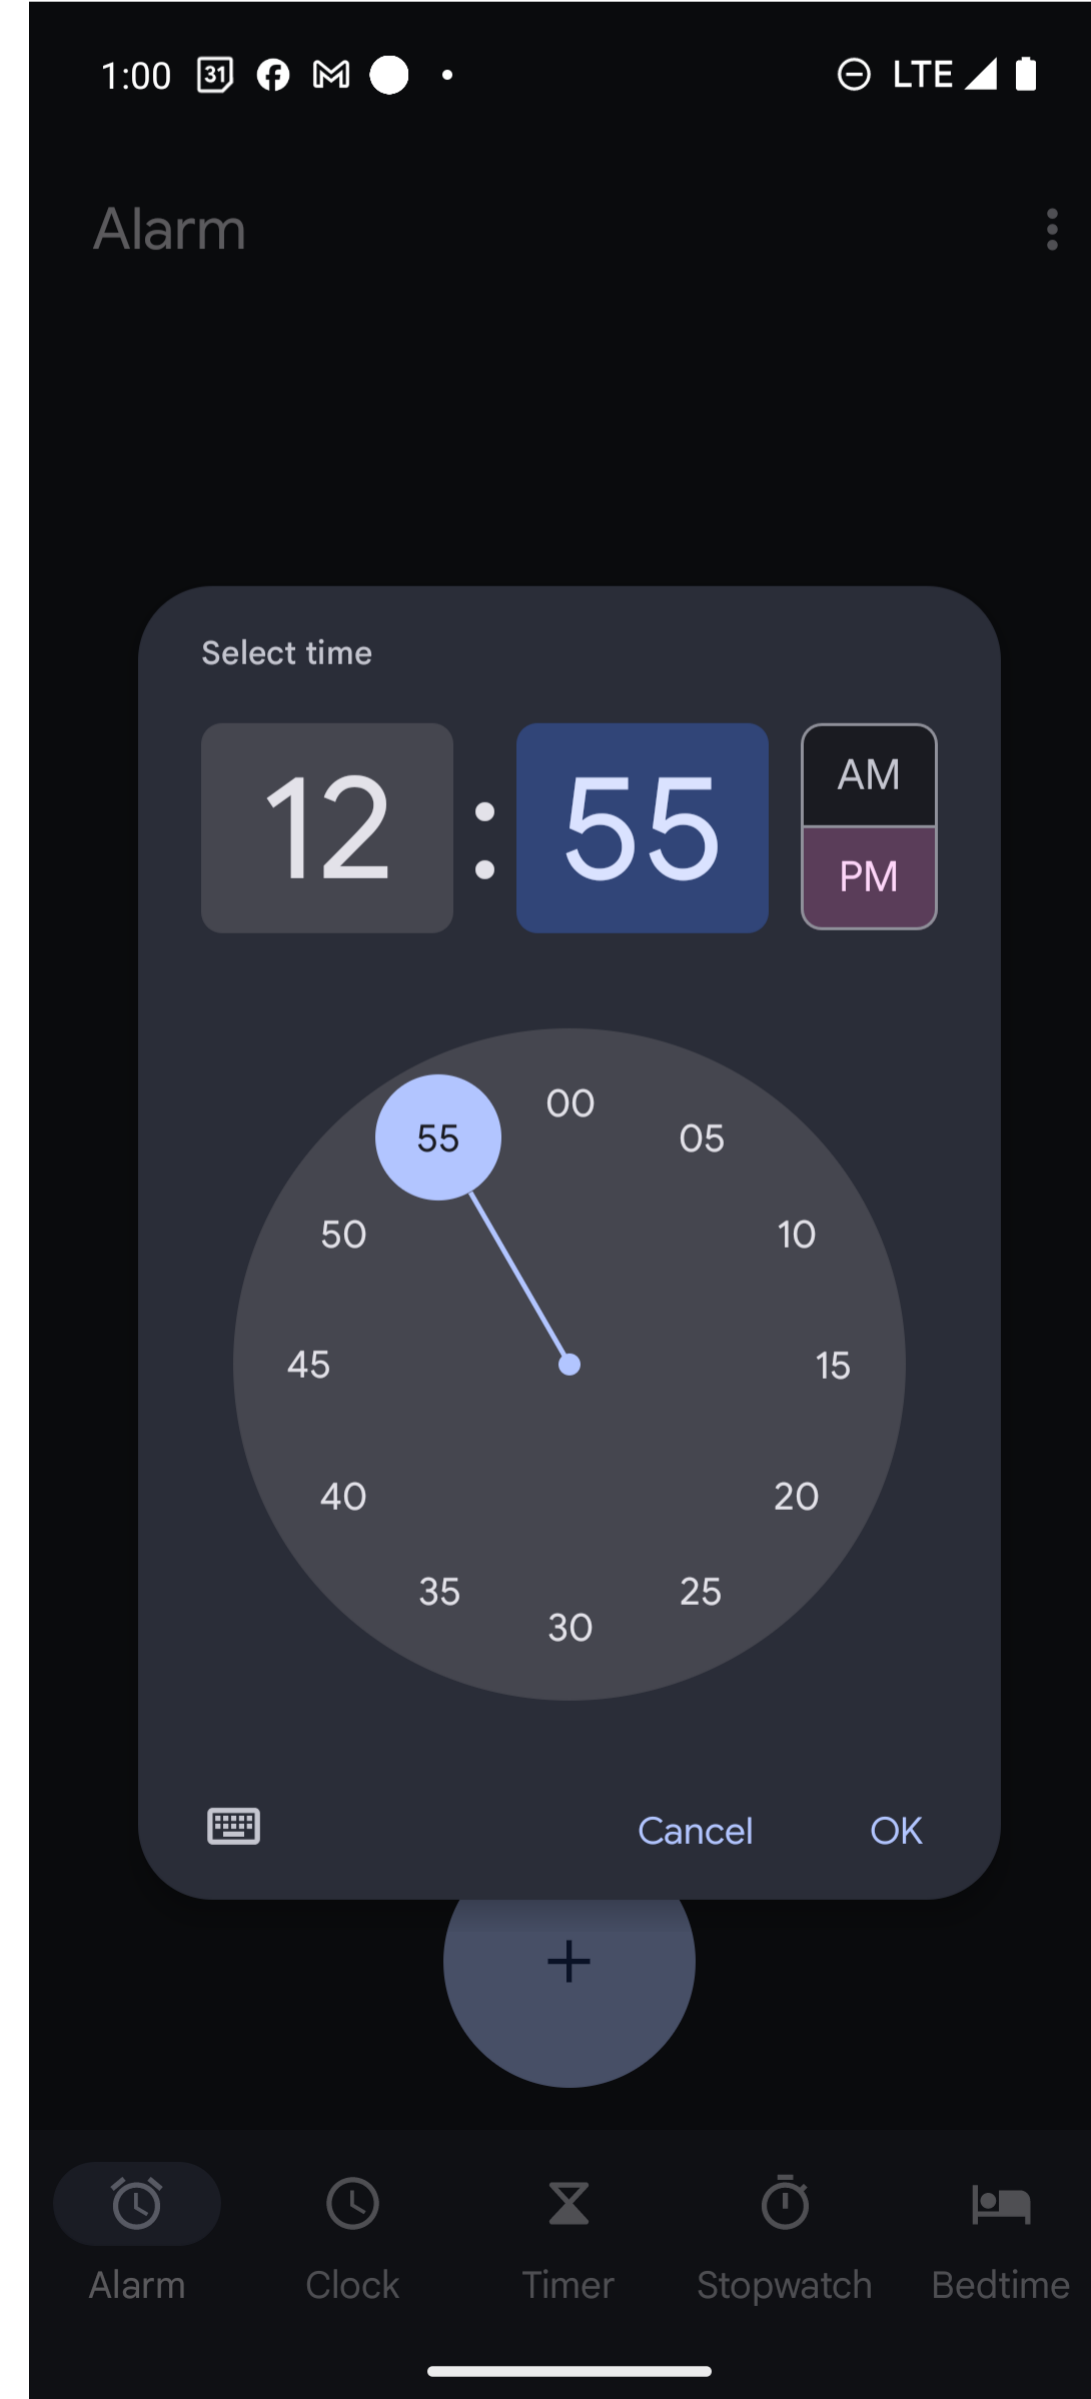

Step 24

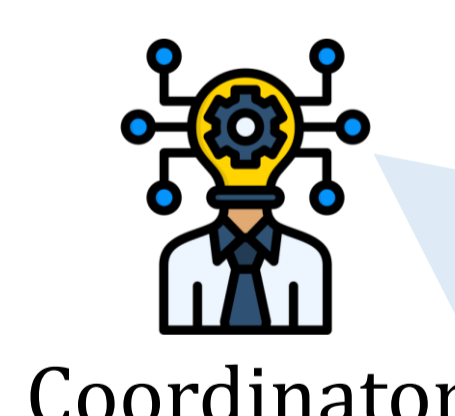

<think>This is a screenshot of the Clock app on an Android phone, showing the time selection interface for setting an alarm. The user is adjusting the minute hand to 55, with the time set to 12:55 PM.I am confirming the time setting for the alarm by clicking 'OK'. This action finalizes the alarm setup, ensuring it is set for the correct time, which is crucial for timely reminders for the business meeting.</think>  
<answer>Confirm the selected alarm time.</answer>

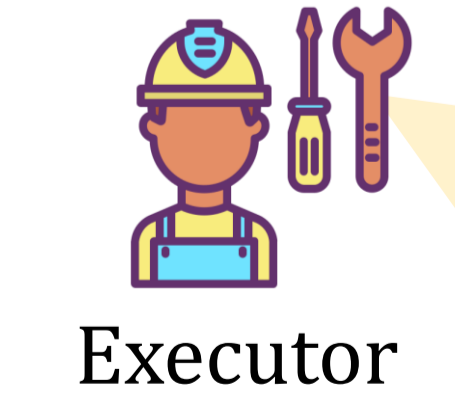

<think>The user wants to confirm the selected alarm time. The current screen shows a time picker with the time set to 12:55 PM. The 'OK' button at the bottom right of the time picker is likely the confirmation button for the selected time. Clicking this button will confirm the selected time and proceed with setting the alarm.</think>  
<answer>CLICK: (873, 1833)</answer>

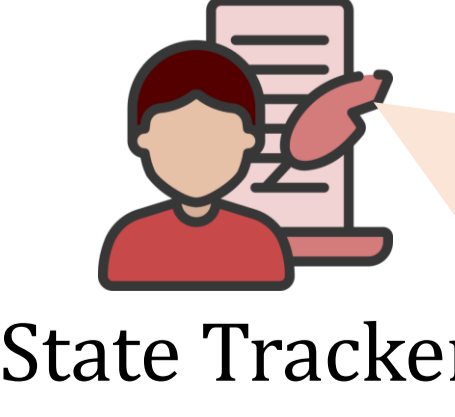

A business meeting with saltyfunssweets has been successfully organized using the Zoom app. The meeting details were sent via direct message on Tumblr, ensuring the recipient received the necessary information. An alarm was set in the Clock app to provide a timely reminder for the meeting.

User Instruction

Organize a business meeting with saltyfunsweets using ZOOM Cloud Meetings, send out the meeting invitations via Tumblr, and set an alarm clock for the meeting time using the Clock app.

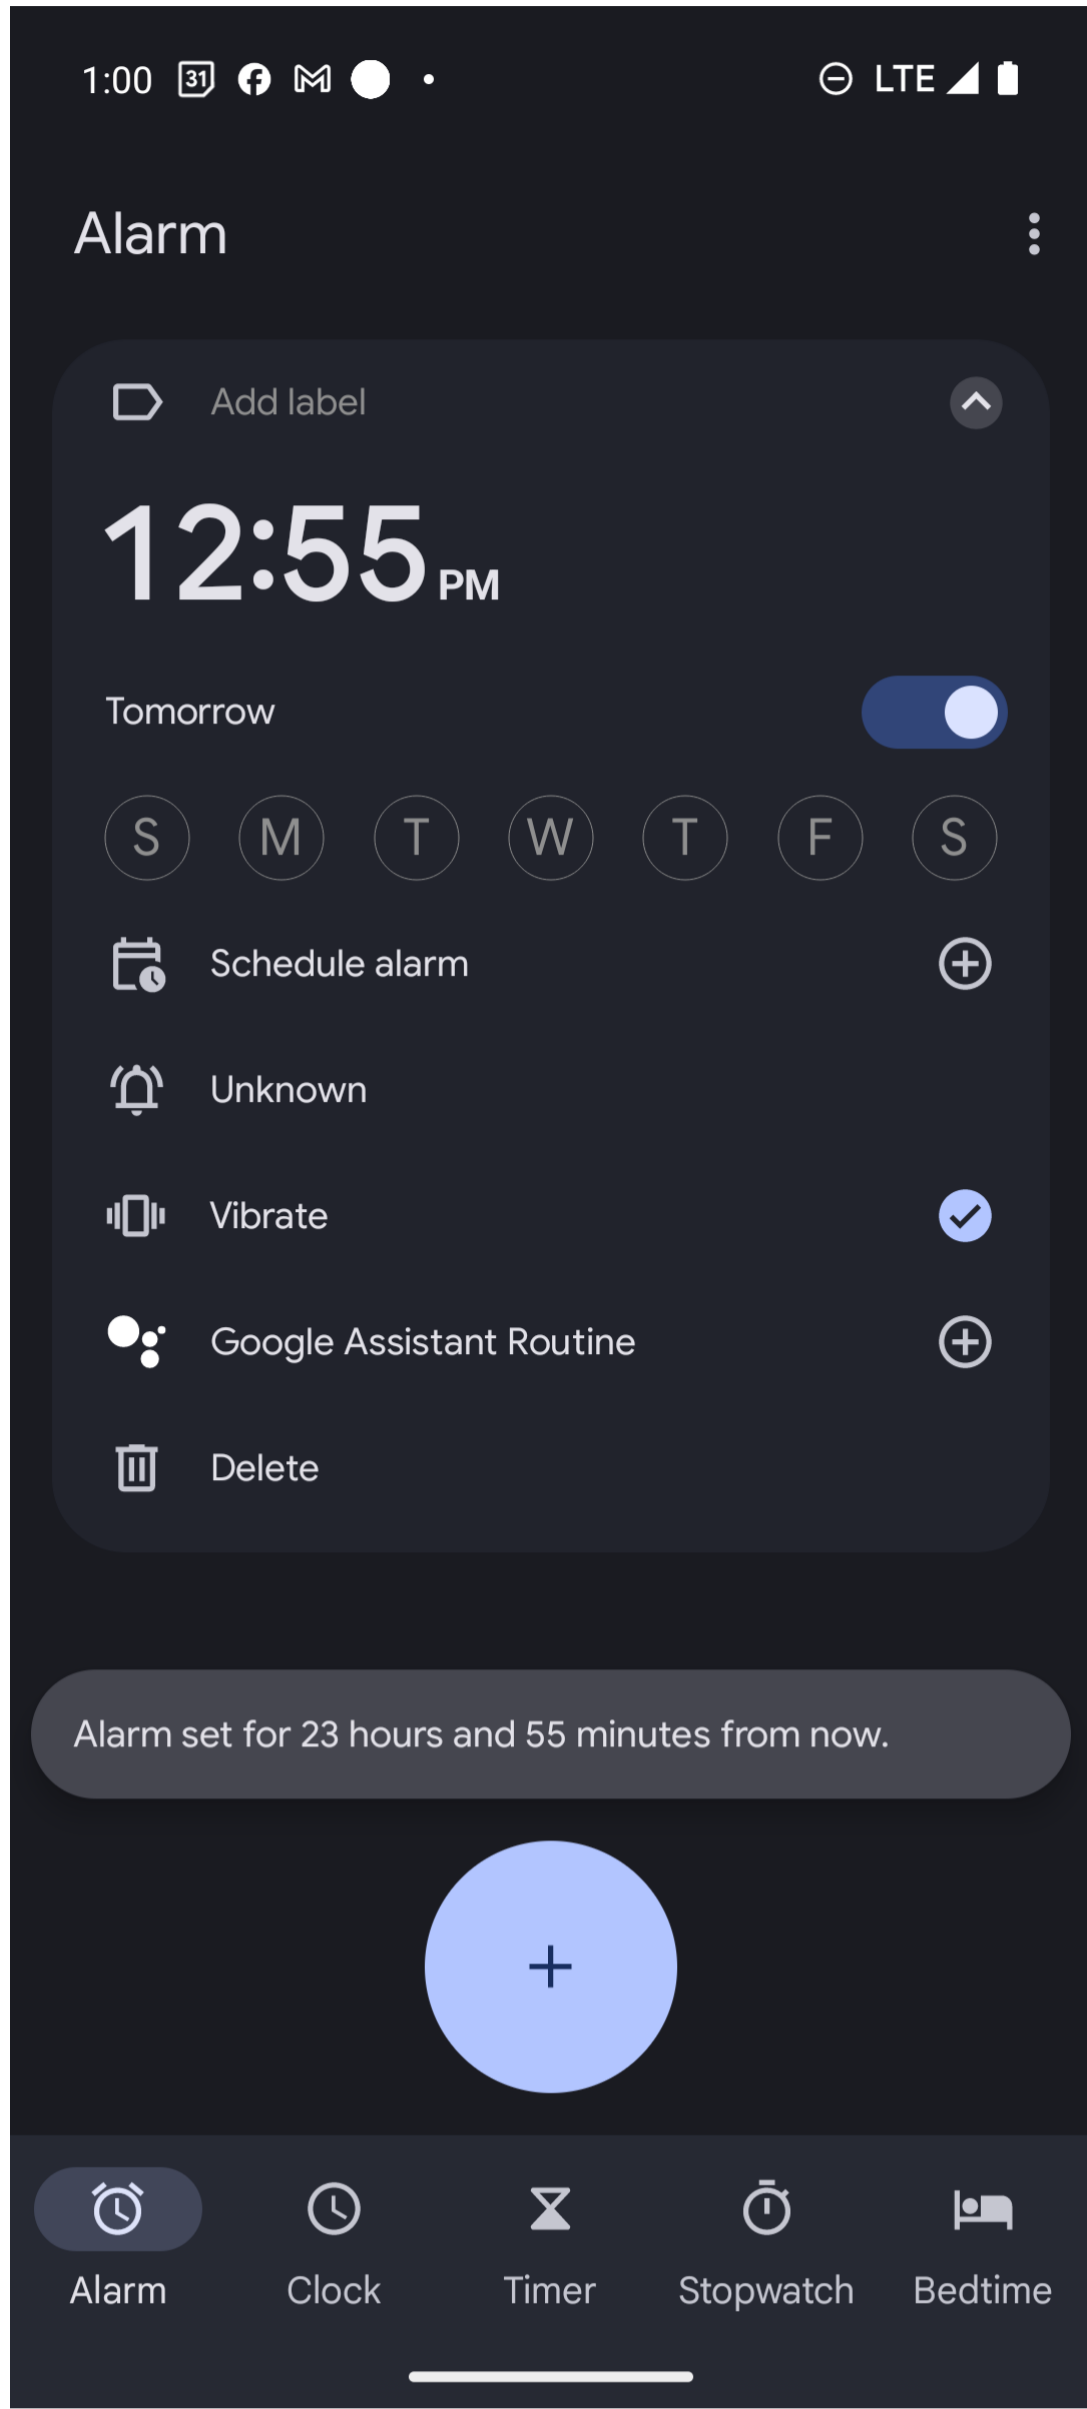

Step 25

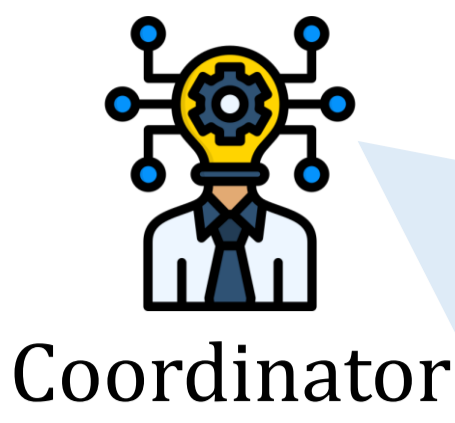

<think>This is a screenshot of the Clock app displaying an alarm set for 12:55 PM with options to schedule, vibrate, and set a Google Assistant Routine. The alarm is set for tomorrow, and the user is in the process of confirming the alarm settings.I am confirming the alarm settings to ensure that the alarm is correctly configured for the business meeting. By clicking 'OK', I finalize the alarm setup, which is necessary to ensure I am reminded of the meeting at the specified time.</think>  
<answer>Confirm the alarm settings.</answer>

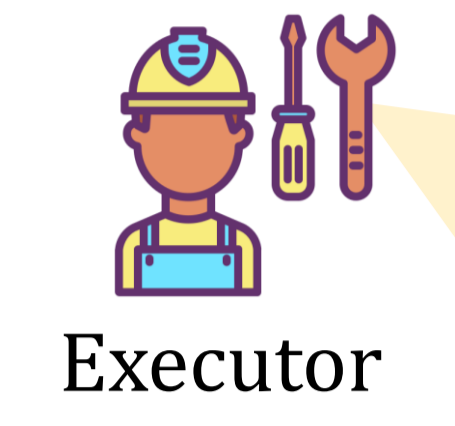

<think>The user wants to confirm the alarm settings. The current screen shows the alarm details, including the time, date, and various settings. The three-dot menu at the top right might provide an option to confirm or save the settings.</think>  
<answer>CLICK: (1036, 226)</answer>

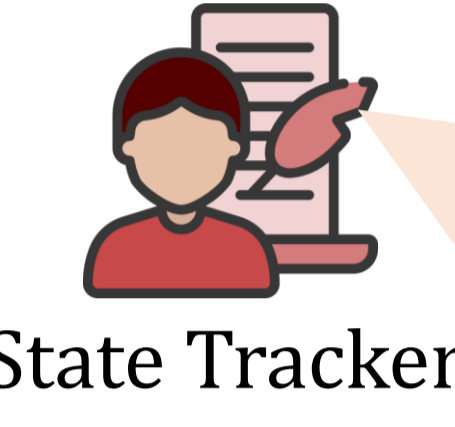

A business meeting with saltyfunsweets has been successfully organized using the Zoom app, and the meeting details have been sent out via direct message on Tumblr. An alarm has been set using the Clock app to ensure a timely reminder for the meeting, with a label added to distinguish it from other alarms.

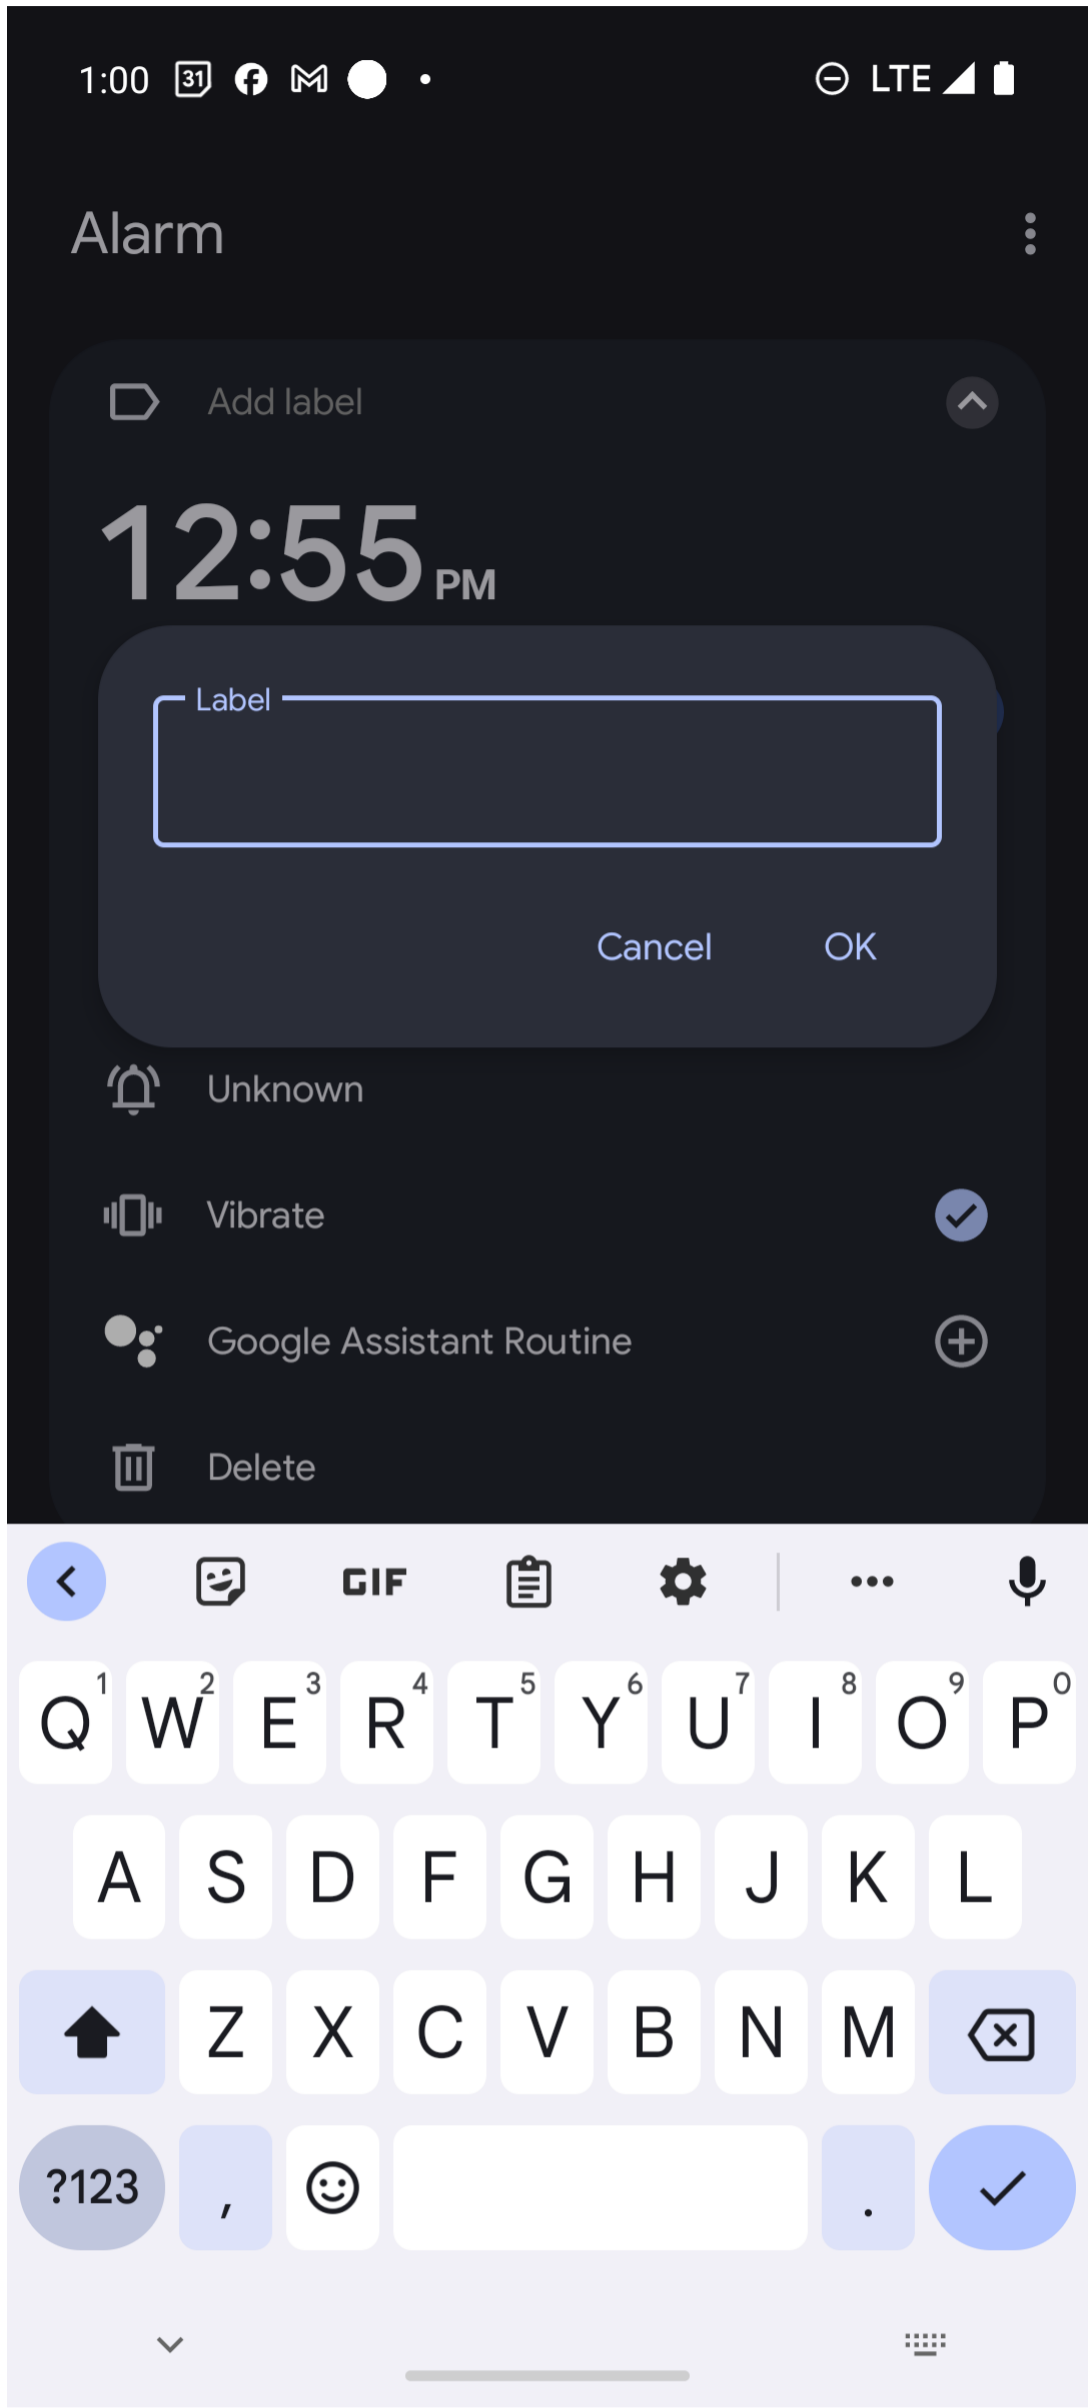

Step 26

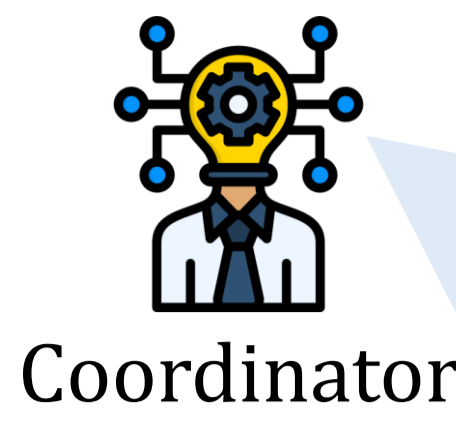

<think>This is a screenshot of the alarm settings on an Android phone, showing a time set for 12:55 PM with options to add a label and confirm the time. The keyboard is visible, indicating that the user is in the process of labeling the alarm.I am labeling the alarm to ensure it is clearly identified as related to the business meeting with saltyfunsweets. This helps in quickly recognizing the purpose of the alarm when it goes off, ensuring I am prepared for the meeting.</think>  
<answer>Label the alarm with 'Meeting'.</answer>

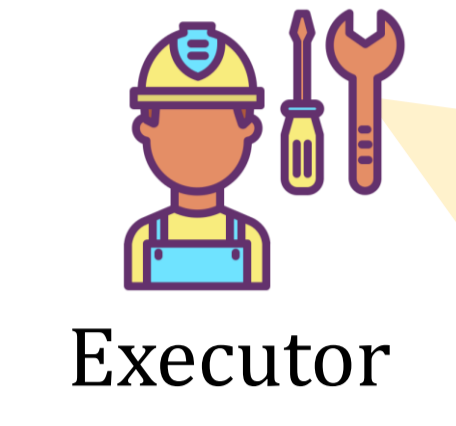

<think>The user wants to label the alarm with 'Meeting'. The 'Label' field is currently empty, and the keyboard is active, indicating that the user can type a label. The next step is to input the desired label into the 'Label' field.</think>  
<answer>TYPE: 'Meeting'</answer>

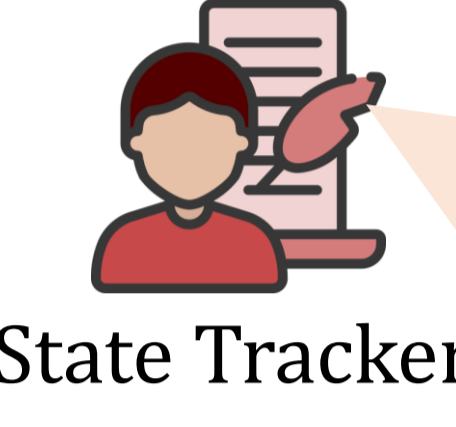

A business meeting with saltyfunsweets has been successfully organized using the Zoom app, and the meeting details have been sent via direct message on Tumblr. An alarm has been set in the Clock app with a specific label to remind of the scheduled meeting, ensuring all necessary preparations are complete.

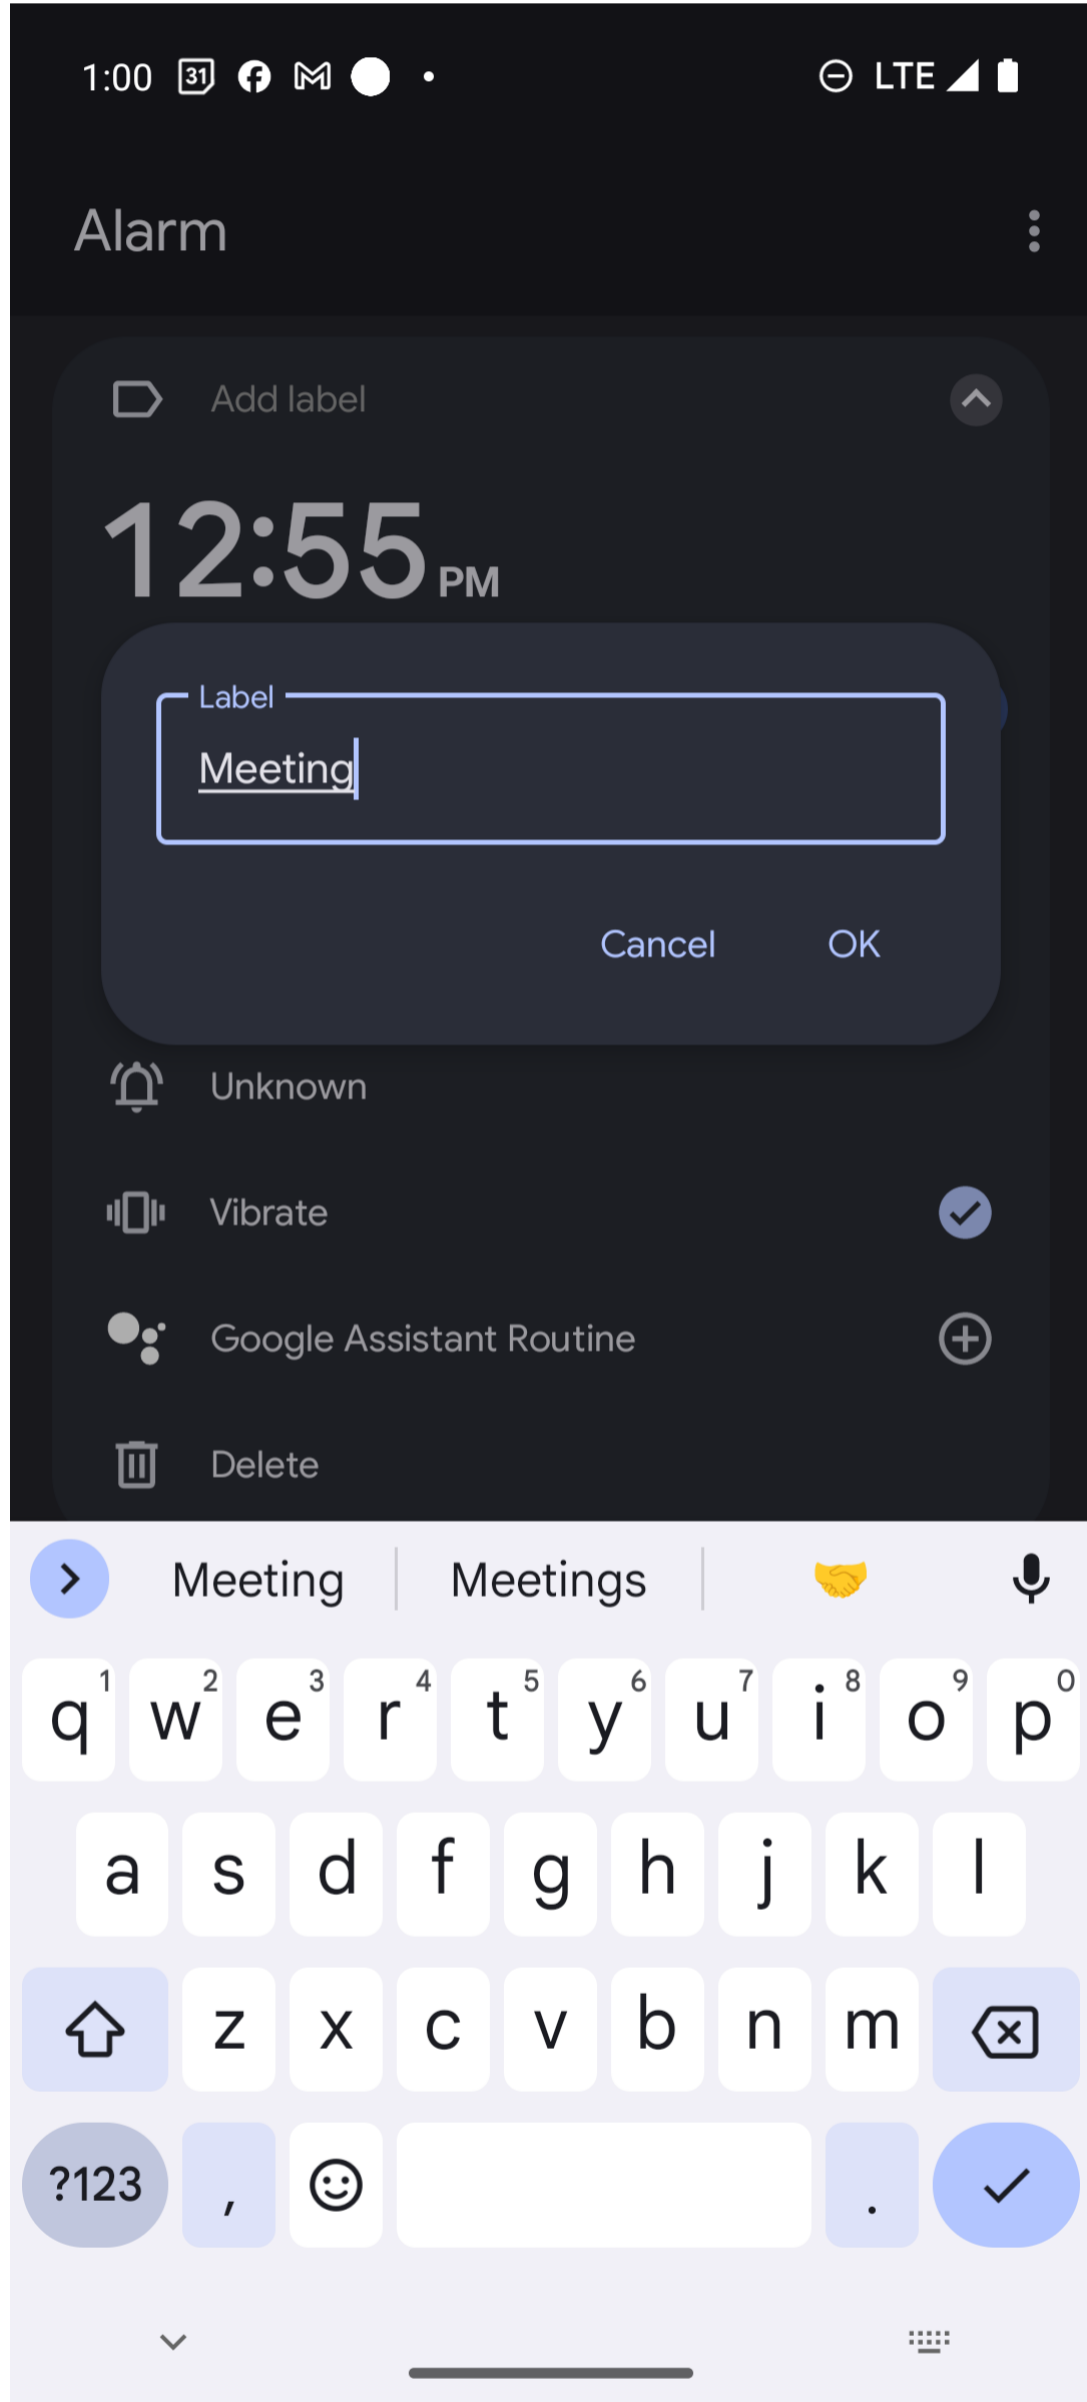

Step 27

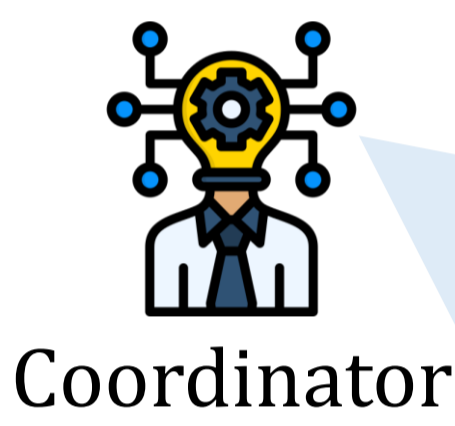

<think>I am confirming the label for the alarm to ensure it is correctly set for the business meeting. By clicking 'OK', I finalize the label, which helps me easily identify the alarm's purpose and ensures I am reminded of the meeting at the right time. This step is crucial to complete the task of setting up the alarm for the meeting.</think>  
<answer>Confirm the alarm label.</answer>

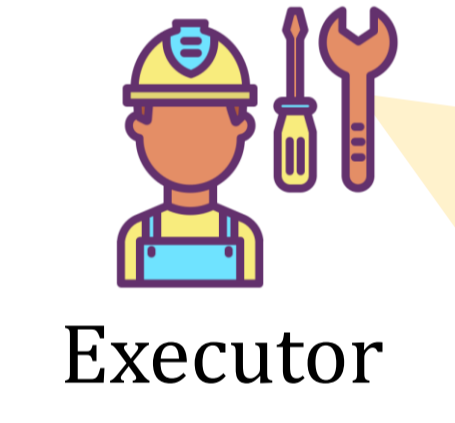

<think>The user has already entered the label 'Meeting' for the alarm. The next step is to confirm this label by clicking the 'OK' button to finalize the alarm setup. This will ensure the alarm is correctly labeled and set for the business meeting.</think>  
<answer>CLICK: (850, 943)</answer>

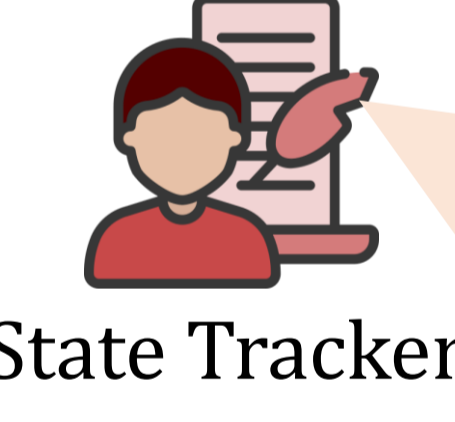

A business meeting with saltyfunsweets has been successfully organized using the Zoom app, and the meeting details have been sent via direct message on Tumblr. An alarm has been set in the Clock app with a specific label to remind of the scheduled meeting, ensuring all necessary preparations are complete.

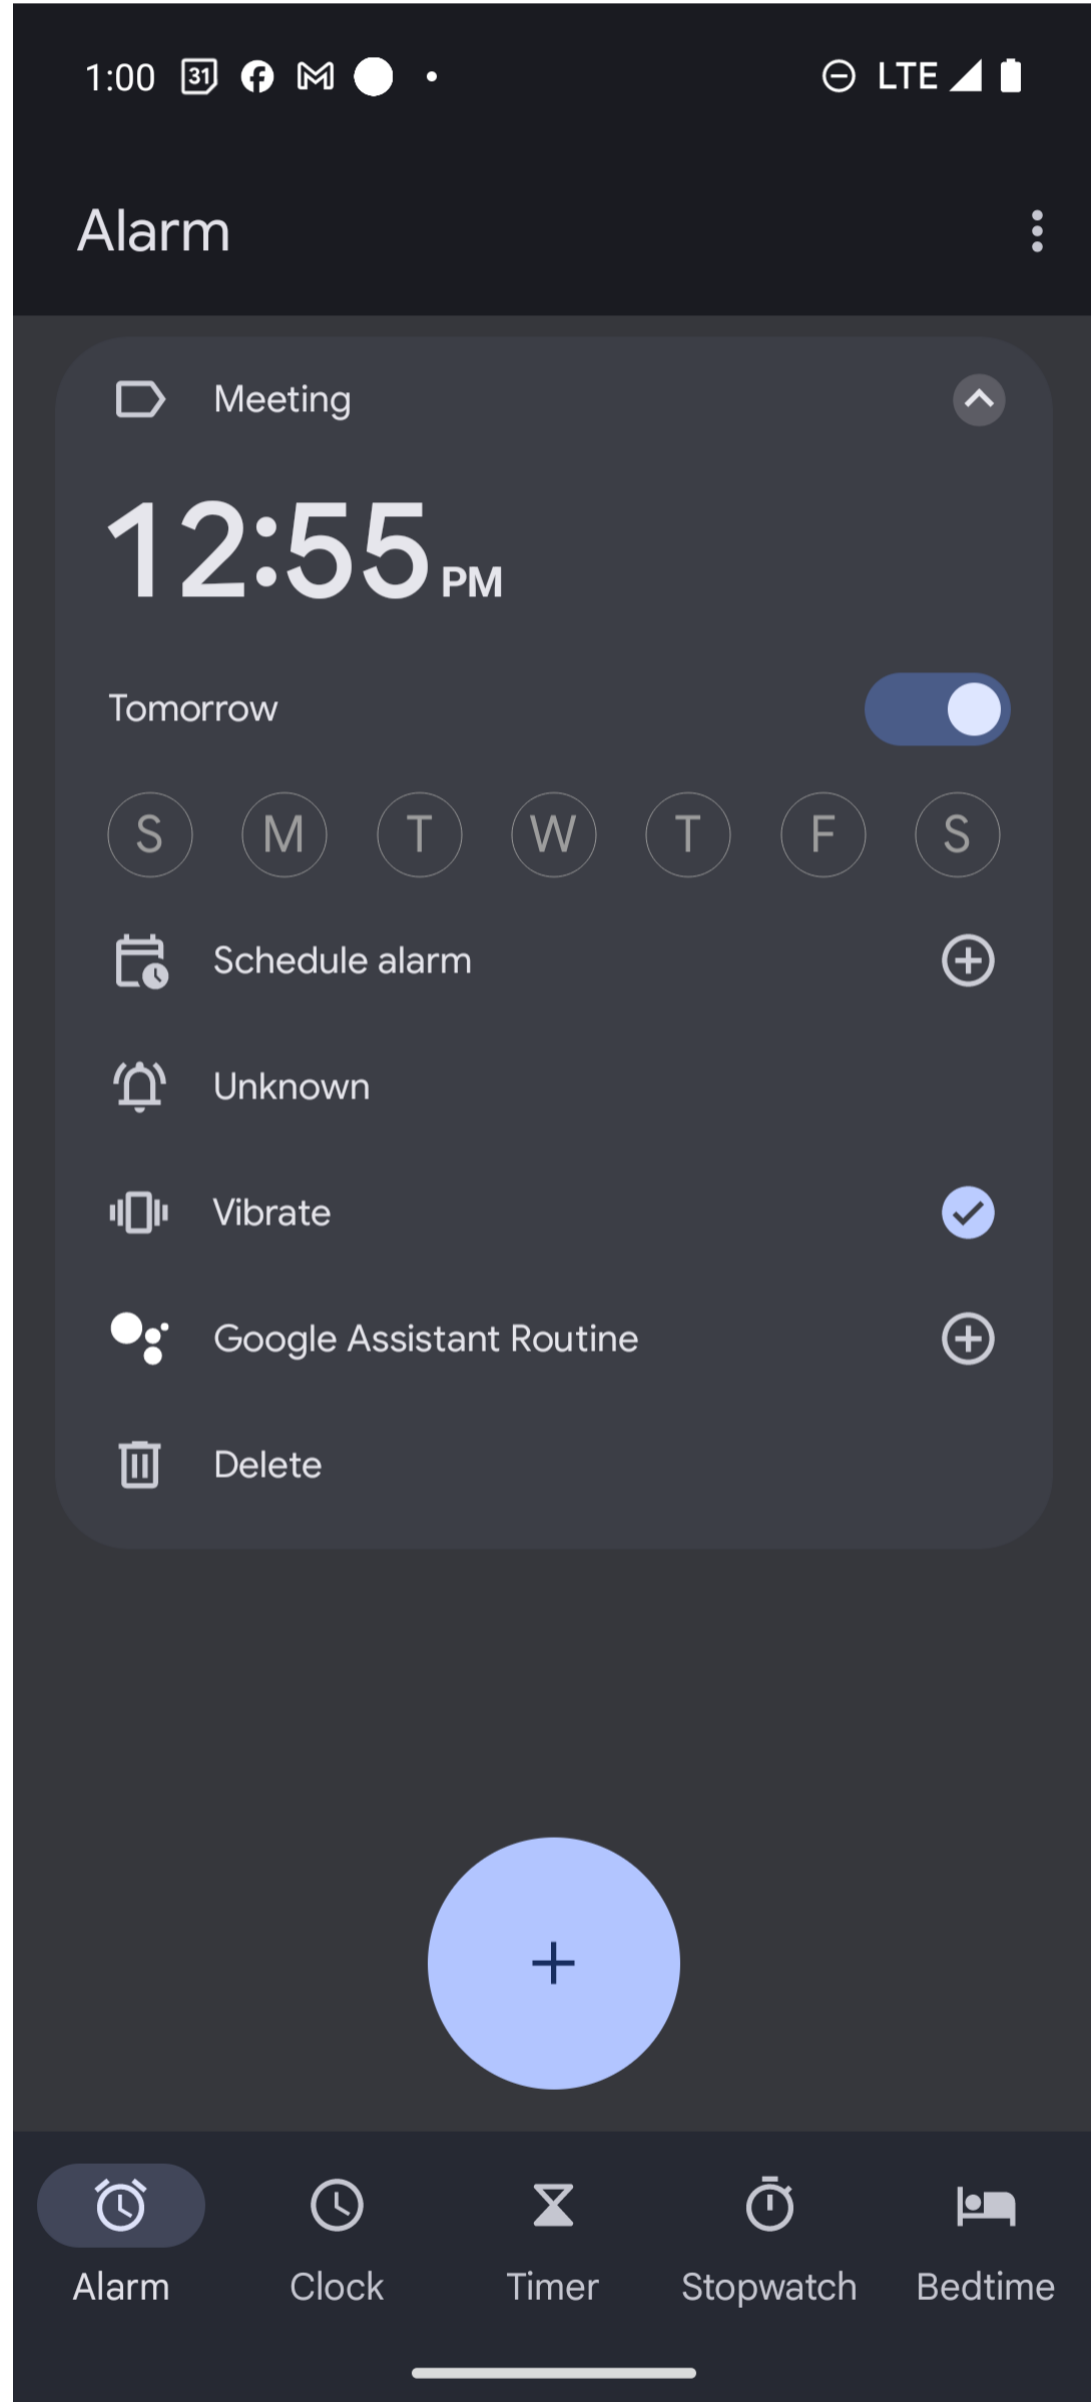

Step 28

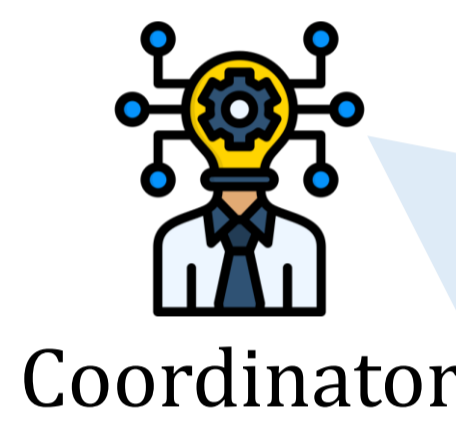

<think>This is a screenshot of the alarm settings on an Android phone, showing an alarm labeled 'Meeting' set for 12:55 PM. The alarm is scheduled for tomorrow with options to vibrate and set a Google Assistant Routine.I am confirming the alarm label 'Meeting' to ensure it is correctly set for the business meeting. This action finalizes the alarm setup, allowing me to proceed with organizing the meeting and sending out invitations.</think>  
<answer>Confirm the alarm.</answer>

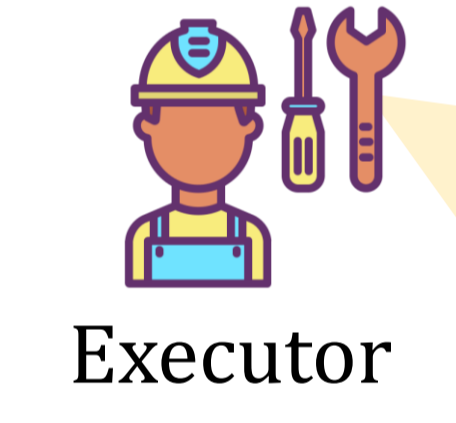

<think>The user wants to confirm the alarm label 'Meeting'. I am setting an alarm to ensure I am reminded of the scheduled business meeting. The action of confirming the alarm setup is crucial to guarantee that I receive a timely notification, ensuring all preparations are complete for the meeting.</think>  
<answer>COMPLETE</answer>

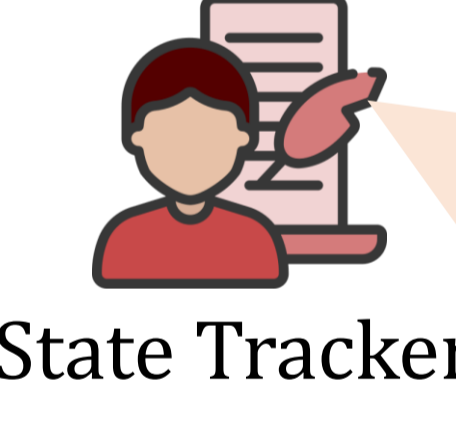

A business meeting with saltyfunsweets has been organized using the Zoom app, with invitations sent out via Tumblr. An alarm has been set in the Clock app to ensure a timely reminder for the meeting, complete with a label for easy identification.
